# Supplementary material for: Differential invariants of Einstein-Weyl structures in 3D
Source: arXiv:1802.00702 ancillary file (2018-02-02)
Supplement: Supplementary file 1 [file EWCalculations.pdf]

# Differential invariants of Einstein-Weyl structures

This Maple-worksheet contains many of the computations done for the paper "Differential invariants of Einstein-Weyl structures" and it is structured in the same way as the paper. It is made with Maple 2016.2 and the version of the DifferentialGeometry package that comes with it.

All sections are supposed to work more or less independently of each other, except for the first one on which every other section depends.

>

## Define PDE and symmetries (must be executed before all other sections)

```
> restart :
with(DifferentialGeometry) :
with(LieAlgebras) :
with(Tensor) :
with(Library) :
with(JetCalculus) :
with(Tools) :
with(ArrayTools) :
with(LinearAlgebra) :
with(RandomTools) :
with(PolynomialIdeals) :
with(PDETools) :
Preferences("ShowFramePrompt", false) :
DGsetup([t, x, y], [u, v], MM, 2) :
```

We define the PDE, and corresponding transformations (inclusions in  $J^k$ ).

```
> E1 := TotalDiff(u[_] * u[3] + u[2] * v[_] + u[1], x) - u[3, 3];
E2 := TotalDiff(-u[_] * v[3] + v[_] * v[2] + v[1], x) - TotalDiff(-2 * u[_] * v[2]
+ v[3], y);
DE2 := DifferentialEquationData([E1, E2], [u[3, 3], v[3, 3]]) : T2
:= Transformation(DE2) :
DE3 := Prolong(DE2, 1) : T3 := Transformation(DE3) :
DE4 := Prolong(DE2, 2) : T4 := Transformation(DE4) :
```

$$E1 := u_{[]} u_{2,3} + u_2 u_3 + u_2 v_2 + u_{2,2} v_{[]} + u_{1,2} - u_{3,3}$$

$$E2 := u_{[]} v_{2,3} - u_2 v_3 + 2 u_3 v_2 + v_{[]} v_{2,2} + v_2^2 + v_{1,2} - v_{3,3} \quad (1.1)$$

The symmetries have been computed both using pdsolve, and "by hand". They are spanned by the following vector fields.

```
> X1 := f1(t) D_t + \left( - \left( \frac{d}{dt} f1(t) \right) x - \frac{1}{2} \left( \frac{d^2}{dt^2} f1(t) \right) y^2 \right) D_x + \left( -u_{[]} \left( \frac{d}{dt} f1(t) \right) \right.
+ 2 y \left( \frac{d^2}{dt^2} f1(t) \right) \left. \right) D_{u[]} + \left( -2 \left( \frac{d}{dt} f1(t) \right) v_{[]} - \left( \frac{d^2}{dt^2} f1(t) \right) x \right.
- y \left( \frac{d^2}{dt^2} f1(t) \right) u_{[]} - \frac{1}{2} \left( \frac{d^3}{dt^3} f1(t) \right) y^2 \left. \right) D_{v[]} :
X2 := \left( 2 f2(t) x + \left( \frac{d}{dt} f2(t) \right) y^2 \right) D_x + f2(t) y D_y + \left( f2(t) u_{[]} \right.
```

$$\begin{aligned}
& -3y \left( \frac{d}{dt} f2(t) \right) D_{-u} + \left( 2f2(t) v_{[]} + 2 \left( \frac{d}{dt} f2(t) \right) x + 2y \left( \frac{d}{dt} f2(t) \right) u_{[]} \right. \\
& \left. + \left( \frac{d^2}{dt^2} f2(t) \right) y^2 \right) D_{-v} : \\
X3 &:= f3(t) D_{-y} + \left( \frac{d}{dt} f3(t) \right) D_{-u} : \\
X4 &:= f4(t) y D_{-x} - 2f4(t) D_{-u} + \left( f4(t) u_{[]} + \left( \frac{d}{dt} f4(t) \right) y \right) D_{-v} : \\
X5 &:= f5(t) D_{-x} + \left( \frac{d}{dt} f5(t) \right) D_{-v} :
\end{aligned}$$

The basis of vector fields can be written more consicely.

$$\begin{aligned}
> Y1 &:= evalDG \left( X1 + eval \left( X2, \left\{ f2(t) = \frac{diff(f1(t), t)}{2} \right\} \right) \right); \\
Y2 &:= X2 : Y3 := X3 : Y4 := X4 : Y5 := X5 : \\
Y1 &:= f1(t) D_{-t} + \frac{\dot{f1}(t) y}{2} D_{-y} + \left( -\frac{u_{[]} \dot{f1}(t)}{2} + \frac{y \ddot{f1}(t)}{2} \right) D_{-u_{[]}} - (\dot{f1}(t) v_{[]} D_{-v_{[]}}) \quad (1.2)
\end{aligned}$$

$$\begin{aligned}
> evalDG \left( Y1 - eval \left( Y2, f2(t) = \frac{diff(f1(t), t)}{2} \right) - X1 \right) \\
0 D_{-t} \quad (1.3)
\end{aligned}$$

The following sequences of symmetries will be usefull in computations.

$$\begin{aligned}
> Y1seq &:= k \rightarrow seq(eval(Y1, f1(t) = t^n), n = 0..k) : \\
Y2seq &:= k \rightarrow seq(eval(Y2, f2(t) = t^n), n = 0..k) : \\
Y3seq &:= k \rightarrow seq(eval(Y3, f3(t) = t^n), n = 0..k) : \\
Y4seq &:= k \rightarrow seq(eval(Y4, f4(t) = t^n), n = 0..k) : \\
Y5seq &:= k \rightarrow seq(eval(Y5, f5(t) = t^n), n = 0..k) :
\end{aligned}$$

The numbering used in the paper is the following:

$$\begin{aligned}
> Z1 &:= eval(Y5, f5(t) = a(t)); Z2 := eval(Y3, f3(t) = b(t)); Z3 := eval(Y4, f4(t) = c(t)); \\
Z4 &:= eval(Y1, f1(t) = d(t)); Z5 := eval(Y2, f2(t) = e(t)); \\
Z1 &:= a(t) D_{-x} + \left( \frac{d}{dt} a(t) \right) D_{-v_{[]}} \\
Z2 &:= b(t) D_{-y} + \left( \frac{d}{dt} b(t) \right) D_{-u_{[]}} \\
Z3 &:= c(t) y D_{-x} - 2c(t) D_{-u_{[]}} + \left( c(t) u_{[]} + \left( \frac{d}{dt} c(t) \right) y \right) D_{-v_{[]}} \\
Z4 &:= d(t) D_{-t} + \frac{\dot{d}(t) y}{2} D_{-y} + \left( -\frac{u_{[]} \dot{d}(t)}{2} + \frac{y \ddot{d}(t)}{2} \right) D_{-u_{[]}} - (\dot{d}(t) v_{[]} D_{-v_{[]}}) \\
Z5 &:= \left( 2e(t) x + \left( \frac{d}{dt} e(t) \right) y^2 \right) D_{-x} + e(t) y D_{-y} + \left( e(t) u_{[]} \right. \\
& \quad \left. - 3y \left( \frac{d}{dt} e(t) \right) \right) D_{-u_{[]}} + \left( 2e(t) v_{[]} + 2 \left( \frac{d}{dt} e(t) \right) x + 2y \left( \frac{d}{dt} e(t) \right) u_{[]} \right. \\
& \quad \left. + \left( \frac{d^2}{dt^2} e(t) \right) y^2 \right) D_{-v_{[]}} \quad (1.4)
\end{aligned}$$

We verify again that they are symmetries.

$$> simplify(Pullback(T2, (map(LieDerivative, map(Prolong, [Z1, Z2, Z3, Z4, Z5], 2)), [E1, E2])))$$

## 2.1 Modified Manakov-Santini equation and its symmetries

Verifying that the modified Manakov-Santini equations E1, E2 are EW equations.

$$\begin{aligned} & \text{> } g := \text{evalDG}(4 \, dt \, dx + 2 \, u(t, x, y) \, dt \, dy - (u(t, x, y)^2 + 4 \, v(t, x, y)) \, dt \, dt \\ & \quad - dy \, dy); \\ & g := - \left( (u(t, x, y)^2 + 4 \, v(t, x, y)) \, dt \, dt \right) + (2 \, dt) \, dx + (u(t, x, y) \, dt) \, dy \\ & \quad + (2 \, dx) \, dt + (u(t, x, y) \, dy) \, dt - (dy \, dy) \end{aligned} \quad (2.1.1)$$

$$\begin{aligned} & \text{> } \omega := \text{evalDG}((u(t, x, y) \, \text{diff}(u(t, x, y), x) + 2 \, \text{diff}(u(t, x, y), y) + 4 \, \text{diff}(v(t, x, y), x)) \, dt - \text{diff}(u(t, x, y), x) \, dy); \\ & \omega := \left( u(t, x, y) \left( \frac{\partial}{\partial x} u(t, x, y) \right) + 2 \left( \frac{\partial}{\partial y} u(t, x, y) \right) + 4 \left( \frac{\partial}{\partial x} v(t, x, y) \right) \right) dt \\ & \quad - \left( \left( \frac{\partial}{\partial x} u(t, x, y) \right) dy \right) \end{aligned} \quad (2.1.2)$$

We show that the Einstein-Weyl condition gives the modified Manakov-Santini equations.

$$\begin{aligned} & \text{> } \text{forms} := [dt, dx, dy] : \text{vfields} := [D\_t, D\_x, D\_y] : \\ & \text{> } \text{connection} := \text{Connection}(\text{add}(\text{add}(\text{add}(C[i, j, k] \, \text{vfields}[i] \, \&t \, \text{forms}[j] \\ & \quad \&t \, \text{forms}[k], k = 1 \, ..3), j = 1 \, ..3), i = 1 \, ..3)) : \\ & \text{> } \text{eq} := \text{DGinfo}(\text{evalDG}(\text{CovariantDerivative}(g, \text{connection}) - g \, \&t \, \omega), \\ & \quad \text{"CoefficientSet"}) \, \mathbf{union} \, \text{DGinfo}(\text{TorsionTensor}(\text{connection}), \text{"CoefficientSet"}) : \\ & \quad \text{nops}(\%) \end{aligned} \quad (2.1.3)$$

$$\begin{aligned} & \text{> } \text{sol} := \text{solve}(\text{eq}, \{\text{seq}(\text{seq}(\text{seq}(C[i, j, k], i = 1 \, ..3), j = 1 \, ..3), k = 1 \, ..3)\} : \\ & \text{> } \text{connection} := \text{DGsimplify}(\text{subs}(\text{sol}, \text{connection})) : \\ & \text{> } \text{EWeq} := \text{DGinfo}(\text{evalDG}(\text{SymmetrizeIndices}(\text{RicciTensor}(\text{connection}), [1, 2], \\ & \quad \text{"Symmetric"}) - f(t, x, y) \, g), \text{"CoefficientSet"}) : \\ & \text{> } \text{nops}(\text{EWeq}) \end{aligned} \quad (2.1.4)$$

$$\begin{aligned} & \text{> } \text{subs}(\text{solve}(\text{EWeq}[1], \{f(t, x, y)\}), \text{EWeq}[2]) \\ & \quad 0 \end{aligned} \quad (2.1.5)$$

$$\begin{aligned} & \text{> } \text{simplify}(\text{ToJet}(\text{simplify}(2 \, \text{subs}(\text{solve}(\text{EWeq}[1], \{f(t, x, y)\}), \text{EWeq}[3])), \{u(t, x, y), \\ & \quad v(t, x, y)\}, \text{jetnotation} = \text{jetnumbers}) + E1) \\ & \quad 0 \end{aligned} \quad (2.1.6)$$

$$\begin{aligned} & \text{> } \text{simplify}(\text{ToJet}(\text{simplify}(\text{subs}(\text{solve}(\text{EWeq}[1], \{f(t, x, y)\}), \text{EWeq}[4])), \{u(t, x, y), \\ & \quad v(t, x, y)\}, \text{jetnotation} = \text{jetnumbers}) - u[ ] \, E1 - 2 \, E2) \\ & \quad 0 \end{aligned} \quad (2.1.7)$$

## Finding symmetry algebra with pdsolve

We use pdsolve to find the symmetries.

$$\begin{aligned} & \text{> } \text{var0} := t, x, y, u[ ], v[ ] : \\ & \quad \text{vf0} := [D\_t, D\_x, D\_y, D\_u[ ], D\_v[ ]]: \\ & \text{> } X := \text{add}(a[i](\text{var0}) \cdot \text{vf0}[i], i = 1 \, ..5); \\ & X := a_1(t, x, y, u[ ], v[ ]) \, D\_t + a_2(t, x, y, u[ ], v[ ]) \, D\_x + a_3(t, x, y, u[ ], v[ ]) \, D\_y \\ & \quad + a_4(t, x, y, u[ ], v[ ]) \, D\_u[ ] + a_5(t, x, y, u[ ], v[ ]) \, D\_v[ ] \end{aligned} \quad (2.2.1)$$

$$\begin{aligned} &> \text{var2} := \text{DGinfo}(\text{MM}, \text{"FrameJetVariables"})[6..23] \\ \text{var2} &:= [u_1, u_2, u_3, v_1, v_2, v_3, u_{1,1}, u_{1,2}, u_{1,3}, u_{2,2}, u_{2,3}, u_{3,3}, v_{1,1}, v_{1,2}, v_{1,3}, v_{2,2}, v_{2,3}, \\ &\quad v_{3,3}] \end{aligned} \quad (2.2.2)$$

$$> \text{sol} := \text{pdsolve}(\text{map}(\text{coeffs}, \text{expand}(\text{Pullback}(\text{T2}, \text{LieDerivative}(\text{Prolong}(\text{X}, 2), [\text{E1}, \text{E2}]))), \text{var2})) :$$

$$> \text{solX} := \text{subs}(\text{sol}, \text{X})$$

$$\begin{aligned} \text{solX} &:= \_F1(t) D\_t + \left( \left( - \left( \frac{d}{dt} \_F1(t) \right) + 2 \_F2(t) \right) x - \frac{1}{2} y^2 \left( \frac{d^2}{dt^2} \_F1(t) \right. \right. \\ &\quad \left. \left. - 2 \left( \frac{d}{dt} \_F2(t) \right) \right) + \_F6(t) y + \_F7(t) + \_C1 \right) D\_x + (\_F2(t) y \\ &\quad + \_F3(t)) D\_y + \left( -u_{[]} \left( \frac{d}{dt} \_F1(t) \right) + \_F2(t) u_{[]} - 3 \left( \frac{d}{dt} \_F2(t) \right) y \right. \\ &\quad \left. + 2 y \left( \frac{d^2}{dt^2} \_F1(t) \right) - 2 \_F6(t) + \frac{d}{dt} \_F3(t) \right) D\_u_{[]} + \left( 2 \left( - \left( \frac{d}{dt} \_F1(t) \right) \right. \right. \\ &\quad \left. \left. + \_F2(t) \right) v_{[]} + \left( - \left( \frac{d^2}{dt^2} \_F1(t) \right) + 2 \left( \frac{d}{dt} \_F2(t) \right) \right) x \right. \\ &\quad \left. + \left( 2 \left( \frac{d}{dt} \_F2(t) \right) y - y \left( \frac{d^2}{dt^2} \_F1(t) \right) + \_F6(t) \right) u_{[]} - \frac{1}{2} y^2 \left( \frac{d^3}{dt^3} \_F1(t) \right. \right. \\ &\quad \left. \left. - 2 \left( \frac{d^2}{dt^2} \_F2(t) \right) \right) + \left( \frac{d}{dt} \_F6(t) \right) y + \frac{d}{dt} \_F7(t) \right) D\_v_{[]} \end{aligned} \quad (2.2.3)$$

$$> (\text{eval}(\text{eval}(\text{solX}, \{ \_F1(t) = f(t) \}), \{ \_C1 = 0, \text{seq}(\_F || i(t) = 0, i = 1..7) \}))$$

$$\begin{aligned} &f(t) D\_t + \left( - \left( \frac{d}{dt} f(t) \right) x - \frac{1}{2} y^2 \left( \frac{d^2}{dt^2} f(t) \right) \right) D\_x + \left( -u_{[]} \left( \frac{d}{dt} f(t) \right) \right. \\ &\quad \left. + 2 y \left( \frac{d^2}{dt^2} f(t) \right) \right) D\_u_{[]} + \left( -2 \left( \frac{d}{dt} f(t) \right) v_{[]} - \left( \frac{d^2}{dt^2} f(t) \right) x \right. \\ &\quad \left. - y \left( \frac{d^2}{dt^2} f(t) \right) u_{[]} - \frac{1}{2} y^2 \left( \frac{d^3}{dt^3} f(t) \right) \right) D\_v_{[]} \end{aligned} \quad (2.2.4)$$

>

By setting  $\_F || i(t)$  to zero, succesively, we get the following five vector fields.

$$\begin{aligned} > Q1 := f1(t) D\_t + \left( -\text{diff}(f1(t), t) x - \frac{\text{diff}(f1(t), t, t) y^2}{2} \right) D\_x + ( \\ &\quad -u_{[]} \text{diff}(f1(t), t) + 2 y \text{diff}(f1(t), t, t)) D\_u_{[]} + \left( -2 \text{diff}(f1(t), t) v_{[]} \right. \\ &\quad \left. - \text{diff}(f1(t), t, t) x - y \text{diff}(f1(t), t, t) u_{[]} - \frac{\text{diff}(f1(t), t, t, t) y^2}{2} \right) D\_v_{[]} \end{aligned}$$

$$\begin{aligned} Q1 &:= f1(t) D\_t + \left( - \left( \frac{d}{dt} f1(t) \right) x - \frac{1}{2} \left( \frac{d^2}{dt^2} f1(t) \right) y^2 \right) D\_x + \left( \right. \\ &\quad \left. -u_{[]} \left( \frac{d}{dt} f1(t) \right) + 2 y \left( \frac{d^2}{dt^2} f1(t) \right) \right) D\_u_{[]} + \left( -2 \left( \frac{d}{dt} f1(t) \right) v_{[]} \right. \\ &\quad \left. - \left( \frac{d^2}{dt^2} f1(t) \right) x - y \left( \frac{d^2}{dt^2} f1(t) \right) u_{[]} - \frac{1}{2} \left( \frac{d^3}{dt^3} f1(t) \right) y^2 \right) D\_v_{[]} \end{aligned} \quad (2.2.5)$$

$$\begin{aligned}
& > Q2 := (2 f2(t) x + \text{diff}(f2(t), t) y^2) D_x + f2(t) y D_y + (f2(t) u[] \\
& \quad - 3 y \text{diff}(f2(t), t) D_u[] + (2 f2(t) v[] + 2 \text{diff}(f2(t), t) x + 2 y \text{diff}(f2(t), \\
& \quad t) u[] + \text{diff}(f2(t), t) y^2) D_v[] \\
& Q2 := \left( 2 f2(t) x + \left( \frac{d}{dt} f2(t) \right) y^2 \right) D_x + f2(t) y D_y + \left( f2(t) u[] \right. \\
\end{aligned} \tag{2.2.6}$$

$$\begin{aligned}
& \quad - 3 y \left( \frac{d}{dt} f2(t) \right) D_u[] + \left( 2 f2(t) v[] + 2 \left( \frac{d}{dt} f2(t) \right) x \right. \\
& \quad \left. + 2 y \left( \frac{d}{dt} f2(t) \right) u[] + \left( \frac{d^2}{dt^2} f2(t) \right) y^2 \right) D_v[]
\end{aligned}$$

$$\begin{aligned}
& > Q3 := f3(t) D_y + \text{diff}(f3(t), t) D_u[] \\
& \quad Q3 := f3(t) D_y + \left( \frac{d}{dt} f3(t) \right) D_u[]
\end{aligned} \tag{2.2.7}$$

$$\begin{aligned}
& > Q4 := f4(t) y D_x - 2 f4(t) D_u[] + (f4(t) u[] + \text{diff}(f4(t), t) y) D_v[] \\
& \quad Q4 := f4(t) y D_x - 2 f4(t) D_u[] + \left( f4(t) u[] + \left( \frac{d}{dt} f4(t) \right) y \right) D_v[]
\end{aligned} \tag{2.2.8}$$

$$\begin{aligned}
& > Q5 := f5(t) D_x + \text{diff}(f5(t), t) D_v[] \\
& \quad Q5 := f5(t) D_x + \left( \frac{d}{dt} f5(t) \right) D_v[]
\end{aligned} \tag{2.2.9}$$

We check that these are the same as the ones listed above.

$$\begin{aligned}
& > X1 - Q1; X2 - Q2; X3 - Q3; X4 - Q4; X5 - Q5; \\
& \quad 0 \\
& \quad 0 \\
& \quad 0 \\
& \quad 0 \\
& \quad 0
\end{aligned} \tag{2.2.10}$$

## ▼ Finding symmetry algebra "by hand"

We verify that pdsolve found all symmetries.

$$\begin{aligned}
& > var0 := t, x, y, u[], v[] : \\
& \quad vf0 := [D_t, D_x, D_y, D_u[], D_v[]] : \\
& > X := \text{add}(a[i](var0) \cdot vf0[i], i = 1..5); \\
& X := a_1(t, x, y, u[], v[]) D_t + a_2(t, x, y, u[], v[]) D_x + a_3(t, x, y, u[], v[]) D_y \\
& \quad + a_4(t, x, y, u[], v[]) D_u[] + a_5(t, x, y, u[], v[]) D_v[]
\end{aligned} \tag{2.3.1}$$

$$\begin{aligned}
& > var2 := DGinfo(MM, "FrameJetVariables")[6..23] \\
& var2 := [u_1, u_2, u_3, v_1, v_2, v_3, u_{1,1}, u_{1,2}, u_{1,3}, u_{2,2}, u_{2,3}, u_{3,3}, v_{1,1}, v_{1,2}, v_{1,3}, v_{2,2}, v_{2,3}, \\
& \quad v_{3,3}]
\end{aligned} \tag{2.3.2}$$

We differentiate, pull back and look at the coefficients of the polynomial in variables from var2.

$$\begin{aligned}
& > eq := \{op(\text{map}(\text{coeffs}, \text{expand}(\text{Pullback}(T2, \text{LieDerivative}(\text{Prolong}(X, 2), [E1, \\
& \quad E2]))), var2))\} : \text{nops}(eq);
\end{aligned} \tag{2.3.3}$$

132

We start by solving the first 36 equations.

$$\begin{aligned}
& > EQ := [op(eq[1..36])]:
\end{aligned}$$

$\triangleright EQa1 := \{EQ[5], EQ[6], EQ[7], EQ[9], EQ[10], EQ[13], EQ[14], EQ[15],$   
 $EQ[16], EQ[17], EQ[18], EQ[27], EQ[28], EQ[29], EQ[30], EQ[31], EQ[32]\}$   
 $\vdots$   
 $EQa2 := \{eq[11], eq[19], eq[20], eq[34], eq[33]\} :$   
 $EQa3 := \{eq[8], eq[12], eq[21], eq[22], eq[23], eq[24], eq[35], eq[36]\} :$   
 $EQa4 := \{eq[1], eq[3], eq[25]\} :$   
 $EQa5 := \{eq[2], eq[4], eq[26]\} :$

$\triangleright EQa1$

$$\begin{aligned}
 & \left\{ -u_{[]} \left( \frac{\partial^2}{\partial u_{[]}^2} a_1(t, x, y, u_{[]}, v_{[]}) \right), -u_{[]} \left( \frac{\partial^2}{\partial v_{[]}^2} a_1(t, x, y, u_{[]}, v_{[]}) \right), \right. \\
 & -u_{[]} \left( \frac{\partial^2}{\partial v_{[]} \partial u_{[]}} a_1(t, x, y, u_{[]}, v_{[]}) \right), -v_{[]} \left( \frac{\partial^2}{\partial u_{[]}^2} a_1(t, x, y, u_{[]}, v_{[]}) \right), \\
 & -v_{[]} \left( \frac{\partial^2}{\partial v_{[]}^2} a_1(t, x, y, u_{[]}, v_{[]}) \right), -\left( \frac{\partial}{\partial x} a_1(t, x, y, u_{[]}, v_{[]}) \right), -2 \left( \frac{\partial}{\partial u_{[]}} a_1(t, \right. \\
 & x, y, u_{[]}, v_{[]}) \right), -\left( \frac{\partial}{\partial u_{[]}} a_1(t, x, y, u_{[]}, v_{[]}) \right), 2 \left( \frac{\partial}{\partial u_{[]}} a_1(t, x, y, u_{[]}, v_{[]}) \right), \\
 & -\left( \frac{\partial}{\partial v_{[]}} a_1(t, x, y, u_{[]}, v_{[]}) \right), 2 \left( \frac{\partial}{\partial v_{[]}} a_1(t, x, y, u_{[]}, v_{[]}) \right), -\left( \frac{\partial^2}{\partial u_{[]}^2} a_1(t, x, y, \right. \\
 & u_{[]}, v_{[]}) \right), -\left( \frac{\partial^2}{\partial v_{[]}^2} a_1(t, x, y, u_{[]}, v_{[]}) \right), -\left( \frac{\partial^2}{\partial u_{[]} \partial x} a_1(t, x, y, u_{[]}, v_{[]}) \right), \\
 & -\left( \frac{\partial^2}{\partial v_{[]} \partial x} a_1(t, x, y, u_{[]}, v_{[]}) \right), -\left( \frac{\partial^2}{\partial v_{[]} \partial u_{[]}} a_1(t, x, y, u_{[]}, v_{[]}) \right), \\
 & \left. 2 \left( \frac{\partial^2}{\partial v_{[]} \partial u_{[]}} a_1(t, x, y, u_{[]}, v_{[]}) \right) \right\}
 \end{aligned} \tag{2.3.4}$$

$$\triangleright eval(EQa1, a[1])(t, x, y, u[ ], v[ ]) = b(t, y) \tag{2.3.5}$$

$\triangleright EQa2; eval(EQa2, a[2])(t, x, y, u[ ], v[ ]) = b(t, x, y)$

$$\begin{aligned}
 & \left\{ -v_{[]} \left( \frac{\partial^2}{\partial u_{[]}^2} a_2(t, x, y, u_{[]}, v_{[]}) \right), -\left( \frac{\partial}{\partial u_{[]}} a_2(t, x, y, u_{[]}, v_{[]}) \right), -\left( \frac{\partial}{\partial v_{[]}} a_2(t, x, y, \right. \right. \\
 & u_{[]}, v_{[]}) \right), -\left( \frac{\partial^2}{\partial u_{[]}^2} a_2(t, x, y, u_{[]}, v_{[]}) \right), -\left( \frac{\partial^2}{\partial v_{[]} \partial u_{[]}} a_2(t, x, y, u_{[]}, v_{[]}) \right) \left. \right\} \\
 & \{0\}
 \end{aligned} \tag{2.3.6}$$

$\triangleright EQa3; eval(EQa3, a[3])(t, x, y, u[ ], v[ ]) = b(t, x, y)$

$$\begin{aligned}
 & \left\{ -u_{[]} \left( \frac{\partial^2}{\partial v_{[]}^2} a_3(t, x, y, u_{[]}, v_{[]}) \right), -v_{[]} \left( \frac{\partial^2}{\partial v_{[]}^2} a_3(t, x, y, u_{[]}, v_{[]}) \right), -\left( \frac{\partial}{\partial u_{[]}} a_3(t, \right. \right. \\
 & x, y, u_{[]}, v_{[]}) \right), -\left( \frac{\partial}{\partial v_{[]}} a_3(t, x, y, u_{[]}, v_{[]}) \right), -\left( \frac{\partial^2}{\partial v_{[]}^2} a_3(t, x, y, u_{[]}, v_{[]}) \right), \\
 & -\left( \frac{\partial^2}{\partial v_{[]} \partial x} a_3(t, x, y, u_{[]}, v_{[]}) \right), -\left( \frac{\partial^2}{\partial v_{[]} \partial u_{[]}} a_3(t, x, y, u_{[]}, v_{[]}) \right),
 \end{aligned}$$

$$2 \left( \frac{\partial^2}{\partial v_{[]} \partial u_{[]}} a_3(t, x, y, u_{[]}, v_{[]}) \right) \Bigg\} \quad \{0\} \quad (2.3.7)$$

$$\begin{aligned} &> EQa4; eval(EQa4, a[4](t, x, y, u_{[]}, v_{[]}) = a(t, x, y, u_{[]}) + b(t, x, y, u_{[]}) v_{[]}) \\ &\left\{ u_{[]} \left( \frac{\partial^2}{\partial v_{[]}^2} a_4(t, x, y, u_{[]}, v_{[]}) \right), v_{[]} \left( \frac{\partial^2}{\partial v_{[]}^2} a_4(t, x, y, u_{[]}, v_{[]}) \right), - \left( \frac{\partial^2}{\partial v_{[]}^2} a_4(t, x, \right. \right. \\ &\quad \left. \left. y, u_{[]}, v_{[]}) \right) \right\} \quad \{0\} \quad (2.3.8) \end{aligned}$$

$$\begin{aligned} &> EQa5; eval(EQa5, a[5](t, x, y, u_{[]}, v_{[]}) = a(t, x, y, v_{[]}) + b(t, x, y, v_{[]}) u_{[]}) \\ &\left\{ u_{[]} \left( \frac{\partial^2}{\partial u_{[]}^2} a_5(t, x, y, u_{[]}, v_{[]}) \right), v_{[]} \left( \frac{\partial^2}{\partial u_{[]}^2} a_5(t, x, y, u_{[]}, v_{[]}) \right), - \left( \frac{\partial^2}{\partial u_{[]}^2} a_5(t, x, \right. \right. \\ &\quad \left. \left. y, u_{[]}, v_{[]}) \right) \right\} \quad \{0\} \quad (2.3.9) \end{aligned}$$

$$\begin{aligned} &> subs0 := \{a[1](t, x, y, u_{[]}, v_{[]}) = A1(t, y), a[2](t, x, y, u_{[]}, v_{[]}) = A2(t, x, y), \\ &\quad a[3](t, x, y, u_{[]}, v_{[]}) = A3(t, x, y), a[4](t, x, y, u_{[]}, v_{[]}) = A4(t, x, y, u_{[]}) \\ &\quad + A5(t, x, y, u_{[]}) v_{[]}, a[5](t, x, y, u_{[]}, v_{[]}) = A6(t, x, y, v_{[]}) + A7(t, x, y, \\ &\quad v_{[]}) u_{[]}\} : \end{aligned}$$

$$> eq2 := [op(simplify(eval(eq, subs0)))] :$$

$$> eq2[2..7]$$

$$\begin{aligned} &\left[ -2 \left( \frac{\partial}{\partial u_{[]}} A5(t, x, y, u_{[]}) \right), u_{[]} \left( \frac{\partial}{\partial x} A5(t, x, y, u_{[]}) \right) - 2 \left( \frac{\partial}{\partial y} A5(t, x, y, \right. \right. \\ &\quad \left. \left. u_{[]}) \right), -2 \left( \frac{\partial}{\partial y} A1(t, y) \right) + \frac{\partial}{\partial v_{[]}} A7(t, x, y, v_{[]}), \frac{\partial}{\partial y} A1(t, y) + \frac{\partial}{\partial v_{[]}} A7(t, \right. \\ &\quad \left. x, y, v_{[]}), 2 \left( \frac{\partial}{\partial y} A1(t, y) \right) - \left( \frac{\partial}{\partial x} A3(t, x, y) \right), - \left( \frac{\partial}{\partial x} A3(t, x, y) \right) \right. \\ &\quad \left. - 2 \left( \frac{\partial}{\partial v_{[]}} A7(t, x, y, v_{[]}) \right) \right] \quad (2.3.10) \end{aligned}$$

$$\begin{aligned} &> subs1 := \{A1(t, y) = A8(t, y), A5(t, x, y, u_{[]}) = A9(t, x, y)\} \\ &\quad subs1 := \{A1(t, y) = A8(t, y), A5(t, x, y, u_{[]}) = A9(t, x, y)\} \quad (2.3.11) \end{aligned}$$

>

$$> subs2 := \{A9(t, x, y) = A10(t), A7(t, x, y, v_{[]}) = 2 v_{[]} diff(A8(t, y), y) + A11(t, x, y)\}$$

$$\begin{aligned} &subs2 := \left\{ A7(t, x, y, v_{[]}) = 2 v_{[]} \left( \frac{\partial}{\partial y} A8(t, y) \right) + A11(t, x, y), A9(t, x, y) \right. \\ &\quad \left. = A10(t) \right\} \quad (2.3.12) \end{aligned}$$

$$> eq3 := eval(eval(eq2, subs1), subs2) :$$

$$> eq3[8..11]$$

$$\left[ - \left( \frac{\partial^2}{\partial v_{[]}^2} A6(t, x, y, v_{[]}) \right), \frac{\partial^2}{\partial v_{[]}^2} A6(t, x, y, v_{[]}), 2 A10(t) - \left( \frac{\partial}{\partial x} A3(t, x, y) \right), \right. \quad (2.3.13)$$

$$-\left(\frac{\partial}{\partial x} A3(t, x, y)\right) - A10(t) \Big]$$

$$> \text{subs3} := \{A8(t, y) = A12(t), A3(t, x, y) = A13(t, y), A6(t, x, y, v[\ ]) = A14(t, x, y) + A15(t, x, y) v[\ ]\}$$

$$\text{subs3} := \{A3(t, x, y) = A13(t, y), A6(t, x, y, v[\ ]) = A14(t, x, y) + A15(t, x, y) v[\ ], \quad (2.3.14)$$

$$A8(t, y) = A12(t) \}$$

$$> \text{eq4} := \text{map}(\text{coeffs}, \text{expand}(\text{eval}(\text{eq3}, \text{subs3})), v[\ ]):$$

$$> \text{eq4}[15..21]$$

$$\left[ 2 \left( \frac{\partial}{\partial x} A14(t, x, y) \right) + 3 \left( \frac{\partial}{\partial x} A11(t, x, y) \right) u[\ ] - 2 \left( \frac{\partial}{\partial y} A11(t, x, y) \right), \quad (2.3.15)$$

$$2 \left( \frac{\partial}{\partial x} A15(t, x, y) \right), - \left( \frac{\partial}{\partial y} A14(t, x, y) \right) + \frac{\partial}{\partial t} A11(t, x, y), - \left( \frac{\partial}{\partial y} A15(t, x,$$

$$y) \right) + 2 \left( \frac{\partial}{\partial x} A11(t, x, y) \right), \frac{\partial^2}{\partial u[\ ] \partial x} A4(t, x, y, u[\ ]), \frac{\partial}{\partial x} A15(t, x, y),$$

$$\frac{\partial}{\partial x} A4(t, x, y, u[\ ]) + \frac{d}{dt} A10(t) \Big]$$

$$> \text{subs4} := \{A15(t, x, y) = A16(t, y), A4(t, x, y, u[\ ]) = A17(t, x, y) + A18(t, x, y) u[\ ],$$

$$A11(t, x, y) = \text{diff}(A2(t, x, y), y), A10(t) = 0\}$$

$$\text{subs4} := \left\{ A10(t) = 0, A11(t, x, y) = \frac{\partial}{\partial y} A2(t, x, y), A15(t, x, y) = A16(t, y), A4(t, \quad (2.3.16)$$

$$x, y, u[\ ]) = A17(t, x, y) + A18(t, x, y) u[\ ] \right\}$$

$$> \text{eq5} := \text{eval}(\text{eq4}, \text{subs4})$$

$$\text{eq5} := \left[ 0, 0, 0, 0, 0, 0, 0, 0, 0, 0, 0, 0, 0, 0, 0, 2 \left( \frac{\partial}{\partial x} A14(t, x, y) \right) \quad (2.3.17)$$

$$+ 3 u[\ ] \left( \frac{\partial^2}{\partial y \partial x} A2(t, x, y) \right) - 2 \left( \frac{\partial^2}{\partial y^2} A2(t, x, y) \right), 0, - \left( \frac{\partial}{\partial y} A14(t, x, y) \right)$$

$$+ \frac{\partial^2}{\partial y \partial t} A2(t, x, y), - \left( \frac{\partial}{\partial y} A16(t, y) \right) + 2 \left( \frac{\partial^2}{\partial y \partial x} A2(t, x, y) \right), \frac{\partial}{\partial x} A18(t, x,$$

$$y), 0, \frac{\partial}{\partial x} A17(t, x, y) + \left( \frac{\partial}{\partial x} A18(t, x, y) \right) u[\ ], 0, 0, 0, 2 \left( \frac{\partial}{\partial y} A13(t, y) \right)$$

$$- \left( \frac{\partial}{\partial x} A2(t, x, y) \right) - \left( \frac{d}{dt} A12(t) \right), - \left( \frac{\partial}{\partial x} A2(t, x, y) \right) + A18(t, x, y)$$

$$+ \frac{\partial}{\partial y} A13(t, y), -2 \left( \frac{\partial}{\partial x} A2(t, x, y) \right) + A16(t, y) + 2 \left( \frac{\partial}{\partial y} A13(t, y) \right),$$

$$-2 \left( \frac{\partial}{\partial x} A2(t, x, y) \right) + A16(t, y) + 2 \left( \frac{\partial}{\partial y} A13(t, y) \right), -A18(t, x, y)$$

$$+ \frac{\partial}{\partial x} A2(t, x, y) - \left( \frac{\partial}{\partial y} A13(t, y) \right), 2 A18(t, x, y) - 2 \left( \frac{\partial}{\partial x} A2(t, x, y) \right)$$

$$+ 2 \left( \frac{\partial}{\partial y} A13(t, y) \right), A14(t, x, y) - \left( \frac{\partial}{\partial t} A2(t, x, y) \right), -2 \left( \frac{\partial}{\partial x} A2(t, x, y) \right)$$

$$+ A16(t, y) + 2 \left( \frac{\partial}{\partial y} A13(t, y) \right), -u[\ ] \left( \frac{\partial}{\partial x} A2(t, x, y) \right) + \left( \frac{\partial}{\partial y} A13(t,$$



$$\begin{aligned}
& y) \Big) u_{[]} + A17(t, x, y) + A18(t, x, y) u_{[]} + 2 \left( \frac{\partial}{\partial y} A2(t, x, y) \right) - \left( \frac{\partial}{\partial t} A13(t, \right. \\
& y) \Big), 0, \left( \frac{\partial^3}{\partial y^2 \partial x} A2(t, x, y) \right) u_{[]}^2 + u_{[]} \left( \frac{\partial^2}{\partial y \partial x} A14(t, x, y) \right) - \left( \frac{\partial^3}{\partial y^3} A2(t, x, \right. \\
& y) \Big) u_{[]} + \left( \frac{\partial^3}{\partial y \partial x \partial t} A2(t, x, y) \right) u_{[]} - \left( \frac{\partial^2}{\partial y^2} A14(t, x, y) \right) + \frac{\partial^2}{\partial x \partial t} A14(t, x, \\
& y), \left( \frac{\partial^3}{\partial y \partial x^2} A2(t, x, y) \right) u_{[]} + \frac{\partial^2}{\partial x^2} A14(t, x, y) - \left( \frac{\partial^2}{\partial y^2} A16(t, y) \right), 0, \\
& \left( \frac{\partial^2}{\partial y \partial x} A17(t, x, y) + \left( \frac{\partial^2}{\partial y \partial x} A18(t, x, y) \right) u_{[]} \right) u_{[]} + \frac{\partial^2}{\partial x \partial t} A17(t, x, y) \\
& + \left( \frac{\partial^2}{\partial x \partial t} A18(t, x, y) \right) u_{[]} - \left( \frac{\partial^2}{\partial y^2} A17(t, x, y) \right) - \left( \frac{\partial^2}{\partial y^2} A18(t, x, y) \right) u_{[]}, \\
& \frac{\partial^2}{\partial x^2} A17(t, x, y) + \left( \frac{\partial^2}{\partial x^2} A18(t, x, y) \right) u_{[]}, 2 \left( \frac{\partial}{\partial x} A18(t, x, y) \right) u_{[]} \\
& + \frac{\partial}{\partial x} A17(t, x, y) - 2 \left( \frac{\partial}{\partial y} A18(t, x, y) \right) + \frac{\partial^2}{\partial y^2} A13(t, y), -2 \left( \frac{\partial}{\partial y} A16(t, \right. \\
& y) \Big) - \left( \frac{\partial}{\partial x} A17(t, x, y) \right) - \left( \frac{\partial}{\partial x} A18(t, x, y) \right) u_{[]} + \frac{\partial^2}{\partial y^2} A13(t, y), \\
& \left( \frac{\partial}{\partial y} A16(t, y) \right) u_{[]} + u_{[]} \left( \frac{\partial^2}{\partial y \partial x} A2(t, x, y) \right) + 2 \left( \frac{\partial}{\partial x} A14(t, x, y) \right) \\
& + 2 \left( \frac{\partial}{\partial y} A17(t, x, y) \right) + 2 \left( \frac{\partial}{\partial y} A18(t, x, y) \right) u_{[]} + \frac{\partial^2}{\partial y^2} A2(t, x, y) \\
& - \left( \frac{\partial^2}{\partial x \partial t} A2(t, x, y) \right) + \frac{\partial}{\partial t} A16(t, y), - \left( \frac{\partial^2}{\partial x^2} A2(t, x, y) \right), 2 \left( \frac{\partial}{\partial y} A18(t, x, \right. \\
& y) \Big) u_{[]} + \frac{\partial}{\partial x} A14(t, x, y) + \frac{\partial}{\partial y} A17(t, x, y) + \frac{\partial}{\partial t} A18(t, x, y) + \frac{\partial^2}{\partial y^2} A2(t, x, \\
& y) - \left( \frac{\partial^2}{\partial x \partial t} A2(t, x, y) \right), - \left( \frac{\partial^2}{\partial x^2} A2(t, x, y) \right) + 2 \left( \frac{\partial}{\partial x} A18(t, x, y) \right), 0, 0, \\
& \left. \frac{\partial^2}{\partial y \partial x} A2(t, x, y) \right]
\end{aligned}$$

$$\begin{aligned}
& \text{> subs5 := } \{A2(t, x, y) = A19(t, y) + x A20(t), A16(t, y) = A21(t)\} \\
& \quad \text{subs5 := } \{A16(t, y) = A21(t), A2(t, x, y) = A19(t, y) + x A20(t)\} \quad (2.3.18)
\end{aligned}$$

$$\begin{aligned}
& \text{> eq6 := map(coeffs, expand(eval(eq5, subs5))), u[ ])} \\
& eq6 := \left[ 0, 0, 0, 0, 0, 0, 0, 0, 0, 0, 0, 0, 0, 0, 2 \left( \frac{\partial}{\partial x} A14(t, x, y) \right) - 2 \left( \frac{\partial^2}{\partial y^2} A19(t, \right. \right. \\
& y) \Big), 0, - \left( \frac{\partial}{\partial y} A14(t, x, y) \right) + \frac{\partial^2}{\partial y \partial t} A19(t, y), 0, \frac{\partial}{\partial x} A18(t, x, y), 0, \\
& \frac{\partial}{\partial x} A17(t, x, y), \frac{\partial}{\partial x} A18(t, x, y), 0, 0, 0, 2 \left( \frac{\partial}{\partial y} A13(t, y) \right) - A20(t) \\
& - \left( \frac{d}{dt} A12(t) \right), -A20(t) + A18(t, x, y) + \frac{\partial}{\partial y} A13(t, y), -2 A20(t) + A21(t)
\end{aligned} \quad (2.3.19)$$

$$\begin{aligned}
& + 2 \left( \frac{\partial}{\partial y} A13(t, y) \right), -2 A20(t) + A21(t) + 2 \left( \frac{\partial}{\partial y} A13(t, y) \right), -A18(t, x, y) \\
& + A20(t) - \left( \frac{\partial}{\partial y} A13(t, y) \right), 2 A18(t, x, y) - 2 A20(t) + 2 \left( \frac{\partial}{\partial y} A13(t, y) \right), \\
& A14(t, x, y) - \left( \frac{\partial}{\partial t} A19(t, y) \right) - x \left( \frac{d}{dt} A20(t) \right), -2 A20(t) + A21(t) \\
& + 2 \left( \frac{\partial}{\partial y} A13(t, y) \right), A17(t, x, y) + 2 \left( \frac{\partial}{\partial y} A19(t, y) \right) - \left( \frac{\partial}{\partial t} A13(t, y) \right), \\
& -A20(t) + A18(t, x, y) + \frac{\partial}{\partial y} A13(t, y), 0, - \left( \frac{\partial^2}{\partial y^2} A14(t, x, y) \right) \\
& + \frac{\partial^2}{\partial x \partial t} A14(t, x, y), \frac{\partial^2}{\partial y \partial x} A14(t, x, y) - \left( \frac{\partial^3}{\partial y^3} A19(t, y) \right), \frac{\partial^2}{\partial x^2} A14(t, x, \\
& y), 0, \frac{\partial^2}{\partial x \partial t} A17(t, x, y) - \left( \frac{\partial^2}{\partial y^2} A17(t, x, y) \right), \frac{\partial^2}{\partial y \partial x} A17(t, x, y) \\
& + \frac{\partial^2}{\partial x \partial t} A18(t, x, y) - \left( \frac{\partial^2}{\partial y^2} A18(t, x, y) \right), \frac{\partial^2}{\partial y \partial x} A18(t, x, y), \frac{\partial^2}{\partial x^2} A17(t, x, \\
& y), \frac{\partial^2}{\partial x^2} A18(t, x, y), \frac{\partial}{\partial x} A17(t, x, y) - 2 \left( \frac{\partial}{\partial y} A18(t, x, y) \right) + \frac{\partial^2}{\partial y^2} A13(t, y), \\
& 2 \left( \frac{\partial}{\partial x} A18(t, x, y) \right), - \left( \frac{\partial}{\partial x} A17(t, x, y) \right) + \frac{\partial^2}{\partial y^2} A13(t, y), - \left( \frac{\partial}{\partial x} A18(t, x, \\
& y) \right), 2 \left( \frac{\partial}{\partial x} A14(t, x, y) \right) + 2 \left( \frac{\partial}{\partial y} A17(t, x, y) \right) + \frac{\partial^2}{\partial y^2} A19(t, y) \\
& - \left( \frac{d}{dt} A20(t) \right) + \frac{d}{dt} A21(t), 2 \left( \frac{\partial}{\partial y} A18(t, x, y) \right), 0, \frac{\partial}{\partial x} A14(t, x, y) \\
& + \frac{\partial}{\partial y} A17(t, x, y) + \frac{\partial}{\partial t} A18(t, x, y) + \frac{\partial^2}{\partial y^2} A19(t, y) - \left( \frac{d}{dt} A20(t) \right), \\
& 2 \left( \frac{\partial}{\partial y} A18(t, x, y) \right), 2 \left( \frac{\partial}{\partial x} A18(t, x, y) \right), 0, 0, 0 \Big]
\end{aligned}$$

> subs6 := {A17(t, x, y) = A22(t, y), A18(t, x, y) = A23(t), A14(t, x, y) = A24(t, y) + A25(t, y) x} :

> eq7 := eval(eq6, subs6)

$$\begin{aligned}
eq7 := & \left[ 0, 0, 0, 0, 0, 0, 0, 0, 0, 0, 0, 0, 0, 0, 0, 2 A25(t, y) - 2 \left( \frac{\partial^2}{\partial y^2} A19(t, y) \right), 0, \quad (2.3.20) \right. \\
& - \left( \frac{\partial}{\partial y} A24(t, y) \right) - \left( \frac{\partial}{\partial y} A25(t, y) \right) x + \frac{\partial^2}{\partial y \partial t} A19(t, y), 0, 0, 0, 0, 0, 0, 0, 0, \\
& 2 \left( \frac{\partial}{\partial y} A13(t, y) \right) - A20(t) - \left( \frac{d}{dt} A12(t) \right), -A20(t) + A23(t) \\
& + \frac{\partial}{\partial y} A13(t, y), -2 A20(t) + A21(t) + 2 \left( \frac{\partial}{\partial y} A13(t, y) \right), -2 A20(t) \\
& \left. + A21(t) + 2 \left( \frac{\partial}{\partial y} A13(t, y) \right), -A23(t) + A20(t) - \left( \frac{\partial}{\partial y} A13(t, y) \right), \right]
\end{aligned}$$

$$\begin{aligned}
& 2 A23(t) - 2 A20(t) + 2 \left( \frac{\partial}{\partial y} A13(t, y) \right), A24(t, y) + A25(t, y) x \\
& - \left( \frac{\partial}{\partial t} A19(t, y) \right) - x \left( \frac{d}{dt} A20(t) \right), -2 A20(t) + A21(t) + 2 \left( \frac{\partial}{\partial y} A13(t, y) \right), A22(t, y) + 2 \left( \frac{\partial}{\partial y} A19(t, y) \right) - \left( \frac{\partial}{\partial t} A13(t, y) \right), -A20(t) + A23(t) \\
& + \frac{\partial}{\partial y} A13(t, y), 0, - \left( \frac{\partial^2}{\partial y^2} A24(t, y) \right) - \left( \frac{\partial^2}{\partial y^2} A25(t, y) \right) x + \frac{\partial}{\partial t} A25(t, y), \\
& \frac{\partial}{\partial y} A25(t, y) - \left( \frac{\partial^3}{\partial y^3} A19(t, y) \right), 0, 0, - \left( \frac{\partial^2}{\partial y^2} A22(t, y) \right), 0, 0, 0, 0, \\
& \frac{\partial^2}{\partial y^2} A13(t, y), 0, \frac{\partial^2}{\partial y^2} A13(t, y), 0, 2 A25(t, y) + 2 \left( \frac{\partial}{\partial y} A22(t, y) \right) \\
& + \frac{\partial^2}{\partial y^2} A19(t, y) - \left( \frac{d}{dt} A20(t) \right) + \frac{d}{dt} A21(t), 0, 0, A25(t, y) + \frac{\partial}{\partial y} A22(t, y) \\
& y) + \frac{d}{dt} A23(t) + \frac{\partial^2}{\partial y^2} A19(t, y) - \left( \frac{d}{dt} A20(t) \right), 0, 0, 0, 0, 0 \Big]
\end{aligned}$$

$\rightarrow$  subs7 := {A22(t, y) = A26(t) + A27(t) y, A13(t, y) = A28(t) + A29(t) y} :

$\rightarrow$  eq8 := map(coeffs, eval(eq7, subs7), x)

$$\begin{aligned}
eq8 := & \left[ 0, 0, 0, 0, 0, 0, 0, 0, 0, 0, 0, 0, 0, 0, 0, 2 A25(t, y) - 2 \left( \frac{\partial^2}{\partial y^2} A19(t, y) \right), 0, \right. \\
& - \left( \frac{\partial}{\partial y} A24(t, y) \right) + \frac{\partial^2}{\partial y \partial t} A19(t, y), - \left( \frac{\partial}{\partial y} A25(t, y) \right), 0, 0, 0, 0, 0, 0, 0, 0, \\
& 2 A29(t) - A20(t) - \left( \frac{d}{dt} A12(t) \right), -A20(t) + A23(t) + A29(t), -2 A20(t) \\
& + A21(t) + 2 A29(t), -2 A20(t) + A21(t) + 2 A29(t), -A23(t) + A20(t) \\
& - A29(t), 2 A23(t) - 2 A20(t) + 2 A29(t), A24(t, y) - \left( \frac{\partial}{\partial t} A19(t, y) \right), \\
& A25(t, y) - \left( \frac{d}{dt} A20(t) \right), -2 A20(t) + A21(t) + 2 A29(t), A26(t) + A27(t) y \\
& + 2 \left( \frac{\partial}{\partial y} A19(t, y) \right) - \left( \frac{d}{dt} A28(t) \right) - \left( \frac{d}{dt} A29(t) \right) y, -A20(t) + A23(t) \\
& + A29(t), 0, - \left( \frac{\partial^2}{\partial y^2} A24(t, y) \right) + \frac{\partial}{\partial t} A25(t, y), - \left( \frac{\partial^2}{\partial y^2} A25(t, y) \right), \\
& \frac{\partial}{\partial y} A25(t, y) - \left( \frac{\partial^3}{\partial y^3} A19(t, y) \right), 0, 0, 0, 0, 0, 0, 0, 0, 0, 0, 2 A25(t, y) \\
& + 2 A27(t) + \frac{\partial^2}{\partial y^2} A19(t, y) - \left( \frac{d}{dt} A20(t) \right) + \frac{d}{dt} A21(t), 0, 0, A25(t, y) \\
& + A27(t) + \frac{d}{dt} A23(t) + \frac{\partial^2}{\partial y^2} A19(t, y) - \left( \frac{d}{dt} A20(t) \right), 0, 0, 0, 0, 0 \Big]
\end{aligned} \tag{2.3.21}$$

$\rightarrow$  subs8 := {A25(t, y) = diff(A20(t), t), A24(t, y) = diff(A19(t, y), t)} :

$\rightarrow$  eq9 := eval(eq8, subs8)

$$eq9 := \left[ 0, 0, 0, 0, 0, 0, 0, 0, 0, 0, 0, 0, 0, 0, 0, 2 \left( \frac{d}{dt} A20(t) \right) - 2 \left( \frac{\partial^2}{\partial y^2} A19(t, y) \right), \quad (2.3.22) \right.$$

$$\begin{aligned} & 0, 0, 0, 0, 0, 0, 0, 0, 0, 0, 0, 2 A29(t) - A20(t) - \left( \frac{d}{dt} A12(t) \right), -A20(t) \\ & + A23(t) + A29(t), -2 A20(t) + A21(t) + 2 A29(t), -2 A20(t) + A21(t) \\ & + 2 A29(t), -A23(t) + A20(t) - A29(t), 2 A23(t) - 2 A20(t) + 2 A29(t), 0, \\ & 0, -2 A20(t) + A21(t) + 2 A29(t), A26(t) + A27(t) y + 2 \left( \frac{\partial}{\partial y} A19(t, y) \right) \\ & - \left( \frac{d}{dt} A28(t) \right) - \left( \frac{d}{dt} A29(t) \right) y, -A20(t) + A23(t) + A29(t), 0, \\ & - \left( \frac{\partial^3}{\partial y^2 \partial t} A19(t, y) \right) + \frac{d^2}{dt^2} A20(t), 0, - \left( \frac{\partial^3}{\partial y^3} A19(t, y) \right), 0, 0, 0, 0, 0, 0, \\ & 0, 0, 0, 0, \frac{d}{dt} A20(t) + 2 A27(t) + \frac{\partial^2}{\partial y^2} A19(t, y) + \frac{d}{dt} A21(t), 0, 0, A27(t) \\ & + \frac{d}{dt} A23(t) + \frac{\partial^2}{\partial y^2} A19(t, y), 0, 0, 0, 0, 0 \end{aligned}$$

$$> subs9 := \{A19(t, y) = A30(t) + A31(t) y + A32(t) y^2\} :$$

$$> eq10 := map(coeffs, eval(eq9, subs9), y)$$

$$eq10 := \left[ 0, 0, 0, 0, 0, 0, 0, 0, 0, 0, 0, 0, 0, 0, 0, 2 \left( \frac{d}{dt} A20(t) \right) - 4 A32(t), 0, 0, 0, 0, \quad (2.3.23) \right.$$

$$\begin{aligned} & 0, 0, 0, 0, 0, 0, 0, 2 A29(t) - A20(t) - \left( \frac{d}{dt} A12(t) \right), -A20(t) + A23(t) \\ & + A29(t), -2 A20(t) + A21(t) + 2 A29(t), -2 A20(t) + A21(t) + 2 A29(t), \\ & -A23(t) + A20(t) - A29(t), 2 A23(t) - 2 A20(t) + 2 A29(t), 0, 0, -2 A20(t) \\ & + A21(t) + 2 A29(t), A26(t) + 2 A31(t) - \left( \frac{d}{dt} A28(t) \right), A27(t) + 4 A32(t) \\ & - \left( \frac{d}{dt} A29(t) \right), -A20(t) + A23(t) + A29(t), 0, -2 \left( \frac{d}{dt} A32(t) \right) \\ & + \frac{d^2}{dt^2} A20(t), 0, 0, 0, 0, 0, 0, 0, 0, 0, 0, 0, 0, \frac{d}{dt} A20(t) + 2 A27(t) \\ & + 2 A32(t) + \frac{d}{dt} A21(t), 0, 0, A27(t) + \frac{d}{dt} A23(t) + 2 A32(t), 0, 0, 0, 0, 0 \end{aligned}$$

$$\begin{aligned} & > subs10 := \left\{ A32(t) = \frac{diff(A20(t), t)}{2}, A23(t) = A20(t) - A29(t), A27(t) \right. \\ & \quad \left. = diff(A29(t), t) - 4 A32(t) \right\} : \end{aligned}$$

$$> eq11 := eval(eq10, subs10)$$

[illegible]

$$\begin{aligned} & \text{evalDG}(\text{eval}(Q, \{A12(t)=0, A30(t)=0, A31(t)=0, A29(t)=0, A28(t)=f(t)\})) \\ & \quad \text{evalDG}(\text{LieBracket}(Z1, Z2) - \text{eval}(Z1, a(t)=f(t)), \\ & \quad \text{eval}(Z4, d(t)=g(t)) - \text{eval}(Z1, a(t)=-g(t) \text{diff}(f(t), t))); \\ & \quad \text{evalDG}(\text{LieBracket}(Z1, Z5) - \text{eval}(Z1, a(t)=2 a(t) e(t))); \end{aligned} \quad (2.3.30)$$

$$\begin{aligned} & \text{evalDG}(\text{LieBracket}(Z2, Z2); \text{evalDG}(\text{LieBracket}(Z2, Z3) - \text{eval}(Z1, a(t)=b(t) c(t))); \\ & \quad \text{evalDG}(\text{LieBracket}(Z2, Z4) - \text{eval}(Z2, b(t)=\frac{1}{2} b(t) \text{diff}(d(t), t) \\ & \quad - d(t) \text{diff}(b(t), t))); \text{evalDG}(\text{LieBracket}(Z2, Z5) - \text{eval}(Z3, c(t) \\ & \quad = 2 b(t) \text{diff}(e(t), t) - \text{eval}(Z2, b(t)=b(t) e(t))); \end{aligned} \quad (2.3.31)$$

## ▼ Lie Algebra structure

$$\begin{aligned} & \text{LieBracket}(Z1, Z2); \text{LieBracket}(Z1, Z3); \text{evalDG}(\text{LieBracket}(\text{eval}(Z1, a(t)=f(t)), \\ & \quad \text{eval}(Z4, d(t)=g(t)) - \text{eval}(Z1, a(t)=-g(t) \text{diff}(f(t), t))); \\ & \quad \text{evalDG}(\text{LieBracket}(Z1, Z5) - \text{eval}(Z1, a(t)=2 a(t) e(t))); \\ & \quad 0 D_t \\ & \quad 0 D_t \\ & \quad 0 D_t \\ & \quad 0 D_t \end{aligned} \quad (2.4.1)$$

$$\begin{aligned} & \text{LieBracket}(Z2, Z2); \text{evalDG}(\text{LieBracket}(Z2, Z3) - \text{eval}(Z1, a(t)=b(t) c(t))); \\ & \quad \text{evalDG}(\text{LieBracket}(Z2, Z4) - \text{eval}(Z2, b(t)=\frac{1}{2} b(t) \text{diff}(d(t), t) \\ & \quad - d(t) \text{diff}(b(t), t))); \text{evalDG}(\text{LieBracket}(Z2, Z5) - \text{eval}(Z3, c(t) \\ & \quad = 2 b(t) \text{diff}(e(t), t) - \text{eval}(Z2, b(t)=b(t) e(t))); \\ & \quad 0 D_t \\ & \quad 0 D_t \\ & \quad 0 D_t \\ & \quad 0 D_t \end{aligned} \quad (2.4.2)$$

$$\begin{aligned} & \text{evalDG}(\text{LieBracket}(Z3, Z4) - \text{eval}(Z3, c(t)=-d(t) \text{diff}(c(t), t) \\ & \quad - \frac{\text{diff}(d(t), t) c(t)}{2})); \text{evalDG}(\text{LieBracket}(Z3, Z5) - \text{eval}(Z3, c(t) \\ & \quad = c(t) e(t))); \\ & \quad 0 D_t \\ & \quad 0 D_t \end{aligned} \quad (2.4.3)$$

$$\begin{aligned} & \text{evalDG}(\text{LieBracket}(\text{eval}(Z4, d(t)=f(t)), \text{eval}(Z4, d(t)=g(t))) - \text{eval}(Z4, d(t) \\ & \quad = f(t) \text{diff}(g(t), t) - g(t) \text{diff}(f(t), t))); \text{evalDG}(\text{LieBracket}(\text{eval}(Z4, d(t) \\ & \quad = f(t)), \text{eval}(Z5, e(t)=g(t))) - \text{eval}(Z5, e(t)=f(t) \text{diff}(g(t), t))); \\ & \quad 0 D_t \\ & \quad 0 D_t \end{aligned} \quad (2.4.4)$$

$$\begin{aligned} & \text{LieBracket}(Z5, \text{eval}(Z5, e(t)=c(t))) \\ & \quad 0 D_t \end{aligned} \quad (2.4.5)$$

## ▼ Symmetry pseudogroup

Consider the following Lie pseudogroup action.

$$\begin{aligned} & t2 := d2(t1) : y2 := \text{sqrt}(\text{diff}(d2(t1), t1)) e2(t1) y1 + b2(t1) : x2 := e2(t1)^2 x1 \\ & \quad + e2(t1) \text{diff}(e2(t1), t1) y1^2 + c2(t1) y1 + a2(t1) : \\ & \quad u2 := \frac{e2(t1) u1}{\sqrt{\frac{d}{dt1} d2(t1)}} \end{aligned}$$

$$\begin{aligned}
& + \frac{1}{2} \frac{1}{\left( \frac{d}{dt} d2(tl) \right)^{3/2} e2(tl)} \left( \left( -6 \left( \frac{d}{dt} d2(tl) \right) e2(tl) \left( \frac{d}{dt} e2(tl) \right) \right. \right. \\
& + \left. \left. \left( \frac{d^2}{dt^2} d2(tl) \right) e2(tl)^2 \right) y1 \right) \\
& + \frac{1}{2} \frac{2 e2(tl) \sqrt{\frac{d}{dt} d2(tl)} \left( \frac{d}{dt} b2(tl) \right) - 4 c2(tl) \left( \frac{d}{dt} d2(tl) \right)}{\left( \frac{d}{dt} d2(tl) \right)^{3/2} e2(tl)} : \\
v2 := & \left( \frac{2 e2(tl) \left( \frac{d}{dt} e2(tl) \right) y1}{\frac{d}{dt} d2(tl)} + \frac{c2(tl)}{\frac{d}{dt} d2(tl)} \right) u1 + \frac{e2(tl)^2 v1}{\frac{d}{dt} d2(tl)} \\
& + \frac{\left( e2(tl)^3 \left( \frac{d^2}{dt^2} e2(tl) \right) - 3 e2(tl)^2 \left( \frac{d}{dt} e2(tl) \right)^2 \right) y1^2}{\left( \frac{d}{dt} d2(tl) \right) e2(tl)^2} \\
& + \frac{\left( e2(tl)^2 \left( \frac{d}{dt} c2(tl) \right) - 4 e2(tl) c2(tl) \left( \frac{d}{dt} e2(tl) \right) \right) y1}{\left( \frac{d}{dt} d2(tl) \right) e2(tl)^2} \\
& + \frac{2 e2(tl) \left( \frac{d}{dt} e2(tl) \right) x1}{\frac{d}{dt} d2(tl)} + \frac{e2(tl)^2 \left( \frac{d}{dt} a2(tl) \right) - c2(tl)^2}{\left( \frac{d}{dt} d2(tl) \right) e2(tl)^2} :
\end{aligned}$$

### Composition of two elements from the pseudogroup

$$\begin{aligned}
> \quad & tt := eval(t2, \{t1 = d1(t)\}) : \\
& yy := eval(y2, \{t1 = d1(t), y1 = \sqrt{diff(d1(t), t)} e1(t) y + b1(t)\}) : \\
& xx := eval(x2, \{t1 = d1(t), y1 = \sqrt{diff(d1(t), t)} e1(t) y + b1(t), x1 = e1(t)^2 x \\
& \quad + e1(t) diff(e1(t), t) y^2 + c1(t) y + a1(t)\}) : \\
uu := & eval \left( u2, \left\{ t1 = d1(t), y1 = \sqrt{diff(d1(t), t)} e1(t) y + b1(t), x1 = e1(t)^2 x \right. \right.
\end{aligned}$$

$$\begin{aligned}
& + e1(t) diff(e1(t), t) y^2 + c1(t) y + a1(t), u1 = \frac{e1(t) u}{\sqrt{\frac{d}{dt} d1(t)}} \\
& + \frac{1}{2} \frac{\left( -6 \left( \frac{d}{dt} d1(t) \right) e1(t) \left( \frac{d}{dt} e1(t) \right) + \left( \frac{d^2}{dt^2} d1(t) \right) e1(t)^2 \right) y}{\left( \frac{d}{dt} d2(t) \right)^{3/2} e1(t)}
\end{aligned}$$

$$\begin{aligned}
& + \frac{1}{2} \frac{2 e l(t) \sqrt{\frac{d}{dt} d l(t)} \left( \frac{d}{dt} b l(t) \right) - 4 c l(t) \left( \frac{d}{dt} d l(t) \right)}{\left( \frac{d}{dt} d l(t) \right)^{3/2} e l(t)}, v l \\
& = \left( \frac{2 e l(t) \left( \frac{d}{dt} e l(t) \right) y}{\frac{d}{dt} d l(t)} + \frac{c l(t)}{\frac{d}{dt} d l(t)} \right) u + \frac{e l(t)^2 v}{\frac{d}{dt} d l(t)} \\
& + \frac{\left( e l(t)^3 \left( \frac{d^2}{dt^2} e l(t) \right) - 3 e l(t)^2 \left( \frac{d}{dt} e l(t) \right)^2 \right) y^2}{\left( \frac{d}{dt} d l(t) \right) e l(t)^2} \\
& + \frac{\left( e l(t)^2 \left( \frac{d}{dt} c l(t) \right) - 4 e l(t) c l(t) \left( \frac{d}{dt} e l(t) \right) \right) y}{\left( \frac{d}{dt} d l(t) \right) e l(t)^2} \\
& + \left. \frac{2 e l(t) \left( \frac{d}{dt} e l(t) \right) x}{\frac{d}{dt} d l(t)} + \frac{e l(t)^2 \left( \frac{d}{dt} a l(t) \right) - c l(t)^2}{\left( \frac{d}{dt} d l(t) \right) e l(t)^2} \right\} :
\end{aligned}$$

$$\begin{aligned}
vv := & eval(v2, \{t1 = d l(t), y1 = \text{sqrt}(\text{diff}(d l(t), t)) e l(t) y + b l(t), x1 = e l(t)^2 x \\
& + e l(t) \text{diff}(e l(t), t) y^2 + c l(t) y + a l(t)\}) :
\end{aligned}$$

### Its Lie algebra of vector fields

We show that the corresponding Lie algebra of vector fields is the Lie algebra of shape-preserving transformations.

> sol := op(eval(diff(expand([eval([t2, x2, y2, u2, v2], {d2(t1) = t1  
+ epsilon d(t1), e2(t1) = 1 + epsilon e(t1), a2(t1) = epsilon a(t1), b2(t1)  
= epsilon b(t1), c2(t1) = epsilon c(t1)})), epsilon), epsilon = 0))

$$sol := \left[ d(t1), 2 x1 e(t1) + \left( \frac{d}{dt1} e(t1) \right) y1^2 + c(t1) y1 + a(t1), \quad (2.5.2.1) \right.$$

$$\left. \frac{1}{2} y1 \left( \frac{d}{dt1} d(t1) \right) + y1 e(t1) + b(t1), u1 e(t1) + \frac{d}{dt1} b(t1) - 2 c(t1) \right.$$

$$\left. - \frac{1}{2} u1 \left( \frac{d}{dt1} d(t1) \right) - 3 y1 \left( \frac{d}{dt1} e(t1) \right) + \frac{1}{2} y1 \left( \frac{d^2}{dt1^2} d(t1) \right), \right.$$

$$\left. u1 c(t1) + 2 v1 e(t1) + 2 \left( \frac{d}{dt1} e(t1) \right) x1 + \frac{d}{dt1} a(t1) \right.$$

$$\left. - v1 \left( \frac{d}{dt1} d(t1) \right) + 2 u1 \left( \frac{d}{dt1} e(t1) \right) y1 + y1^2 \left( \frac{d^2}{dt1^2} e(t1) \right) \right.$$

$$\left. + y1 \left( \frac{d}{dt1} c(t1) \right) \right]$$

We compare these to the components of the vector fields.



> LieDerivative(Z1 + Z2 + Z3 + Z4 + Z5, t) - eval(sol[1], {t1=t, y1=y, x1=x, u1=u, v1=v}); LieDerivative(Z1 + Z2 + Z3 + Z4 + Z5, x) - eval(sol[2], {t1=t, y1=y, x1=x, u1=u, v1=v}); LieDerivative(Z1 + Z2 + Z3 + Z4 + Z5, y) - eval(sol[3], {t1=t, y1=y, x1=x, u1=u, v1=v}); LieDerivative(Z1 + Z2 + Z3 + Z4 + Z5, u[ ]) - eval(sol[4], {t1=t, y1=y, x1=x, u1=u[ ], v1=v[ ]}); LieDerivative(Z1 + Z2 + Z3 + Z4 + Z5, v[ ]) - eval(sol[5], {t1=t, y1=y, x1=x, u1=u[ ], v1=v[ ]});

0  
0  
0  
0  
0

(2.5.2.2)

> Transf := Transformation  $\left( MM, MM, \left[ \begin{array}{l} t = d(t), x = e(t)^2 x + e(t) \operatorname{diff}(e(t), t) y^2 \\ + c(t) y + a(t), y = \operatorname{diff}(d(t), t)^{\frac{1}{2}} \cdot e(t) y + b(t), u[ ] = \frac{e(t) u[ ]}{\sqrt{\frac{d}{dt} d(t)}} \\ + \frac{1}{2} \frac{\left( -6 \left( \frac{d}{dt} d(t) \right) e(t) \left( \frac{d}{dt} e(t) \right) + \left( \frac{d^2}{dt^2} d(t) \right) e(t)^2 \right) y}{\left( \frac{d}{dt} d(t) \right)^{3/2} e(t)} \\ + \frac{1}{2} \frac{2 e(t) \sqrt{\frac{d}{dt} d(t)} \left( \frac{d}{dt} b(t) \right) - 4 c(t) \left( \frac{d}{dt} d(t) \right)}{\left( \frac{d}{dt} d(t) \right)^{3/2} e(t)}, v[ ] \end{array} \right.$

$$= \left( \frac{2 e(t) \left( \frac{d}{dt} e(t) \right) y}{\frac{d}{dt} d(t)} + \frac{c(t)}{\frac{d}{dt} d(t)} \right) u[ ] + \frac{e(t)^2 v[ ]}{\frac{d}{dt} d(t)}$$

$$+ \frac{\left( e(t)^3 \left( \frac{d^2}{dt^2} e(t) \right) - 3 e(t)^2 \left( \frac{d}{dt} e(t) \right)^2 \right) y^2}{\left( \frac{d}{dt} d(t) \right) e(t)^2}$$

$$+ \frac{\left( e(t)^2 \left( \frac{d}{dt} c(t) \right) - 4 e(t) c(t) \left( \frac{d}{dt} e(t) \right) \right) y}{\left( \frac{d}{dt} d(t) \right) e(t)^2} + \frac{2 e(t) \left( \frac{d}{dt} e(t) \right) x}{\frac{d}{dt} d(t)}$$

$$\begin{aligned}
& + \frac{e(t)^2 \left( \frac{d}{dt} a(t) \right) - c(t)^2}{\left( \frac{d}{dt} d(t) \right) e(t)^2} \Bigg] \\
\text{Transf} := & \left[ t = d(t), x = e(t)^2 x + e(t) \dot{e}(t) y^2 + c(t) y + a(t), y = \sqrt{\dot{d}(t)} e(t) y \right. \\
& + b(t), u_{[]} = \frac{e(t) u_{[]}}{\sqrt{\dot{d}(t)}} + \frac{(-6 \dot{d}(t) e(t) \dot{e}(t) + \ddot{d}(t) e(t)^2) y}{2 \dot{d}(t)^{3/2} e(t)} \\
& + \frac{2 e(t) \sqrt{\dot{d}(t)} \dot{b}(t) - 4 \dot{d}(t) c(t)}{2 \dot{d}(t)^{3/2} e(t)}, v_{[]} = \left( \frac{2 e(t) \dot{e}(t) y}{\dot{d}(t)} + \frac{c(t)}{\dot{d}(t)} \right) u_{[]} \\
& + \frac{e(t)^2 v_{[]}}{\dot{d}(t)} + \frac{(e(t)^3 \ddot{e}(t) - 3 e(t)^2 \dot{e}(t)^2) y^2}{\dot{d}(t) e(t)^2} \\
& + \frac{(e(t)^2 \dot{c}(t) - 4 e(t) c(t) \dot{e}(t)) y}{\dot{d}(t) e(t)^2} + \frac{2 e(t) \dot{e}(t) x}{\dot{d}(t)} + \frac{e(t)^2 \dot{a}(t) - c(t)^2}{\dot{d}(t) e(t)^2}
\end{aligned} \tag{2.5.1}$$

## 2.2 Dimension of generic orbits

We compute the orbit dimensions on the equation inside  $J^1$ ,  $J^2$ ,  $J^3$  and  $J^4$ . The dimensions are 11, 18, 23, 28 respectively.

### First prolongation

$$\begin{aligned}
> \text{var1} := \text{DGinfo}(MM, \text{"FrameJetVariables"})[1..11] \\
& \text{var1} := [t, x, y, u_{[]}, v_{[]}, u_1, u_2, u_3, v_1, v_2, v_3]
\end{aligned} \tag{3.1}$$

$$\begin{aligned}
> \text{nops}([Y1seq(2), Y2seq(1), Y3seq(2), Y4seq(1), Y5seq(2)]) \\
& 13
\end{aligned} \tag{3.2}$$

$$\begin{aligned}
> \text{Rank}(\text{Pullback}(T2, \text{map}(\text{LieDerivative}, \text{map}(\text{Prolong}, [Y1seq(3), Y2seq(2), Y3seq(3), \\
& Y4seq(2), Y5seq(3)]), 1), \text{var1})) \\
& 11
\end{aligned} \tag{3.3}$$

### Second prolongation

$$\begin{aligned}
> \text{var2} := \text{DGinfo}(MM, \text{"FrameJetVariables"})[1..23] \\
\text{var2} := [t, x, y, u_{[]}, v_{[]}, u_1, u_2, u_3, v_1, v_2, v_3, u_{1,1}, u_{1,2}, u_{1,3}, u_{2,2}, u_{2,3}, u_{3,3}, v_{1,1}, v_{1,2}, v_{1,3}, \\
& v_{2,2}, v_{2,3}, v_{3,3}]
\end{aligned} \tag{3.4}$$

$$\begin{aligned}
> \text{nops}([Y1seq(3), Y2seq(2), Y3seq(3), Y4seq(2), Y5seq(3)]) \\
& 18
\end{aligned} \tag{3.5}$$

$$\begin{aligned}
> \text{Rank}(\text{Pullback}(T2, \text{map}(\text{LieDerivative}, \text{map}(\text{Prolong}, [Y1seq(3), Y2seq(2), Y3seq(3), \\
& Y4seq(2), Y5seq(3)]), 2), \text{var2})) \\
& 18
\end{aligned} \tag{3.6}$$

$$\begin{aligned}
> \text{Rank}(\text{subs}(u[2] = 1, u[2, 2] = 1, \text{seq}(\text{var2}[i] = 0, i = 1.. \text{nops}(\text{var2})), \text{Pullback}(T2, \\
& \text{map}(\text{LieDerivative}, \text{map}(\text{Prolong}, [Y1seq(3), Y2seq(2), Y3seq(3), Y4seq(2), \\
& Y5seq(3)]), 2), \text{var2}))) \\
& 18
\end{aligned} \tag{3.7}$$

### Third prolongation

$$\begin{aligned}
> \text{var3} := \text{DGinfo}(MM, \text{"FrameJetVariables"})[1..43] \\
&
\end{aligned} \tag{3.8}$$

$$\text{var3} := [t, x, y, u[], v[], u_1, u_2, u_3, v_1, v_2, v_3, u_{1,1}, u_{1,2}, u_{1,3}, u_{2,2}, u_{2,3}, u_{3,3}, v_{1,1}, v_{1,2}, v_{1,3}, v_{2,2}, v_{2,3}, v_{3,3}, u_{1,1,1}, u_{1,1,2}, u_{1,1,3}, u_{1,2,2}, u_{1,2,3}, u_{1,3,3}, u_{2,2,2}, u_{2,2,3}, u_{2,3,3}, u_{3,3,3}, v_{1,1,1}, v_{1,1,2}, v_{1,1,3}, v_{1,2,2}, v_{1,2,3}, v_{1,3,3}, v_{2,2,2}, v_{2,2,3}, v_{2,3,3}, v_{3,3,3}] \quad (3.8)$$

$$\begin{aligned} &> \text{Rank}(\text{subs}(u[2]=1, u[2,2]=1, \text{seq}(\text{var3}[i]=0, i=1..nops(\text{var3})), \text{Pullback}(T3, \\ &\quad \text{map}(\text{LieDerivative}, \text{map}(\text{Prolong}, [Y1seq(4), Y2seq(3), Y3seq(4), Y4seq(3), \\ &\quad Y5seq(4)], 3), \text{var3}))) \end{aligned} \quad 23 \quad (3.9)$$

#### Fourth prolongation

$$\begin{aligned} &> \text{var4} := \text{DGinfo}(MM, \text{"FrameJetVariables"})[1..73] \\ \text{var4} &:= [t, x, y, u[], v[], u_1, u_2, u_3, v_1, v_2, v_3, u_{1,1}, u_{1,2}, u_{1,3}, u_{2,2}, u_{2,3}, u_{3,3}, v_{1,1}, v_{1,2}, v_{1,3}, \end{aligned} \quad (3.10)$$

$$\begin{aligned} &\quad v_{2,2}, v_{2,3}, v_{3,3}, u_{1,1,1}, u_{1,1,2}, u_{1,1,3}, u_{1,2,2}, u_{1,2,3}, u_{1,3,3}, u_{2,2,2}, u_{2,2,3}, u_{2,3,3}, u_{3,3,3}, \\ &\quad v_{1,1,1}, v_{1,1,2}, v_{1,1,3}, v_{1,2,2}, v_{1,2,3}, v_{1,3,3}, v_{2,2,2}, v_{2,2,3}, v_{2,3,3}, v_{3,3,3}, u_{1,1,1,1}, \\ &\quad u_{1,1,1,2}, u_{1,1,1,3}, u_{1,1,2,2}, u_{1,1,2,3}, u_{1,1,3,3}, u_{1,2,2,2}, u_{1,2,2,3}, u_{1,2,3,3}, u_{1,3,3,3}, \\ &\quad u_{2,2,2,2}, u_{2,2,2,3}, u_{2,2,3,3}, u_{2,3,3,3}, u_{3,3,3,3}, v_{1,1,1,1}, v_{1,1,1,2}, v_{1,1,1,3}, v_{1,1,2,2}, \\ &\quad v_{1,1,2,3}, v_{1,1,3,3}, v_{1,2,2,2}, v_{1,2,2,3}, v_{1,2,3,3}, v_{1,3,3,3}, v_{2,2,2,2}, v_{2,2,2,3}, v_{2,2,3,3}, \\ &\quad v_{2,3,3,3}, v_{3,3,3,3}] \end{aligned}$$

$$\begin{aligned} &> \text{Rank}(\text{subs}(u[2]=1, u[2,2]=1, \text{seq}(\text{var4}[i]=0, i=1..nops(\text{var4})), \text{Pullback}(T4, \\ &\quad \text{map}(\text{LieDerivative}, \text{map}(\text{Prolong}, [Y1seq(7), Y2seq(7), Y3seq(7), Y4seq(7), \\ &\quad Y5seq(7)], 4), \text{var4}))) \end{aligned} \quad 28 \quad (3.11)$$

The equation dimension can be computed for general k, and we may compute the number of differential invariants. We see that it agrees with the Hilbert polynomial for small k.

$$\begin{aligned} &> \text{EquationNumber} := k \rightarrow \frac{2 \cdot (k-2+3) \cdot (k-2+2) \cdot (k-2+1)}{3 \cdot 2 \cdot 1} \\ &\quad \text{EquationNumber} := k \rightarrow \frac{1}{6} (2k+2) k (k-1) \end{aligned} \quad (3.12)$$

$$\begin{aligned} &> \text{DimJ} := k \rightarrow 3 + \frac{2 \cdot (k+3) \cdot (k+2) \cdot (k+1)}{3 \cdot 2 \cdot 1} \\ &\quad \text{DimJ} := k \rightarrow 3 + \frac{1}{6} (2k+6) (k+2) (k+1) \end{aligned} \quad (3.13)$$

$$\begin{aligned} &> \text{DimEq} := k \rightarrow \text{simplify}(\text{DimJ}(k) - \text{EquationNumber}(k)) \\ &\quad \text{DimEq} := k \rightarrow \text{simplify}(\text{DimJ}(k) - \text{EquationNumber}(k)) \end{aligned} \quad (3.14)$$

$$\begin{aligned} &> \text{DimEq}(k) \\ &\quad 2k^2 + 4k + 5 \end{aligned} \quad (3.15)$$

$$\begin{aligned} &> \text{DimEq}(1) - 11; \text{DimEq}(2) - 18; \text{DimEq}(3) - 23; \text{DimEq}(4) - 28; \\ &\quad 0 \\ &\quad 3 \\ &\quad 12 \\ &\quad 25 \end{aligned} \quad (3.16)$$

For general order k we refer to the proof of the paper (section 2.2). Here are some of the calculations that are not displayed in the proof.

$$\begin{aligned} &> \\ &> \text{omega}[1] := du[] - u[1] dt - u[2] dx - u[3] dy : \text{omega}[2] := dv[] - v[1] dt \\ &\quad - v[2] dx - v[3] dy : \\ &> \end{aligned}$$

$$\begin{aligned} &> \text{phi}[1] := [ \text{Hook}(Z1, \text{omega}[1]), \text{Hook}(Z1, \text{omega}[2]) ] \\ &\quad \phi_1 := \left[ -u_2 a(t), \frac{d}{dt} a(t) - v_2 a(t) \right] \end{aligned} \quad (3.17)$$

$$\begin{aligned} &> [ \text{Hook}(Z2, \text{omega}[1]), \text{Hook}(Z2, \text{omega}[2]) ]; [ \text{Hook}(Z3, \text{omega}[1]), \text{Hook}(Z3, \\ &\quad \text{omega}[2]) ]; [ \text{Hook}(Z4, \text{omega}[1]), \text{Hook}(Z4, \text{omega}[2]) ]; [ \text{Hook}(Z5, \text{omega}[1]), \\ &\quad \text{Hook}(Z5, \text{omega}[2]) ]; \\ &\quad \left[ \frac{d}{dt} b(t) - u_3 b(t), -v_3 b(t) \right] \\ &\quad \left[ -2 c(t) - u_2 c(t) y, c(t) u_{[]} + \left( \frac{d}{dt} c(t) \right) y - v_2 c(t) y \right] \\ &\quad \left[ -\frac{1}{2} u_{[]} \left( \frac{d}{dt} d(t) \right) + \frac{1}{2} y \left( \frac{d^2}{dt^2} d(t) \right) - \frac{1}{2} u_3 \left( \frac{d}{dt} d(t) \right) y - u_1 d(t), \right. \\ &\quad \left. - \left( \frac{d}{dt} d(t) \right) v_{[]} - \frac{1}{2} v_3 \left( \frac{d}{dt} d(t) \right) y - v_1 d(t) \right] \\ &\quad \left[ e(t) u_{[]} - 3 y \left( \frac{d}{dt} e(t) \right) - u_3 e(t) y - u_2 \left( 2 e(t) x + \left( \frac{d}{dt} e(t) \right) y^2 \right), 2 e(t) v_{[]} \right. \\ &\quad \left. + 2 \left( \frac{d}{dt} e(t) \right) x + 2 y \left( \frac{d}{dt} e(t) \right) u_{[]} + \left( \frac{d^2}{dt^2} e(t) \right) y^2 - v_3 e(t) y - v_2 \left( 2 e(t) x \right. \right. \\ &\quad \left. \left. + \left( \frac{d}{dt} e(t) \right) y^2 \right) \right] \end{aligned} \quad (3.18)$$

$$\begin{aligned} &> \\ &> \text{DGSimplify} \left( \text{eval} \left( \text{Prolong} \left( \text{eval} \left( \text{eval} \left( Z1, a(t) = \frac{t^m}{m!} \right), m=10 \right), 9 \right), \{t=0\} \right) \right) \\ &\quad D_{-v_{1,1,1,1,1,1,1,1,1}} \end{aligned} \quad (3.19)$$

$$\begin{aligned} &> \text{DGSimplify} \left( \text{eval} \left( \text{Prolong} \left( \text{eval} \left( \text{eval} \left( Z2, b(t) = \frac{t^m}{m!} \right), m=10 \right), 9 \right), \{t=0\} \right) \right) \\ &\quad D_{-u_{1,1,1,1,1,1,1,1,1}} \end{aligned} \quad (3.20)$$

$$\begin{aligned} &> \text{DGSimplify} \left( \text{eval} \left( \text{Prolong} \left( \text{eval} \left( \text{eval} \left( Z4, d(t) = \frac{t^m}{m!} \right), m=10 \right), 9 \right), \{t=0, y=0, u[ ] \right. \right. \\ &\quad \left. \left. =0, v[ ]=0 \right\} \right) \right) \\ &\quad \frac{1}{2} D_{-u_{1,1,1,1,1,1,1,1,3}} \end{aligned} \quad (3.21)$$

$$\begin{aligned} &> \text{DGSimplify} \left( \text{eval} \left( \text{Prolong} \left( \text{eval} \left( \text{eval} \left( Z3, c(t) = \frac{t^m}{m!} \right), m=10 \right), 10 \right), \{t=0, y=0, u[ ] \right. \right. \\ &\quad \left. \left. =0, v[ ]=0, u[2]=1, u[1]=0, u[3]=0, v[2]=0 \right\} \right) \right) \\ &\quad - (2 D_{-u_{1,1,1,1,1,1,1,1,1}}) + D_{-v_{1,1,1,1,1,1,1,1,3}} \end{aligned} \quad (3.22)$$

$$\begin{aligned} &> \text{DGSimplify} \left( \text{eval} \left( \text{Prolong} \left( \text{eval} \left( \text{eval} \left( Z5, e(t) = \frac{t^m}{m!} \right), m=10 \right), 10 \right), \{t=0, y=0, u[ ] \right. \right. \\ &\quad \left. \left. =0, v[ ]=0, u[2]=1, u[1]=0, u[3]=0, v[2]=0, x=0 \right\} \right) \right) \\ &\quad - (3 D_{-u_{1,1,1,1,1,1,1,1,3}}) + 2 D_{-v_{1,1,1,1,1,1,1,1,2}} + 2 D_{-v_{1,1,1,1,1,1,1,1,3,3}} \end{aligned} \quad (3.23)$$

## 2.3 Shape-preserving transformations

### Finding the vector fields

We find the Lie algebra of structure-preserving vector fields, coming from transformations on the base  $R^3(t, x, y)$ . We notice that this Lie algebra is the same as the symmetry algebra of the modified MS-equations.

$$\begin{aligned} & g := \text{evalDG}(4 \, dt \, dx + 2 \, u(t, x, y) \, dt \, dy - (u(t, x, y)^2 + 4 \, v(t, x, y)) \, dt \, dy \\ & \quad - dy \, dy) \\ & g := - \left( (u(t, x, y)^2 + 4 \, v(t, x, y)) \, dt \, dt + (2 \, dt \, dx + (u(t, x, y) \, dt \, dy \right. \\ & \quad \left. + (2 \, dx \, dt + (u(t, x, y) \, dy \, dt - (dy \, dy) \right) \end{aligned} \quad (4.1.1)$$

$$\begin{aligned} & \omega := \text{evalDG}((u(t, x, y) \, \text{diff}(u(t, x, y), x) + 2 \, \text{diff}(u(t, x, y), y) + 4 \, \text{diff}(v(t, x, y), x)) \, dt - \text{diff}(u(t, x, y), x) \, dy) \\ & \omega := \left( u(t, x, y) \left( \frac{\partial}{\partial x} u(t, x, y) \right) + 2 \left( \frac{\partial}{\partial y} u(t, x, y) \right) + 4 \left( \frac{\partial}{\partial x} v(t, x, y) \right) \right) dt \\ & \quad - \left( \left( \frac{\partial}{\partial x} u(t, x, y) \right) dy \right) \end{aligned} \quad (4.1.2)$$

$$\begin{aligned} & Xg := \text{DGsimplify}(\text{LieDerivative}(a1(t, x, y) \, D_t + a2(t, x, y) \, D_x + a3(t, x, y) \, D_y, g)) : \\ & X\omega := \text{DGsimplify}(\text{LieDerivative}(a1(t, x, y) \, D_t + a2(t, x, y) \, D_x + a3(t, x, y) \, D_y, \omega)) : \\ & \text{scalingcoeff} := -\text{DGinfo}(Xg, \text{"CoefficientList"}, [dy \, \& \, dy])[1] \\ & \text{scalingcoeff} := 2 \left( \frac{\partial}{\partial y} a3(t, x, y) \right) - 2 \left( \frac{\partial}{\partial y} a1(t, x, y) \right) u(t, x, y) \end{aligned} \quad (4.1.3)$$

$$\begin{aligned} & \text{op}(\text{DGinfo}(g, \text{"CoefficientList"}, [dt \, \& \, dy])); \\ & u1 := \text{op} \left( \text{DGinfo} \left( \text{evalDG} \left( \frac{Xg}{\text{scalingcoeff}} \right), \text{"CoefficientList"}, [dt \, \& \, dy] \right) \right); \\ & u1 := \left( \left( \frac{\partial}{\partial y} a3(t, x, y) \right) u(t, x, y) - \left( \frac{\partial}{\partial t} a3(t, x, y) \right) + 2 \left( \frac{\partial}{\partial y} a2(t, x, y) \right) \right. \\ & \quad \left. + \left( \frac{\partial}{\partial y} a1(t, x, y) \right) (-u(t, x, y)^2 - 4 \, v(t, x, y)) + \left( \frac{\partial}{\partial t} a1(t, x, y) \right) u(t, x, y) \right. \\ & \quad \left. + a1(t, x, y) \left( \frac{\partial}{\partial t} u(t, x, y) \right) + a2(t, x, y) \left( \frac{\partial}{\partial x} u(t, x, y) \right) + a3(t, x, y) \left( \frac{\partial}{\partial y} u(t, x, y) \right) \right) \\ & \quad \left. \right) / \left( 2 \left( \frac{\partial}{\partial y} a3(t, x, y) \right) - 2 \left( \frac{\partial}{\partial y} a1(t, x, y) \right) u(t, x, y) \right) \end{aligned} \quad (4.1.4)$$

$$\begin{aligned} & \mu := \text{simplify}(\text{scalingcoeff} \cdot (u1 - u(t, x, y))) \\ & \mu := \left( \frac{\partial}{\partial y} a1(t, x, y) \right) u(t, x, y)^2 - 4 \left( \frac{\partial}{\partial y} a1(t, x, y) \right) v(t, x, y) + \left( \frac{\partial}{\partial t} a1(t, x, y) \right) u(t, x, y) \\ & \quad - \left( \frac{\partial}{\partial y} a3(t, x, y) \right) u(t, x, y) + a1(t, x, y) \left( \frac{\partial}{\partial t} u(t, x, y) \right) \\ & \quad + a2(t, x, y) \left( \frac{\partial}{\partial x} u(t, x, y) \right) + a3(t, x, y) \left( \frac{\partial}{\partial y} u(t, x, y) \right) + 2 \left( \frac{\partial}{\partial y} a2(t, x, y) \right) \\ & \quad - \left( \frac{\partial}{\partial t} a3(t, x, y) \right) \end{aligned} \quad (4.1.5)$$

$$- \frac{\text{op}(\text{DGinfo}(g, \text{"CoefficientList"}, [dt \, \& \, dt])) + u(t, x, y)^2}{4};$$

```

vI := simplify(
  op( DGinfo( evalDG(  $\frac{Xg}{scalingcoeff}$  ), "CoefficientList", [dt &t dt] ) ) + uI2 )
  -  $\frac{v(t, x, y)}{4}$  );

vI := ( -  $\frac{1}{2}$  (  $\frac{\partial}{\partial t}$  a3(t, x, y) ) u(t, x, y) - (  $\frac{\partial}{\partial t}$  a2(t, x, y) ) -  $\frac{1}{2}$  (  $\frac{\partial}{\partial t}$  aI(t, x, y) ) ( (4.1.6)
  - u(t, x, y)2 - 4 v(t, x, y) ) -  $\frac{1}{4}$  aI(t, x, y) ( - 2 u(t, x, y) (  $\frac{\partial}{\partial t}$  u(t, x, y) )
  - 4 (  $\frac{\partial}{\partial t}$  v(t, x, y) ) ) -  $\frac{1}{4}$  a2(t, x, y) ( - 2 u(t, x, y) (  $\frac{\partial}{\partial x}$  u(t, x, y) )
  - 4 (  $\frac{\partial}{\partial x}$  v(t, x, y) ) ) -  $\frac{1}{4}$  a3(t, x, y) ( - 2 u(t, x, y) (  $\frac{\partial}{\partial y}$  u(t, x, y) )
  - 4 (  $\frac{\partial}{\partial y}$  v(t, x, y) ) ) ) / ( 2 (  $\frac{\partial}{\partial y}$  a3(t, x, y) ) - 2 (  $\frac{\partial}{\partial y}$  aI(t, x, y) ) u(t, x,
  y) ) -  $\frac{1}{4}$  ( - (  $\frac{\partial}{\partial y}$  aI(t, x, y) ) u(t, x, y)2 - 4 (  $\frac{\partial}{\partial y}$  aI(t, x, y) ) v(t, x, y)
  + (  $\frac{\partial}{\partial t}$  aI(t, x, y) ) u(t, x, y) + (  $\frac{\partial}{\partial y}$  a3(t, x, y) ) u(t, x, y) + aI(t, x,
  y) (  $\frac{\partial}{\partial t}$  u(t, x, y) ) + a2(t, x, y) (  $\frac{\partial}{\partial x}$  u(t, x, y) ) + a3(t, x, y) (  $\frac{\partial}{\partial y}$  u(t, x, y) )
  + 2 (  $\frac{\partial}{\partial y}$  a2(t, x, y) ) - (  $\frac{\partial}{\partial t}$  a3(t, x, y) ) )2 / ( 2 (  $\frac{\partial}{\partial y}$  a3(t, x, y) )
  - 2 (  $\frac{\partial}{\partial y}$  aI(t, x, y) ) u(t, x, y) )2

> nu := simplify( scalingcoeff (  $\frac{1}{4}$  ( uI2 - u(t, x, y)2 ) + vI - v(t, x, y) ) -  $\frac{1}{2}$  u(t, x, y)
  · mu )

v := 4 (  $\frac{\partial}{\partial y}$  aI(t, x, y) ) u(t, x, y) v(t, x, y) - (  $\frac{\partial}{\partial y}$  a2(t, x, y) ) u(t, x, y) (4.1.7)
  + 2 (  $\frac{\partial}{\partial t}$  aI(t, x, y) ) v(t, x, y) + (  $\frac{\partial}{\partial x}$  v(t, x, y) ) a2(t, x, y) - 2 (  $\frac{\partial}{\partial y}$  a3(t, x,
  y) ) v(t, x, y) + aI(t, x, y) (  $\frac{\partial}{\partial t}$  v(t, x, y) ) + a3(t, x, y) (  $\frac{\partial}{\partial y}$  v(t, x, y) )
  - (  $\frac{\partial}{\partial t}$  a2(t, x, y) )

>
> lg := evalDG( scalingcoeff g + 2 mu dt &s dy - ( 2 u(t, x, y) · mu + 4 nu ) dt &t dt ) :
  lω := evalDG( ( diff( u(t, x, y) · mu, x ) + 2 diff( mu, y ) + 4 diff( nu, x ) ) · dt - diff( mu,
  x ) · dy + ExteriorDerivative( scalingcoeff ) ) :
> EQ := ToJet( DGinfo( evalDG( Xg - lg ), "CoefficientSet" ) ) union DGinfo( evalDG( Xω
  - lω ), "CoefficientSet" ), { u(t, x, y), v(t, x, y) }, jetnotation = jetnumbers ) :
> sol := pdsolve( map( coeffs, numer( expand( EQ ) ), [ u[ ], u[1], u[2], u[3], u[1,1],
  u[1,2], u[1,3], u[2,2], u[2,3], u[3,3], v[ ], v[1], v[2], v[3], v[1,1], v[1,2],
  v[1,3], v[2,2], v[2,3], v[3,3] ] ) ) :

```

$$\begin{aligned}
& \text{eval}(a1(t, x, y) D_t + a2(t, x, y) D_x + a3(t, x, y) D_y, sol) \\
& \_F1(t) D_t + \left( \_F4(t) x + \frac{1}{2} \left( \frac{d}{dt} \_F4(t) \right) y^2 + \_F5(t) y + \_F6(t) \right) D_x \\
& + \left( \frac{1}{2} \left( \frac{d}{dt} \_F1(t) + \_F4(t) \right) y + \_F7(t) \right) D_y
\end{aligned} \tag{4.1.8}$$

## The Lie pseudogroup of shape-preserving transformations

The Lie pseudogroup action is given by

$$\begin{aligned}
& t2 := d2(t1) : y2 := \text{sqrt}(\text{diff}(d2(t1), t1)) e2(t1) y1 + b2(t1) : x2 := e2(t1)^2 x1 \\
& + e2(t1) \text{diff}(e2(t1), t1) y1^2 + c2(t1) y1 + a2(t1) :
\end{aligned}$$

We verify that it is closed under composition.

$$\begin{aligned}
& \text{eval}(\text{diff}(\text{simplify}(\text{eval}([t2, y2, x2], \{d2(t1) = 1 + \text{epsilon}[4] d(t1), e2(t1) = 1 \\
& + \text{epsilon}[5] e(t1), c2(t1) = \text{epsilon}[3] c(t1), a2(t1) = \text{epsilon}[1] a(t1), b2(t1) \\
& = \text{epsilon}[2] b(t1)\})), \text{epsilon}[5]), \{\text{epsilon}[4] = 0, \text{epsilon}[5] = 1\})
\end{aligned}$$

$$\begin{aligned}
& \left[ 0, 0, 2(1 + e(t1)) x1 e(t1) + e(t1) \left( \frac{d}{dt1} e(t1) \right) y1^2 + (1 \right. \\
& \left. + e(t1)) \left( \frac{d}{dt1} e(t1) \right) y1^2 \right]
\end{aligned} \tag{4.2.1}$$

$$\begin{aligned}
& tt := \text{eval}(t2, \{t1 = d1(t)\}) : \\
& yy := \text{eval}(y2, \{t1 = d1(t), y1 = \text{sqrt}(\text{diff}(d1(t), t)) e1(t) y + b1(t)\}) : \\
& xx := \text{eval}(x2, \{t1 = d1(t), y1 = \text{sqrt}(\text{diff}(d1(t), t)) e1(t) y + b1(t), x1 = e1(t)^2 x \\
& + e1(t) \text{diff}(e1(t), t) y^2 + c1(t) y + a1(t)\}) :
\end{aligned}$$

$$\begin{aligned}
& DD := tt; BB := \text{simplify}(\text{eval}(yy, y=0)); EE := \text{simplify}(\text{sqrt}(\text{diff}(xx, x)), \\
& \text{symbolic}); AA := \text{eval}(xx, \{x=0, y=0\}); CC := \text{eval}(\text{diff}(xx, y), y=0); \\
& DD := d2(d1(t))
\end{aligned}$$

$$BB := \sqrt{\frac{d}{dt1} d2(t1) \Big|_{t1=d1(t)}} e2(d1(t)) b1(t) + b2(d1(t))$$

$$EE := e2(d1(t)) e1(t)$$

$$\begin{aligned}
AA := & e2(d1(t))^2 a1(t) + e2(d1(t)) \left( \frac{d}{dt1} e2(t1) \Big|_{t1=d1(t)} \right) b1(t)^2 \\
& + c2(d1(t)) b1(t) + a2(d1(t))
\end{aligned}$$

$$\begin{aligned}
CC := & e2(d1(t))^2 c1(t) + 2 e2(d1(t)) \left( \frac{d}{dt1} e2(t1) \Big|_{t1=d1(t)} \right) \\
& b1(t) \sqrt{\frac{d}{dt} d1(t) e1(t) + c2(d1(t))} \sqrt{\frac{d}{dt} d1(t) e1(t)}
\end{aligned} \tag{4.2.2}$$

$$\begin{aligned}
& \text{simplify}(\text{sqrt}(\text{diff}(DD, t)) \cdot EE - \text{diff}(yy, y), \text{symbolic}) \\
& 0
\end{aligned} \tag{4.2.3}$$

$$\begin{aligned}
& \text{simplify}(\text{eval}(yy, y=0) - BB) \\
& 0
\end{aligned} \tag{4.2.4}$$

$$\begin{aligned}
& \text{simplify}(\text{eval}(xx, \{x=0, y=0\}) - AA) \\
& 0
\end{aligned} \tag{4.2.5}$$

$$\begin{aligned}
& \text{simplify}(\text{eval}(\text{diff}(xx, x), \{x=0, y=0\}) - EE^2) \\
& 0
\end{aligned} \tag{4.2.6}$$

$$0 \quad (4.2.6)$$

$$> \text{simplify}(\text{eval}(\text{diff}(xx, y), \{x=0, y=0\}) - CC) \quad (4.2.7)$$

$$> \text{simplify}\left(\frac{\text{diff}(xx, y, y)}{2} - EE \text{diff}(EE, t), \text{symbolic}\right) \quad (4.2.8)$$

$$\begin{aligned} > \text{Transf} := \text{Transformation}\left(MM, MM, \left[t = d(t), x = e(t)^2 x + e(t) \text{diff}(e(t), t) y^2 \right. \right. \\ &\quad \left. \left. + c(t) y + a(t), y = \text{diff}(d(t), t) \frac{1}{2} \cdot e(t) y + b(t), u[] = u[], v[] = v[]\right]\right) \\ \text{Transf} := &\left[t = d(t), x = e(t)^2 x + e(t) \dot{e}(t) y^2 + c(t) y + a(t), y = \sqrt{d(t)} e(t) y \right. \\ &\left. + b(t), u[] = u[], v[] = v[]\right] \end{aligned} \quad (4.2.9)$$

We show that the corresponding Lie algebra of vector fields is the Lie algebra of shape-preserving transformations.

$$\begin{aligned} > \text{eval}(\text{diff}(\text{expand}([\text{eval}([t2, x2, y2, u2, v2], \{d2(t1) = t1 + \text{epsilon} d(t1), e2(t1) = 1 \\ &\quad + \text{epsilon} e(t1), a2(t1) = \text{epsilon} a(t1), b2(t1) = \text{epsilon} b(t1), c2(t1) \\ &\quad = \text{epsilon} c(t1)\}]), \text{epsilon}), \text{epsilon} = 0) \\ &\left[\left[d(t1), 2 x1 e(t1) + \left(\frac{d}{dt1} e(t1)\right) y1^2 + c(t1) y1 + a(t1), \frac{1}{2} y1 \left(\frac{d}{dt1} d(t1)\right) \right. \right. \\ &\quad \left. \left. + y1 e(t1) + b(t1)\right]\right] \end{aligned} \quad (4.2.10)$$

We compare these to the components of the vector fields.

$$\begin{aligned} > \text{LieDerivative}(Z1 + Z2 + Z3 + Z4 + Z5, t); \text{LieDerivative}(Z1 + Z2 + Z3 + Z4 + Z5, \\ &\quad x); \text{LieDerivative}(Z1 + Z2 + Z3 + Z4 + Z5, y); \\ &\quad d(t) \\ &\quad 2 e(t) x + \left(\frac{d}{dt} e(t)\right) y^2 + c(t) y + a(t) \\ &\quad e(t) y + \frac{1}{2} \left(\frac{d}{dt} d(t)\right) y + b(t) \end{aligned} \quad (4.2.11)$$

## ▼ Lift of pseudogroup

$$\begin{aligned} > \text{unassign}('tt', 'xx', 'yy') : \\ > \text{DGsetup}([t, x, y], M) : \\ > \text{DGsetup}([tt, xx, yy], N) : \\ > T := \text{Transformation}(M, N, [tt = d(t), xx = e(t)^2 x + e(t) \text{diff}(e(t), t) y^2 + c(t) y \\ &\quad + a(t), yy = \text{sqrt}((\text{diff}(d(t), t))) e(t) y + b(t)]) : \\ > \text{scalingcoeff} := -\text{DGinfo}(\text{Pullback}(T, 4 \text{dtt} \&s \text{dxx} + 2 \text{uu} \text{dtt} \&s \text{dyy} - (\text{uu}^2 \\ &\quad + 4 \text{vv}) \text{dtt} \&s \text{dtt} - \text{dyy} \&s \text{dyy}), \text{"CoefficientList"}, [\text{dy} \&t \text{dy}])[1] \\ &\quad \text{scalingcoeff} := \left(\frac{d}{dt} d(t)\right) e(t)^2 \end{aligned} \quad (4.3.1)$$

$$\begin{aligned} > \text{ContractIndices}(\text{evalDG}(4 \text{dtt} \&s \text{dxx} + 2 \text{uu} \text{dtt} \&s \text{dyy} - (\text{uu}^2 + 4 \text{vv}) \text{dtt} \&s \text{dtt} \\ &\quad - \text{dyy} \&s \text{dyy}), D\_tt \&t D\_yy, [[1, 1], [2, 2]]) \\ &\quad uu \end{aligned} \quad (4.3.2)$$



>  $u1 := \text{ContractIndices}\left(\text{evalDG}\left(\frac{1}{\text{scalingcoeff}} \text{Pullback}(T, 4 \text{ dtt} \&s \text{ dxx} + 2 \text{ uu} \text{ dtt} \&s \text{ dyy} - (uu^2 + 4 \text{ vv}) \text{ dtt} \&s \text{ dtt} - \text{dyy} \&s \text{ dyy})\right), D\_t \&t D\_y, [[1, 1], [2, 2]]\right)$

$$u1 := -\frac{1}{2} \frac{1}{e(t)^2 \left(\frac{d}{dt} d(t)\right)} \left( -2 \text{ uu} \left(\frac{d}{dt} d(t)\right)^{3/2} e(t) + e(t)^2 \left(\frac{d^2}{dt^2} d(t)\right) y \right. \\ \left. - 6 \left(\frac{d}{dt} d(t)\right) e(t) \left(\frac{d}{dt} e(t)\right) y + 2 e(t) \sqrt{\frac{d}{dt} d(t)} \left(\frac{d}{dt} b(t)\right) \right. \\ \left. - 4 c(t) \left(\frac{d}{dt} d(t)\right) \right) \quad (4.3.3)$$

>  $\text{simplify}\left(-\frac{1}{4} \left(\text{ContractIndices}(\text{evalDG}(4 \text{ dtt} \&s \text{ dxx} + 2 \text{ uu} \text{ dtt} \&s \text{ dyy} - (uu^2 + 4 \text{ vv}) \text{ dtt} \&s \text{ dtt} - \text{dyy} \&s \text{ dyy}), D\_t \&t D\_t, [[1, 1], [2, 2]]) + uu^2\right)\right)$

vv

(4.3.4)

>  $v1 := \text{simplify}\left(-\frac{1}{4} \left(\text{ContractIndices}\left(\text{evalDG}\left(\frac{1}{\text{scalingcoeff}} \text{Pullback}(T, 4 \text{ dtt} \&s \text{ dxx} + 2 \text{ uu} \text{ dtt} \&s \text{ dyy} - (uu^2 + 4 \text{ vv}) \text{ dtt} \&s \text{ dtt} - \text{dyy} \&s \text{ dyy})\right), D\_t \&t D\_t, [[1, 1], [2, 2]]\right) + u1^2\right)\right)$

$$v1 := \frac{1}{2} \frac{1}{\left(\frac{d}{dt} d(t)\right) e(t)^4} \left( -4 \text{ uu} e(t) \left(e(t) \left(\frac{d}{dt} e(t)\right) y \right. \right. \\ \left. \left. + \frac{1}{2} c(t) \right) \left(\frac{d}{dt} d(t)\right)^{3/2} + 4 \left(\frac{d}{dt} b(t)\right) e(t) \left(e(t) \left(\frac{d}{dt} e(t)\right) y \right. \right. \\ \left. \left. + \frac{1}{2} c(t) \right) \sqrt{\frac{d}{dt} d(t)} + \left(2 e(t)^3 \left(\frac{d}{dt} e(t)\right) y^2 + e(t)^2 y c(t)\right) \left(\frac{d^2}{dt^2} d(t)\right) \right. \\ \left. - 4 \left(\frac{d}{dt} d(t)\right) \left(\frac{1}{2} e(t)^3 \left(\frac{d^2}{dt^2} e(t)\right) y^2 - \frac{1}{2} e(t)^2 \left(\frac{d}{dt} d(t)\right) \text{ vv} \right. \right. \\ \left. \left. + \frac{3}{2} e(t)^2 \left(\frac{d}{dt} e(t)\right)^2 y^2 + e(t) \left(e(t)^2 x + \frac{3}{2} c(t) y\right) \left(\frac{d}{dt} e(t)\right) \right. \right. \\ \left. \left. + \frac{1}{2} e(t)^2 \left(\frac{d}{dt} c(t)\right) y + \frac{1}{2} e(t)^2 \left(\frac{d}{dt} a(t)\right) + \frac{1}{2} c(t)^2 \right) \right) \quad (4.3.5)$$

>  $\text{sol} := (\text{solve}(\{v1 - v, u1 - u\}, \{\text{uu}, \text{vv}\})) :$

>  $\text{collect}(\text{eval}(\text{uu}, \text{sol}), [u, y])$

$$\frac{e(t) u}{\sqrt{\frac{d}{dt} d(t)}} + \frac{1}{2} \frac{\left(-6 \left(\frac{d}{dt} d(t)\right) e(t) \left(\frac{d}{dt} e(t)\right) + \left(\frac{d^2}{dt^2} d(t)\right) e(t)^2\right) y}{\left(\frac{d}{dt} d(t)\right)^{3/2} e(t)} \quad (4.3.6)$$

$$+ \frac{1}{2} \frac{2 e(t) \sqrt{\frac{d}{dt} d(t)} \left( \frac{d}{dt} b(t) \right) - 4 c(t) \left( \frac{d}{dt} d(t) \right)}{\left( \frac{d}{dt} d(t) \right)^{3/2} e(t)}$$

>

> collect(eval(vv, sol), [v, u, y, x])

$$\begin{aligned} & \left( \frac{2 e(t) \left( \frac{d}{dt} e(t) \right) y}{\frac{d}{dt} d(t)} + \frac{c(t)}{\frac{d}{dt} d(t)} \right) u + \frac{e(t)^2 v}{\frac{d}{dt} d(t)} \\ & + \frac{\left( e(t)^3 \left( \frac{d^2}{dt^2} e(t) \right) - 3 e(t)^2 \left( \frac{d}{dt} e(t) \right)^2 \right) y^2}{\left( \frac{d}{dt} d(t) \right) e(t)^2} \\ & + \frac{\left( e(t)^2 \left( \frac{d}{dt} c(t) \right) - 4 e(t) c(t) \left( \frac{d}{dt} e(t) \right) \right) y}{\left( \frac{d}{dt} d(t) \right) e(t)^2} + \frac{2 e(t) \left( \frac{d}{dt} e(t) \right) x}{\frac{d}{dt} d(t)} \\ & + \frac{e(t)^2 \left( \frac{d}{dt} a(t) \right) - c(t)^2}{\left( \frac{d}{dt} d(t) \right) e(t)^2} \end{aligned} \quad (4.3.7)$$

## ▼ Lifts of shape-preserving vector fields are point symmetries

The point symmetries can be recovered from the shape-preserving vector fields.

The metric as a horizontal 2-form:

$$> g := 4 dt \&s dx + 2 u[ ] dt \&s dy - (u[ ]^2 + 4 v[ ]) dt \&s dt - dy \&s dy :$$

We would like to lift a general shape-preserving vector field. The requirement that the Lie-derivative of g be proportional to g, determines A and B uniquely.

$$> Z := 2 d(t) D_{-t} + (a(t) + y c(t) + 2 x e(t) + y^2 \text{diff}(e(t), t)) D_{-x} + (b(t) + y \text{diff}(d(t), t) + y e(t)) D_{-y} + A D_{-u}[ ] + B D_{-v}[ ] :$$

>

$$> coefficient := -op(DGinfo(LieDerivative(Z, g), "CoefficientList", [dy \&t dy]))$$

$$coefficient := 2 \left( \frac{d}{dt} d(t) \right) + 2 e(t) \quad (4.4.1)$$

$$> sol := solve(DGinfo(evalDG(LieDerivative(Z, g) - coefficient g), "CoefficientSet"), \{A, B\})$$

$$\begin{aligned} sol := & \left\{ A = -u_{[ ]} \left( \frac{d}{dt} d(t) \right) + y \left( \frac{d^2}{dt^2} d(t) \right) + e(t) u_{[ ]} - 3 y \left( \frac{d}{dt} e(t) \right) \right. \\ & + \frac{d}{dt} b(t) - 2 c(t), B = \left( \frac{d^2}{dt^2} e(t) \right) y^2 + 2 y \left( \frac{d}{dt} e(t) \right) u_{[ ]} \\ & - 2 \left( \frac{d}{dt} d(t) \right) v_{[ ]} + \left( \frac{d}{dt} c(t) \right) y + c(t) u_{[ ]} + 2 e(t) v_{[ ]} + 2 \left( \frac{d}{dt} e(t) \right) x \\ & \left. + \frac{d}{dt} a(t) \right\} \end{aligned} \quad (4.4.2)$$

We see that we get the point symmetries, and check that the lift behaves appropriately on our 1-form.

$$\begin{aligned} &> \text{eval}(\text{evalDG}(\text{eval}(Z, \text{sol}) - (Y1 + Y2 + Y3 + Y4 + Y5)), \{f1(t) = 2 d(t), f5(t) \\ &= a(t), f2(t) = e(t), f4(t) = c(t), f3(t) = b(t)\}) \\ &\quad 0 D_t + 0 D_x + 0 D_y + 0 D_u + 0 D_v \end{aligned} \quad (4.4.3)$$

$$\begin{aligned} &> \text{LieDerivative}(\text{Prolong}(\text{eval}(Z, \text{sol}), 1), (u[1] u[2] + 2 u[3] + 4 v[2]) dt - u[2] dy) \\ &\quad - \text{ExteriorDerivative}(\text{coefficient}) \\ &\quad 0 \end{aligned} \quad (4.4.4)$$

### 3.2 Differential invariants of second order and invariant derivations

> *ChangeFrame*(MM) :

$$\begin{aligned} &> I1 := \frac{u_{2,3} + v_{2,2}}{u_2^2} : I2 := \frac{u_2^2 u_{2,3} + u_2 u_{2,2} v_2 + u_{2,2} u_{3,3} - u_{2,3}^2}{u_2^4} : I3 \\ &:= \frac{u_2^2 v_{2,2} - u_2 u_{2,2} v_2 + u_{2,2} v_{2,3} - u_{2,3} v_{2,2}}{u_2^4} : \end{aligned}$$

We check that they are invariant under the Lie algebra action.

$$\begin{aligned} &> \text{simplify}(\text{map}(\text{LieDerivative}, \text{map}(\text{Prolong}, [X1, X2, X3, X4, X5], 2), [I1, I2, I3])) \\ &\quad [[0, 0, 0], [0, 0, 0], [0, 0, 0], [0, 0, 0], [0, 0, 0]] \end{aligned} \quad (5.1)$$

We check that they are independent. They are independent both on the equation, and outside.

$$\begin{aligned} &> \text{var2} := [u[1, 1], u[1, 2], u[1, 3], u[2, 2], u[2, 3], u[3, 3], v[1, 1], v[1, 2], v[1, 3], v[2, \\ &2], v[2, 3], v[3, 3]] \\ &\quad \text{var2} := [u_{1,1}, u_{1,2}, u_{1,3}, u_{2,2}, u_{2,3}, u_{3,3}, v_{1,1}, v_{1,2}, v_{1,3}, v_{2,2}, v_{2,3}, v_{3,3}] \end{aligned} \quad (5.2)$$

$$\begin{aligned} &> \text{Rank}([\text{seq}(\text{diff}(\text{Pullback}(T2, [I1, I2, I3]), \text{var2}[i]), i = 1 .. \text{nops}(\text{var2}))]) \\ &\quad 3 \end{aligned} \quad (5.3)$$

$$\begin{aligned} &> \text{Rank}([\text{seq}(\text{diff}([I1, I2, I3], \text{var2}[i]), i = 1 .. \text{nops}(\text{var2}))]) \\ &\quad 3 \end{aligned} \quad (5.4)$$

When restricted to sections, I1, I2, I3 gives a new set of local coordinates around almost any point. The exception is given by the following set.

$$\begin{aligned} &> \text{SingularSet} := \text{factor}(\text{Determinant}([\text{simplify}(\text{map}(\text{TotalDiff}, [I1, I2, I3], t)), \\ &\quad \text{simplify}(\text{map}(\text{TotalDiff}, [I1, I2, I3], x)), \text{simplify}(\text{map}(\text{TotalDiff}, [I1, I2, I3], y)))] : \end{aligned}$$

>

>

$$\begin{aligned} &> D1 := \text{proc}(\text{funct}) \\ &\quad \text{simplify}\left(\frac{u_2}{u_{2,2}} \text{TotalDiff}(\text{funct}, x)\right); \\ &\text{end proc;} \\ &D2 := \text{proc}(\text{funct}) \\ &\quad \text{simplify}\left(\frac{u_{2,3}}{u_2 u_{2,2}} \text{TotalDiff}(\text{funct}, x) - \frac{1}{u_2} \text{TotalDiff}(\text{funct}, y)\right); \\ &\text{end proc;} \\ &D3 := \text{proc}(\text{funct}) \\ &\quad \text{simplify}\left(\frac{1}{u[2]^3} (u[2, 2] \text{TotalDiff}(\text{funct}, t) + (v[1] u_{2,2} + v_2 u_2 + u[3, \end{aligned}$$

3])  $TotalDiff(funct, x) + (u_{[1]} u_{2,2} + u_{2,2}^2 - 2 u_{2,3}) TotalDiff(funct, y) \Big)$ ;

end proc:

## Commutation relations of derivations

The following four functions appear in the commutation relations of the derivations.

$$\begin{aligned}
 & K1 := \text{expand} \left( \frac{u_2 u_{2,2,2}}{u_{2,2}^2} - 3 \right) : K2 := - \frac{u_{2,2} u_{2,2,3} - u_{2,3} u_{2,2,2}}{u_2 u_{2,2}^2} : \\
 & K3 := K2 \cdot \left( 1 - \frac{2 u[2,3]}{u[2]^2} \right) + 2 \cdot \frac{u[2,2] u[3,3] - u[2,3]^2}{u[2]^4} \\
 & \quad + 2 \cdot \frac{(u[2,3] u[2,2,3] - u[2,2] u[2,3,3])}{u[2]^3 u[2,2]} : \\
 & K4 := -\text{simplify} \left( \frac{1}{u_2^5 u_{2,2}^2} \left( u_{[1]} u_{2,2}^3 u_{2,3,3} - u_{[1]} u_{2,2}^2 u_{2,3} u_{2,2,3} + u_{2,2}^2 u_{2,2}^2 u_{2,3,3} - 2 \right. \right. \\
 & \quad u_{2,2}^2 u_{2,2} u_{2,3} u_{2,2,3} + u_{2,2}^2 u_{2,3}^2 u_{2,2,2} + u_{2,2} u_{2,2}^3 v_{2,3} - u_{2,2} u_{2,2}^2 u_{2,3}^2 - u_{2,2} u_{2,2}^2 u_{2,3} v_{2,2} \\
 & \quad + u_3 u_{2,2}^3 u_{2,3} + u_{2,2}^4 v_3 - u_{2,2}^3 u_{2,3} v_2 + u_{2,2}^3 u_{2,2,3} v_{[1]} - u_{2,2}^2 u_{2,3} u_{2,2,2} v_{[1]} + \\
 & \quad u_{2,2}^3 u_{1,2,3} + u_{2,2}^3 u_{3,3,3} - u_{2,2}^2 u_{2,3} u_{1,2,2} - 5 u_{2,2}^2 u_{2,3} u_{2,3,3} + 6 u_{2,2} u_{2,3}^2 u_{2,2,3} \\
 & \quad \left. \left. - 2 u_{2,3}^3 u_{2,2,2} \right) \right) :
 \end{aligned}$$

These four functions are differential invariants, which we may verify.

$$\begin{aligned}
 & > \text{simplify}(\text{map}(\text{LieDerivative}, \text{map}(\text{Prolong}, [Z1, Z2, Z3, Z4, Z5], 3), [K1, K2, K3, \\
 & \quad K4])) \\
 & \quad [0, 0, 0, 0], [0, 0, 0, 0], [0, 0, 0, 0], [0, 0, 0, 0], [0, 0, 0, 0] \quad (5.1.1)
 \end{aligned}$$

Using these, the commutation relations may be written in a simple form.

$$\begin{aligned}
 & > D1(D2(t)) - D2(D1(t)) + D2(t); \text{Pullback}(T3, \text{simplify}(D1(D2(x)) - D2(D1(x))) \\
 & \quad + D2(x)); \text{Pullback}(T3, \text{simplify}(D1(D2(y)) - D2(D1(y)) + D2(y))) \\
 & \quad 0 \\
 & \quad 0 \\
 & \quad 0 \quad (5.1.2)
 \end{aligned}$$

$$\begin{aligned}
 & > \text{simplify}(\text{Pullback}(T3, D1(D3(t)) - D3(D1(t)) - K1 D3(t) - (K1 - 2 K2) D2(t) \\
 & \quad + K3 D1(y))); \text{simplify}(\text{Pullback}(T3, D1(D3(x)) - D3(D1(x)) - K1 D3(x) \\
 & \quad - (K1 - 2 K2) D2(x) + K3 D1(x))); \text{simplify}(\text{Pullback}(T3, D1(D3(y)) \\
 & \quad - D3(D1(y)) - K1 D3(y) - (K1 - 2 K2) D2(y) + K3 D1(y))); \\
 & \quad 0 \\
 & \quad 0 \\
 & \quad 0 \quad (5.1.3)
 \end{aligned}$$

$$\begin{aligned}
 & > \text{simplify}(D2(D3(t)) - D3(D2(t)) - K2 D3(t) - K3 D2(t) - K4 D1(t)); \\
 & \quad \text{simplify}(\text{Pullback}(T3, D2(D3(x)) - D3(D2(x)) - K2 D3(x) - K3 D2(x) \\
 & \quad - K4 D1(x))); \text{simplify}(\text{Pullback}(T3, D2(D3(y)) - D3(D2(y)) - K2 D3(y) \\
 & \quad - K3 D2(y) - K4 D1(y))) \\
 & \quad 0 \\
 & \quad 0 \\
 & \quad 0 \quad (5.1.4)
 \end{aligned}$$

> We may rewrite K1,...,K4 in a better way. These are the expressions appearing in the paper.

$$\begin{aligned}
 & \text{> } L1 := D1(\log(u[2, 2])) - 3; L2 := D2(\log(u[2, 2])); \\
 & L3 := \text{simplify}\left(K2 \cdot \left(1 - \frac{2 u[2, 3]}{u[2]^2}\right) - \frac{2 \cdot u[2, 2]}{u[2]^3} (D2(u[3])) + 2 \frac{D2(u[2, 3])}{u[2]^2}\right); \\
 & L4 := \text{simplify}\left(\frac{1}{u[2]^4} \left(u[2, 2] D2(2 u[3, 3] - u[2] u[3]) - D2\left(\frac{u[2, 3]}{u[2, 2]}\right) u[2, \right. \right. \\
 & \quad \left. \left. 2\right] (2 u[2, 3] - u[2]^2) - D2(u[2, 3]^2)\right)\right); \\
 & \quad L1 := \frac{u_{2,2,2}}{u_{2,2}^2} - 3 \\
 & \quad L2 := -\frac{u_{2,2} u_{2,2,3} - u_{2,3} u_{2,2,2}}{u_{2,2}^2} \tag{5.1.5}
 \end{aligned}$$

$$\begin{aligned}
 & \text{> } K1 - L1; K2 - L2; \text{simplify}(K3 - L3); \text{simplify}(\text{Pullback}(T3, K4 - L4)) \\
 & \quad 0 \\
 & \quad 0 \\
 & \quad 0 \\
 & \quad 0 \tag{5.1.6}
 \end{aligned}$$

## Generating invariants of higher order

$$\begin{aligned}
 & \text{> } I11 := (\text{Pullback}(T3, D1(I1))) : I12 := (\text{Pullback}(T3, D2(I1))) : I13 \\
 & \quad := (\text{Pullback}(T3, D3(I1))) : \\
 & I21 := (\text{Pullback}(T3, D1(I2))) : I22 := (\text{Pullback}(T3, D2(I2))) : I23 \\
 & \quad := (\text{Pullback}(T3, D3(I2))) : \\
 & I31 := (\text{Pullback}(T3, D1(I3))) : I32 := (\text{Pullback}(T3, D2(I3))) : I33 \\
 & \quad := (\text{Pullback}(T3, D3(I3))) :
 \end{aligned}$$

We show that the third order invariants are generated by the three invariant derivations and the three second order invariants. The nine third order invariants are independent.

$$\begin{aligned}
 & \text{> } DGinfo(MM, \text{"FrameJetVariables"})[1..43] \\
 & \quad [t, x, y, u[], v[], u_1, u_2, u_3, v_1, v_2, v_3, u_{1,1}, u_{1,2}, u_{1,3}, u_{2,2}, u_{2,3}, u_{3,3}, v_{1,1}, v_{1,2}, v_{1,3}, v_{2,2}, \\
 & \quad v_{2,3}, v_{3,3}, u_{1,1,1}, u_{1,1,2}, u_{1,1,3}, u_{1,2,2}, u_{1,2,3}, u_{1,3,3}, u_{2,2,2}, u_{2,2,3}, u_{2,3,3}, u_{3,3,3}, \\
 & \quad v_{1,1,1}, v_{1,1,2}, v_{1,1,3}, v_{1,2,2}, v_{1,2,3}, v_{1,3,3}, v_{2,2,2}, v_{2,2,3}, v_{2,3,3}, v_{3,3,3}] \\
 & \text{> } \text{Rank}(\text{subs}(\text{seq}(\text{var3}[i] = \text{Generate}(\text{rational}), i = 1..nops(\text{var3})), \\
 & \quad [\text{seq}(\text{diff}(\text{Pullback}(T3, [I1, I2, I3, I11, I12, I13, I21, I22, I23, I31, I32, I33])), \\
 & \quad \text{var3}[i]), i = 1..nops(\text{var3}))]) \tag{5.2.2} \\
 & \quad 12
 \end{aligned}$$

We verify that they are invariant.

$$\begin{aligned}
 & \text{> } \text{simplify}(\text{Pullback}(T3, \text{map}(\text{LieDerivative}, \text{map}(\text{Prolong}, [X1, X2, X3, X4, X5], 3), \\
 & \quad [I1, I2, I3, I11, I12, I13, I21, I22, I23, I31, I32, I33]))) \\
 & \quad [[0, 0, 0, 0, 0, 0, 0, 0, 0, 0, 0, 0, 0], [0, 0, 0, 0, 0, 0, 0, 0, 0, 0, 0, 0, 0], [0, 0, 0, 0, 0, 0, 0, 0, 0, 0, 0, 0, 0], \\
 & \quad [0, 0, 0, 0, 0, 0, 0, 0, 0, 0, 0, 0, 0]] \tag{5.2.3} \\
 & \text{> } \text{var4} := DGinfo(MM, \text{"FrameJetVariables"})[1..73] \\
 & \text{> } \text{invar4} := [\text{op}([I1, I2, I3, I11, I12, I13, I21, I22, I23, I31, I32, I33]), \text{op}(\text{map}(D2, [I11,
 \end{aligned}$$

```

I12, I13, I21, I22, I23, I31, I32, I33]))), op(map(D1, [I11, I12, I13, I21, I22, I23,
I31, I32, I33])), op(map(D3, [I11, I12, I13, I21, I22, I23, I31, I32, I33]))):
> Rank(subs(seq(var4[i] = Generate(rational), i = 1..nops(var4)),
[seq(diff(Pullback(T4, invar4), var4[i]), i = 1..nops(var4))]))

```

By the way, we also have some simpler invariants of order 3

```

> [  $\frac{-u_{2,2} u_{2,2,3} + u_{2,3} u_{2,2,2}}{u_{2,2}^2}, \frac{u_{2,2} u_{2,2,2}}{u_{2,2}^2}, \frac{u_{2,2,3} + v_{2,2,2}}{u_{2,2} u_{2,2}}$  ]

```

## I2 and derivations generate all invariants

We show that I1 and I3 are combinations of K1,...,K4 and derivatives of I2.

```

> I2 :=  $\frac{u_{2,2}^2 u_{2,3} + u_{2,2} u_{2,2} v_2 + u_{2,2} u_{3,3} - u_{2,3}^2}{u_2^4} : K1 := \text{expand}\left(\frac{u_{2,2} u_{2,2,2}}{u_{2,2}^2} - 3\right) : K2 :=$ 
 $-\frac{u_{2,2} u_{2,2,3} - u_{2,3} u_{2,2,2}}{u_{2,2}^2} :$ 

```

```

K3 := K2 ·  $\left(1 - \frac{2 u[2,3]}{u[2]^2}\right) + 2 \cdot \frac{u[2,2] u[3,3] - u[2,3]^2}{u[2]^4}$ 
+ 2 ·  $\frac{(u[2,3] u[2,2,3] - u[2,2] u[2,3,3])}{u[2]^3 u[2,2]} :$ 

```

```

K4 := -simplify $\left(\frac{1}{u_{2,2}^5 u_{2,2}^2} \left(u_{[1]} u_{2,2}^3 u_{2,3,3} - u_{[1]} u_{2,2}^2 u_{2,3} u_{2,2,3} + u_{2,2}^2 u_{2,2}^2 u_{2,3,3} - 2\right.\right.$ 
 $u_{2,2}^2 u_{2,2} u_{2,3} u_{2,2,3} + u_{2,2}^2 u_{2,3}^2 u_{2,2,2} + u_{2,2} u_{2,2}^3 v_{2,3} - u_{2,2} u_{2,2}^2 u_{2,3}^2 - u_{2,2} u_{2,2}^2 u_{2,3} v_{2,2}$ 
 $+ u_{2,3} u_{2,2}^3 u_{2,3} + u_{2,2}^4 v_3 - u_{2,2}^3 u_{2,3} v_2 + u_{2,2}^3 u_{2,2,3} v_{[1]} - u_{2,2}^2 u_{2,3} u_{2,2,2} v_{[1]} +$ 
 $u_{2,2}^3 u_{1,2,3} + u_{2,2}^3 u_{3,3,3} - u_{2,2}^2 u_{2,3} u_{1,2,2} - 5 u_{2,2}^2 u_{2,3} u_{2,3,3} + 6 u_{2,2} u_{2,3}^2 u_{2,2,3}$ 
 $\left. - 2 u_{2,3}^3 u_{2,2,2}\right) :$ 

```

```

> D1 := proc (funct)

```

```

simplify $\left(\frac{u_2}{u_{2,2}} \text{TotalDiff}(funct, x)\right);$ 

```

```

end proc:

```

```

D2 := proc (funct)

```

```

simplify $\left(\frac{u_{2,3}}{u_{2,2} u_{2,2}} \text{TotalDiff}(funct, x) - \frac{1}{u_2} \text{TotalDiff}(funct, y)\right);$ 

```

```

end proc:

```

```

D3 := proc (funct)

```

```

simplify $\left(\frac{1}{u[2]^3} \left(u[2,2] \text{TotalDiff}(funct, t) + (v_{[1]} u_{2,2} + v_2 u_2 + u[3,$ 
 $3]) \text{TotalDiff}(funct, x) + (u_{[1]} u_{2,2} + u_2^2 - 2 u_{2,3}) \text{TotalDiff}(funct, y)\right)\right);$ 

```

```

end proc:

```

```

>

```

```

> B := Pullback(T2, I2) :

```

```

> for i from 1 to 3 do

```

```

B[i] := Pullback(T3, D[i](B));

```

```

od:
> for j from 1 to 3 do
  for k from 1 to 3 do
    B||k||j := Pullback(T4, D||j(D||k(B)) );
  od:od:

```

We have the following relations.

$$\text{> simplify}\left(\text{Pullback}\left(T3, -B K1 + B1 + \frac{K2}{2} + \frac{K3}{2}\right) - I1\right) \quad (5.3.1)$$

0

$$\text{> simplify}\left(\text{Pullback}\left(T3, -B K1 + K2 B - B + B1 - B2 + \frac{1}{4} K2 + \frac{3}{4} K3 + \frac{1}{2} K4\right) - I3\right) \quad (5.3.2)$$

0

```

>

```

### How we found the relations

```

[> var3 := DGinfo(MM, "FrameJetVariables")[1..43]
> invar3 := Pullback(T4, [B, B1, B2, B3, K1, K2, K3, K4]) :
> Rank(subs(seq(var3[i] = Generate(rational), i = 1..nops(var3)),
  [seq(diff(invar3, var3[i]), i = 1..nops(var3))]))

```

8

(5.3.1.1)

```

> pt := {seq(var3[i] = Generate(rational), i = 1..nops(var3))} :
> lineq := [seq(add(eval(diff(invar3[i], var3[j]), pt) * w[var3[j]], j = 1
  ..nops(var3)), i = 1..nops(invar3))] :
> sol := [op(eliminate(lineq, [seq(w[var3[i]], i = 24..nops(var3))][2]))] :
  nops(%)

```

3

(5.3.1.2)

```

> Rank([seq(diff(sol, w[var3[i]]), i = 1..nops(var3))]

```

3

(5.3.1.3)

```

> sol := eliminate(Pullback(T4, [B - b, B1 - b1, B2 - b2, B3 - b3, K1 - k1, K2
  - k2, K3 - k3, K4 - k4]), var3[24..43])[2] :
> factor(simplify(eliminate(sol union {I1 - i1, I3 - i3, B - b}, {u[2, 3], v[2, 2],
  u[2, 2]}))[2]))

```

$$\left\{ -\left(u_2 v_2 - v_{2,3}\right)^2 (2 b k1 - 2 b1 + 2 i1 - k2 - k3), -\left(u_2 v_2 - v_{2,3}\right)^2 (4 b k2 - 4 b - 4 b2 + 4 i1 - 4 i3 - k2 + k3 + 2 k4) \right\} \quad (5.3.1.4)$$

```

> solve({(4 b k2 - 4 b - 4 b2 + 4 i1 - 4 i3 - k2 + k3 + 2 k4), (2 b k1 - 2 b1
  + 2 i1 - k2 - k3)}, {i1, i3})

```

$$\left\{ i1 = -b k1 + b1 + \frac{1}{2} k2 + \frac{1}{2} k3, i3 = -b k1 + k2 b - b + b1 - b2 + \frac{1}{4} k2 + \frac{3}{4} k3 + \frac{1}{2} k4 \right\} \quad (5.3.1.5)$$

```

>

```

## 3.3 EW-structure written in invariant coframe

We find the coframe dual to our set of derivations

```

> B := MatrixInverse(Matrix([map(D1, [t, x, y]), map(D2, [t, x, y]), map(D3, [t, x, y])]))

```

$$B := \left[ \begin{array}{c} \left[ -\frac{u_{[]} u_{2,2} u_{2,3} + u_2^2 u_{2,3} + u_2 u_{2,2} v_2 + u_{2,2}^2 v_{[]} + u_{2,2} u_{3,3} - 2 u_{2,3}^2}{u_2 u_{2,2}}, \right. \\ \left. \frac{u_2 (u_{[]} u_{2,2} + u_2^2 - 2 u_{2,3})}{u_{2,2}}, \frac{u_2^3}{u_{2,2}} \right], \\ \left[ \frac{u_{2,2}}{u_2}, 0, 0 \right], \\ \left[ \frac{u_{2,3}}{u_2}, -u_2, 0 \right] \end{array} \right] \quad (6.1)$$

$$\begin{aligned} &> \text{alpha}[1] := B[1, 1] dt + B[2, 1] dx + B[3, 1] dy; \text{alpha}[2] := B[1, 2] dt + B[2, 2] dx \\ &\quad + B[3, 2] dy; \text{alpha}[3] := B[1, 3] dt + B[2, 3] dx + B[3, 3] dy; \\ \alpha_1 &:= -\frac{dt (u_{[]} u_{2,2} u_{2,3} + u_2^2 u_{2,3} + u_2 u_{2,2} v_2 + u_{2,2}^2 v_{[]} + u_{2,2} u_{3,3} - 2 u_{2,3}^2)}{u_2 u_{2,2}} \\ &\quad + \frac{dx u_{2,2}}{u_2} + \frac{dy u_{2,3}}{u_2} \\ \alpha_2 &:= \frac{dt u_2 (u_{[]} u_{2,2} + u_2^2 - 2 u_{2,3})}{u_{2,2}} - dy u_2 \\ \alpha_3 &:= \frac{dt u_2^3}{u_{2,2}} \end{aligned} \quad (6.2)$$

We check that this is correct.

$$\begin{aligned} &> V3 := D3(x) D_{_x} + D3(t) D_{_t} + D3(y) D_{_y}; V2 := D2(x) D_{_x} + D2(t) D_{_t} \\ &\quad + D2(y) D_{_y}; V1 := D1(x) D_{_x} + D1(t) D_{_t} + D1(y) D_{_y}; \\ &> \text{Hook}(D1(x) D_{_x}, \text{alpha}[1]); \text{Hook}(D1(x) D_{_x}, \text{alpha}[2]); \text{Hook}(D1(x) D_{_x}, \text{alpha}[3]); \\ &\quad 1 \\ &\quad 0 \\ &\quad 0 \end{aligned} \quad (6.3)$$

$$\begin{aligned} &> \text{Hook}(D2(x) D_{_x} + D2(t) D_{_t} + D2(y) D_{_y}, \text{alpha}[1]); \text{Hook}(D2(x) D_{_x} + D2(t) D_{_t} \\ &\quad + D2(y) D_{_y}, \text{alpha}[2]); \text{Hook}(D2(x) D_{_x} + D2(t) D_{_t} + D2(y) D_{_y}, \text{alpha}[3]); \\ &\quad 0 \\ &\quad 1 \\ &\quad 0 \end{aligned} \quad (6.4)$$

$$\begin{aligned} &> \text{Pullback}(T2, \text{Hook}(D3(x) D_{_x} + D3(t) D_{_t} + D3(y) D_{_y}, \text{alpha}[1])); \text{Hook}(D3(x) D_{_x} \\ &\quad + D3(t) D_{_t} + D3(y) D_{_y}, \text{alpha}[2]); \text{Hook}(D3(x) D_{_x} + D3(t) D_{_t} + D3(y) D_{_y}, \\ &\quad \text{alpha}[3]); \\ &\quad 0 \\ &\quad 0 \\ &\quad 1 \end{aligned} \quad (6.5)$$

Where are they independent?

$$\begin{aligned} &> \text{evalDG}(\text{alpha}[1] \&w \text{alpha}[2] \&w \text{alpha}[3]) \\ &\quad - \left( \left( (u_2^3 dt) \wedge dx \right) \wedge dy \right) \end{aligned} \quad (6.6)$$

We rewrite our metric and one-form in terms of the coframe, as described in the paper.

$$\begin{aligned} &> g := \text{evalDG}(4 dt \&s dx + 2 u_{[]} dt \&s dy - (u_{[]}^2 + 4 v_{[]}) dt \&t dt - dy \&t dy); \end{aligned} \quad (6.7)$$



$$g := - \left( \left( (u_{[1]}^2 + 4 v_{[1]}) dt \right) dt \right) + (2 dt) dx + (u_{[1]} dt) dy + (2 dx) dt + (u_{[1]} dy) dt - (dy dy) \quad (6.7)$$

$$\begin{aligned} > \text{omega} := \text{evalDG}((u_{[1]} u_{[2]} + 2 u_{[3]} + 4 v_{[2]}) dt - u_{[2]} dy); \\ & \quad \omega := (u_{[1]} u_2 + 2 u_3 + 4 v_2) dt - (u_2 dy) \end{aligned} \quad (6.8)$$

$$\begin{aligned} > \text{scalingfactor} := u_{[2]}^2 \\ & \quad \text{scalingfactor} := u_2^2 \end{aligned} \quad (6.9)$$

$$\begin{aligned} > G := \text{simplify}(\text{scalingfactor Matrix}([[\text{Hook}([V1, V1], g), \text{Hook}([V1, V2], g), \\ & \quad \text{Hook}([V1, V3], g)], [\text{Hook}([V2, V1], g), \text{Hook}([V2, V2], g), \text{Hook}([V2, V3], g)], \\ & \quad [\text{Hook}([V3, V1], g), \text{Hook}([V3, V2], g), \text{Hook}([V3, V3], g)])) \\ & \quad G := \begin{bmatrix} 0 & 0 & 2 \\ 0 & -1 & 1 \\ 2 & 1 & -\frac{u_2^4 - 4 u_2^2 u_{2,3} - 4 u_2 u_{2,2} v_2 - 4 u_{2,2} u_{3,3} + 4 u_{2,3}^2}{u_2^4} \end{bmatrix} \end{aligned} \quad (6.10)$$

$$\begin{aligned} > \text{simplify}(\text{Pullback}(T2, G[3, 3] - (4 I2 - 1))) \\ & \quad 0 \end{aligned} \quad (6.11)$$

$$\begin{aligned} > \text{Hook}(V1, \text{omega}) + 2 D1(\log(u_{[2]})) - 2; \text{Hook}(V2, \text{omega}) + 2 D2(\log(u_{[2]})) - 1; \\ & \quad \text{simplify}(\text{Pullback}(T2, \text{Hook}(V3, \text{omega}) + 2 D3(\log(u_{[2]})) - (4 I2 - 1))) \\ & \quad 0 \\ & \quad 0 \\ & \quad 0 \end{aligned} \quad (6.12)$$

### 3.4 The equivalence problem

#### The differential syzygies of order 4

$$\begin{aligned} > I1 := \frac{u_{2,3} + v_{2,2}}{u_2^2} : I2 := \frac{u_2^2 u_{2,3} + u_2 u_{2,2} v_2 + u_{2,2} u_{3,3} - u_{2,3}^2}{u_2^4} : I3 \\ & \quad := \frac{u_2^2 v_{2,2} - u_2 u_{2,2} v_2 + u_{2,2} v_{2,3} - u_{2,3} v_{2,2}}{u_2^4} : K1 := \text{expand}\left(\frac{u_2 u_{2,2,2}}{u_{2,2}^2} - 3\right) : \\ & \quad K2 := -\frac{u_{2,2} u_{2,2,3} - u_{2,3} u_{2,2,2}}{u_2 u_{2,2}^2} : \\ & \quad K3 := K2 \cdot \left(1 - \frac{2 u_{[2,3]}}{u_{[2]}^2}\right) + 2 \cdot \frac{u_{[2,2]} u_{[3,3]} - u_{[2,3]}^2}{u_{[2]}^4} \\ & \quad + 2 \cdot \frac{(u_{[2,3]} u_{[2,2,3]} - u_{[2,2]} u_{[2,3,3]})}{u_{[2]}^3 u_{[2,2]}} : \\ & \quad K4 := -\text{simplify}\left(\frac{1}{u_2^5 u_{2,2}^2} (u_{[1]} u_{2,2}^3 u_{2,3,3} - u_{[1]} u_{2,2}^2 u_{2,3} u_{2,2,3} + u_2^2 u_{2,2}^2 u_{2,3,3} - 2 \right. \\ & \quad u_2^2 u_{2,2} u_{2,3} u_{2,2,3} + u_2^2 u_{2,3}^2 u_{2,2,2} + u_2 u_{2,2}^3 v_{2,3} - u_2 u_{2,2}^2 u_{2,3}^2 - u_2 u_{2,2}^2 u_{2,3} v_{2,2} \\ & \quad \left. + u_3 u_{2,2}^3 u_{2,3} + u_{2,2}^4 v_3 - u_{2,2}^3 u_{2,3} v_2 + u_{2,2}^3 u_{2,2,3} v_{[1]} - u_{2,2}^2 u_{2,3} u_{2,2,2} v_{[1]} + \right. \end{aligned}$$

$$u_{2,2}^3 u_{1,2,3} + u_{2,2}^3 u_{3,3,3} - u_{2,2}^2 u_{2,3} u_{1,2,2} - 5 u_{2,2}^2 u_{2,3} u_{2,3,3} + 6 u_{2,2} u_{2,3}^2 u_{2,2,3} - 2 u_{2,3}^3 u_{2,2,2}) : \\$$

> D1 := **proc**( *funct* )

*simplify*  $\left( \frac{u_2}{u_{2,2}} \text{TotalDiff}( \text{funct}, x ) \right);$

**end proc**:

D2 := **proc**( *funct* )

*simplify*  $\left( \frac{u_{2,3}}{u_2 u_{2,2}} \text{TotalDiff}( \text{funct}, x ) - \frac{1}{u_2} \text{TotalDiff}( \text{funct}, y ) \right);$

**end proc**:

D3 := **proc**( *funct* )

*simplify*  $\left( \frac{1}{u[2]^3} \left( u[2,2] \text{TotalDiff}( \text{funct}, t ) + (v[1] u_{2,2} + v_2 u_2 + u[3,3]) \text{TotalDiff}( \text{funct}, x ) + (u[1] u_{2,2} + u_2^2 - 2 u_{2,3}) \text{TotalDiff}( \text{funct}, y ) \right) \right);$

**end proc**:

We compute syzygies. The computation is a little time-consuming (around one hour), so if you just want to see the syzygies they are made available in a subsection. In these computations we have taken double derivatives in both ways, meaning that the commutation relations of the derivations appear as syzygies.

> A := *Pullback*(T2, I1) : B := *Pullback*(T2, I2) : C := *Pullback*(T2, I3) :

> **for** i **from** 1 **to** 3 **do**

A || i := *Pullback*(T3, D || i(A)); B || i := *Pullback*(T3, D || i(B)); C || i := *Pullback*(T3, D || i(C));

**od**:

> **for** j **from** 1 **to** 3 **do**

**for** k **from** 1 **to** 3 **do**

A || k || j := *Pullback*(T4, D || j(D || k(A))); B || k || j := *Pullback*(T4, D || j(D || k(B))); C || k || j := *Pullback*(T4, D || j(D || k(C)));

**od:od**:

>

> eq1 := *eliminate*( { *seq*(*seq*(A || k || j - a || k || j, k = 1 .. 3), j = 1 .. 3), *seq*(*seq*(B || k || j - b || k || j, k = 1 .. 3), j = 1 .. 3), *seq*(*seq*(C || k || j - c || k || j, k = 1 .. 3), j = 1 .. 3) }, { u[1,1,1,1], u[1,1,1,2], u[1,1,1,3], u[1,1,2,2], u[1,1,2,3], u[1,2,2,2], u[1,2,2,3], u[2,2,2,2], u[2,2,2,3], v[1,1,1,1], v[1,1,1,2], v[1,1,1,3], v[1,1,2,2], v[1,1,2,3], v[1,2,2,2], v[1,2,2,3], v[2,2,2,2], v[2,2,2,3] } ) [2] :

> *nops*(*invariants4*); *nops*(eq1); *nops*( { u[1,1,1,1], u[1,1,1,2], u[1,1,1,3], u[1,1,2,2], u[1,1,2,3], u[1,2,2,2], u[1,2,2,3], u[2,2,2,2], u[2,2,2,3], v[1,1,1,1], v[1,1,1,2], v[1,1,1,3], v[1,1,2,2], v[1,1,2,3], v[1,2,2,2], v[1,2,2,3], v[2,2,2,2], v[2,2,2,3] } );

27

14

18

(7.1.1)

> *fourjets* := { *seq*(*seq*(*seq*(*seq*(op([u[i1,i2,i3,i4], v[i1,i2,i3,i4]]), i4 = i3 .. 3), i3 = i2 .. 3), i2 = i1 .. 3), i1 = 1 .. 3) } : *nops*(%)

30

(7.1.2)

> *tmpp* := { } : **for** j **to** *nops*(eq1) **do** **for** i **to** *nops*(*fourjets*) **do** *tmpp* := *tmpp* **union** { *diff*(eq1[j], *fourjets*[i]) } : **od:od**: *tmpp*

{0}

(7.1.3)

```

> eq2 := eliminate( {op(simplify(eq1)), seq(A||i - a||i, i = 1 ..3), seq(B||i - b||i, i = 1
..3), seq(C||i - c||i, i = 1 ..3)}, {u[1, 1, 1], u[1, 1, 2], u[1, 1, 3], u[1, 2, 2], u[1,
2, 3], u[2, 2, 2], u[2, 2, 3], v[1, 1, 1], v[1, 1, 2], v[1, 1, 3], v[1, 2, 2], v[1, 2, 3],
v[2, 2, 2], v[2, 2, 3]})[2]:
> smpleq2 := simplify(eq2) :
> threejets := {seq(seq(seq(op([u[i1, i2, i3], v[i1, i2, i3]]), i3 = i2 ..3), i2 = i1 ..3), i1
= 1 ..3)) : nops(%)}
20 (7.1.4)
> tmpp := { } :for j to nops(eq2) do for i to nops(threejets) do tmpp := tmpp
union {diff(eq2[j], threejets[i])} :od:od: tmpp
{0} (7.1.5)
> smpleq2[1]
a12 - a2 - a21 (7.1.6)
> eq3 := eliminate( {op(smpleq2), A - a, B - b, C - c}, {u[1, 1], u[1, 2], u[1, 3],
u[2, 2], u[2, 3], v[1, 1], v[1, 2], v[1, 3], v[2, 2], v[2, 3]})[2]:
> simplify(eq3[1])
a12 - a2 - a21 (7.1.7)
> nops(simplify(eq3))
14 (7.1.8)
> twojets := {seq(seq(seq(op([u[i1, i2], v[i1, i2]]), i2 = i1 ..3), i1 = 1 ..3)) : nops(%)}
12 (7.1.9)
> tmpp := { } :for j to nops(eq3) do for i to nops(twojets) do tmpp := tmpp
union {diff(eq3[j], twojets[i])} :od:od: tmpp
{0} (7.1.10)

```

## Results

```

> eq3
{a12 - a2 - a21, b12 - b2 - b21, c12 - c2 - c21, -a3 a3 - a32 a + a3 a2 (7.1.1.1)
+ b1 a3 - a2 a2 + a2 a1 - c22 a + b22 a2 - c22 a2 - b2 a3 + c1 a4 - c2 a4
+ b2 a5 + a2 c2 - a2 c1 - 2 b3 a3 + 2 b3 a2 + a2 a3 - a1 b c c1 - 5 c4
- 2 a a3 b1 c + a b1 b2 c - 2 a a1 b1 c + 3 a a2 b1 c - a3 a1 + 2 a b1 c c1
- 2 a b1 c c2 - a b1 c c3 + 5 a2 b b1 c1 - 5 a2 b b2 c1 - 4 a a1 b2 c1
- 4 a a1 b2 c2 + 4 a a2 b2 c1 + 6 a b2 c c1 - a a2 b c1 - 4 a a2 b c2
+ a a2 b c3 - 3 a a3 b c1 + 7 a a3 b c2 + a b b1 c1 - a b b1 c2
- 3 a b b2 c1 + 4 a b b2 c2 + 2 a b c c3 - 4 a b c1 c2 + a b c1 c3
- 2 a1 b c c2 - a1 b c c3 + 2 a2 b c c1 - a3 b c c1 - b b1 c c1
- 2 b b2 c c1 + 2 a a1 a2 b c + 2 a a1 a3 b c - 2 a a1 b c c1
- 2 a a2 b b1 c - 3 a2 a1 b b1 c + a2 b c c11 + 4 a2 b c c2 + a a12 b c
- 3 a a1 a3 b2 - a a1 b2 b2 - 4 a a1 b c2 + a a1 b1 c2 - 2 a a22 b c
- a a2 b2 b1 - 2 a a2 b c2 + a a13 b c + 2 a a2 b b3 - 2 a a23 b c
+ 3 a a3 b b2 + 2 a b b3 c1 - 2 b b2 c + 2 a a2 c - a2 a3 b - a2 b b2
- 2 a2 b c - 3 a2 b b1 - a2 b b2 - 14 a2 b c - a2 b c12 + a2 b c22
+ 3 a b2 b1 + a b2 b2 + 18 a b2 c + a b b2 + 4 a b c - a2 b1 b2 - a2 b c2
+ 2 a3 b c + a2 a2 b - a2 a3 b + 4 a a1 b2 - a a2 b2 - a1 b2 c1 + 3 a1 b c2

```

$$\begin{aligned}
& + 8a^2al b^2 - 2a^2al b + al a3 b + 2a a3 b^2 - al a3 b^2 + a2^2 b c \\
& - 6a2 b^2 c - 9a2 b c^2 + a b2 c + al b2 c + al c c2 - a2 a3 c - a2 b2 c \\
& - 4a^2 a2 c + 4a^2 a3 c + al b1 c^2 - a al a3 - a^2 a2 b1 + 7a a2 c^2 \\
& - 2a^3 al c - 5a al c^2 - a al b2 + a^2 al b1 + 5a al b c2 + 6a a2 b c \\
& + al b b1 c - 3a a2 a3 b + 2a a2 b b1 - 3a a2 b b2 + 3a^2 al b c \\
& + 2a^2 a2 b b1 + 6a^2 b b1 c - 4a^2 al b b1 + 4a al a3 b - a al b b1 \\
& + 3a al b b2 - a al b c + a al b c1 - a a3 b b1 + 6a b b1 c + 6a b b2 c \\
& - a a3 b c - al a2 b c - al a3 b c + al b b2 c - a2 b b1 c - 5a al b^2 c \\
& - a al b b3 - b^3 + 4a al b b1 c + a^3 c^2 + 2a^3 c + 2a c^2 + al c^2 + 2al c^3 \\
& - 9a^2 c^2 - a al b2 c + 2a^2 al b b2 - 3a^2 b b11 c + a b b1 b2 \\
& - 2a b b12 c + b c2 c3 - 9a^2 b^2 c1 + 10a^2 b^2 c2 + 5a b^3 c1 + 4a b^2 c1^2 \\
& + 3a^2 b c1 - 4a^2 b c2 - a^2 b c23 - 2a^2 b c3 - 4a b^2 c1 + a b^2 c2 \\
& + 2a b^2 c3 - a b c1^2 + 4a b c2^2 - 2al b^2 c2 - al b^2 c3 + 2a2 b^2 c1 \\
& - a3 b^2 c1 + 4b^2 c c2 - 3b c^2 c1 + 2b c^2 c2 + b c c1^2 + a^2 c c3 + 4a c^2 c1 \\
& - a c^2 c2 - b1 c^2 c1 + b1 c^2 c2 - 2b2 c^2 c1 + a c c23 + a3 c c3 - b2 c c1 \\
& + b2 c c2 + b2 c c3 - c c1 c2 + c c2 c3 - a3 c c1 + 2a3 c c2 - 2a^2 c c1 \\
& - a^2 b1 c1 - a a3 c3 + 2a b c1 - a b c2 + a b c23 - a b c3 - a b2 c3 \\
& + 2a c c1 - a c c2 - a c c3 - a c2 c3 - a3 b c1 + 2a3 b c2 + a3 b c3 \\
& - b b2 c1 + b b2 c2 + b b2 c3 - 2b c c1 - 2b c c23 - b c1 c2 + 4a^2 al c \\
& + 2al b2 c^2 - a2 b1 c^2 + al a3 c + a3 b2 c + 3a b1 c^2 + 5a b2 c^2 \\
& - 3a^2 b1 c - a^3 b1 c - a^2 b1^2 c - 2a a3 c - 2a^3 b1 b2 + 10a^3 b c \\
& + 2a^3 b c1 + 4a^2 b^2 b1 - 12a^2 b^2 c + a^2 b^2 c11 + a^3 a2 b + al^2 b^2 c \\
& + 27a b c^2 - al b^2 b2 - 3b^2 b1 c + a3 b b2 - 2a al b + 2a a2 b \\
& + al b b2 + 2al b c + al b c2 + a^2 c^2 c1 + 5a^2 al c^2 + 2a a3 c c2 \\
& - 2a b1 b3 c + 2a b2 c c2 + a a2 b1 c^2 - 2a b1 c^2 c1 - 2a c c1 c2 \\
& - a al b3 c - a a2 a3 c - 2a a2 c c2 - a a3 c c1 - a^2 a2 b2 c - a^2 b1 c c2 \\
& - a^2 b2 c c1 - a al b2 c^2 + a^2 a3 b1 c + 3a^2 b1 c c1 + a al c c2 \\
& + a a2 c c1 - a^2 al b1 c + 2a^2 al b2 c - a al a2 c + 2a b c c1^2 \\
& - al b b1 c^2 + 3a^2 b b12 c - 8a^2 b b2 c - 3a^2 b c c1 + a^2 al a2 b \\
& - a^2 al a3 b + a^2 al b b3 - 2a^2 al b c2 + 2a^2 a2 a3 b - a^4 c - 5a b^2 b1 c \\
& + a b^2 b11 c - 2a b^2 c c11 - 4a b b1 c^2 - a^2 a2 b b2 - 6a^2 a2 b c \\
& - 2a^2 a2 b c1 + 4a^2 a2 b c2 - 2a^2 a3 b c1 - a^2 b b1 b2 - 2a^3 al b b2 \\
& - a^3 al b c + a^3 b b1 c + a^3 b b1 c1 + a^3 b b11 c + 4a^2 al b^2 c \\
& + 4a^2 al b^2 c1 - 2a al^2 b^2 c + 2a^3 al b b1 + 2a b c c12 - 2a b c c22 \\
& - a2 a3 b c - 2a2 b b2 c + a3 b b1 c - 2b b1 b2 c + 2a b b11 c^2 \\
& + a b c^2 c1 - a b c^2 c11 - c3 a^3 + b^3 c1 + 2b^3 c2 + b^2 c1^2 + c3 a^2 - b^2 c1 \\
& - b^2 c23 + b c2^2 - 2c^3 c1 - c^2 c1 - c^2 c23 + c c2^2 - 4a b b1 c c1 \\
& + 12a c^3 + a^2 b1 c3 + a^2 c c2 - a2 c c2 - 2a al c - 2a^3 c c1 - a^2 c
\end{aligned}$$

$$\begin{aligned}
& + a^3 b l^2 + a^3^2 b - b^2 b_2 - 3 b^2 c - 3 b c^2 + 4 a^3 b^2 - 5 a^2 b^2 + 3 a b^3 \\
& - 8 b^3 c - 18 b^2 c^2 - 16 b c^3 + 2 a b^2 - a l b^3 + a l b^2 - a_2 b^2 + a_3 b^2 \\
& + a^3^2 c - a_2 c^2 + a_3 c^2 - b l c^3 - b_2 c^2 - a a l c_2 - c_2 a_3 a^2 + c l b_2 a^2 \\
& + c_2 c l a^2 + a_3 a_2 a + b_2 a_2 a + c_2 a_2 a - b_2 a_3 a + c l a_3 a - 2 c_2 a_3 a \\
& + b_2 a_3 a^2 + c l b_2 a - c_2 b_2 a + c_2 c l a + c l a_3 a^2 - 2 c_2 b_3 a \\
& - 2 b_3 a_3 a - 2 b_3 b_2 a + a l_3 b^3 + a^5 b - a^4 b^2 + 4 a^3 b^3 + b^3 b l_2 \\
& - a_3 b^2 - b^2 b_3_2 + 4 a b^4 - 2 a l b^4 - a^5 b l - 4 a_2 c^3 + b l_2 c^3 - 4 b_2 c^3 \\
& - a_3 c^2 - b_3_2 c^2 + a^3 b_2^2 + a^4 b l^2 - 6 a^2 b c^2 - a^2 b c l^2 + 2 a a_2 b^3 \\
& - 2 a b^3 b l + 8 a b^3 c - a b^3 c l_1 + 2 a_3 b b_3 - 2 a_3 b c + 2 b b_2 b_3 \\
& + 2 b b_3 c_2 - 2 b b_3_2 c + a a_3 b + 2 a l_3 b^2 c + a l_3 b c^2 - a_2 a_3 b^2 \\
& - a_3 b^2 b l - b^2 b l b_2 - b^2 b l c_2 + 3 b^2 b l_2 c - 4 b^2 b_2 c + 3 b b l_2 c^2 \\
& - 8 b b_2 c^2 + 3 a a_3^2 b + 2 a b^2 b_3 + a b^2 c l_2 - a b^2 c_2_2 - a l b^2 b_3 \\
& - a^2 a_3 b - a^2 b b_3_2 + 4 a b^2 c^2 + a l b^3 b l - 4 a l b^3 c - 2 a l b^2 c^2 \\
& + a^2 a l_3 b^2 - a^2 a_2^2 b + 6 a^2 a_3 b^2 + 2 a^2 b^2 b l_2 - 2 a^2 b^2 b_2 + a c^2 c l_2 \\
& - a c^2 c_2_2 + 2 a c c_2^2 + a l b_3 c^2 - 2 a_2 b_2 c^2 + 2 a_3 b l c^2 - b l b_2 c^2 \\
& + a a_3 c + a b_3_2 c + a^2 b l_2 c^2 - 2 a^2 b_2 c^2 + a^3 a_3 b_2 + a^3 b_2 c_2 \\
& - a^4 b l b_2 - a a_2 b^2 + a^3 a l_3 b - a^3 a_2 b + 6 a^3 b b_2 - 2 a^3 b b_3 \\
& + a^3 b c l_2 - a^3 b c_2 - a^3 b c_2_2 - 2 a^3 a l b^2 + 2 a^3 a_2 b^2 - 3 a^3 b^2 c l \\
& - a^3 b^2 c l_1 - a^2 a l^2 b^2 - 2 a^2 a l b^3 + a^4 a l b - a^4 a_2 b - a^4 b b l \\
& - a^4 b b l_1 + a^4 b b l_2 - a^4 b c l + a b b_3_2 - a^2 c c l_2 + a^2 c c_2_2 + a a_2^2 c \\
& + 2 a^3 a_2 c + 3 a^3 b_2 c - 3 a^2 a_2 c^2 + a^4 b l c + a a l_3 c^2 - a a_2 b c^2 \\
& - 3 a a_3 c^2 - 2 a b_3 c^2 + 2 a_3 b_3 c + 2 b_2 b_3 c + 2 b_3 c c_2 - 3 a a l c^3 \\
& - a b l c^3 + a b l_1 c^3 - a^3 b l^2 c + a^3 b l_1 c - a^3 b l_2 c + 2 a^2 b l c^2 \\
& - 2 a^2 b l_1 c^2 + 2 a^3 c c_2 - a^3 b l c l - a^3 a_3 b l - a^2 a l_3 c + a^2 a_2 b c \\
& + 4 a^2 b_3 c - b^4 - a^2 b b_3 - a^2 b^2 b l_1 + 2 a^2 b l b_3 + 2 b b_3 c - 3 a b b_3 \\
& - 3 a b_3 c + b^2 b_3 + b_3 c^2 - 6 a^2 b^3 - b^3 b l + a l^2 b^3 + a^2 b^2 - a_2 b^3 \\
& + 3 a^3 b - a^2 b - 3 a^4 b - 3 b b l c^2 - a b^2 b l_2 + a^2 a_2 b - a l a_2 b^2 \\
& - 8 a^2 a_2 b^2 - 4 a a l b^3 - 2 a^3 b b l + a^3 b b l_1 - a^3 b b l_2 - 2 a a_3 b \\
& - a^2 a l_3 b - a b l_2 c^2 - c^3, -a_3 a^3 - a^3^2 a + a_3 a^2 - b l a^2 + 2 b l a^3 \\
& - a^2 a_2 + a^2 a l - b_2^2 a - c_2^2 a + b_2^2 a^2 - c_2^2 a^2 + b_2 a^2 - 2 b_2 a^3 \\
& + c l a^4 - c_2 a^4 + b_2 a^5 + a^2 c_2 - a^2 c l + b l a_3 a - b_3 a^3 + b_3 a^2 + a_2 a^3 \\
& - a l b c c l - 5 c^4 - b_2 b_3 c^2 - 2 a a_3 b l c - 2 a a l b l c + 3 a a_2 b l c \\
& - a^3 a l + 2 a b l c c l - 2 a b l c c_2 - a b l c c_3 + 5 a^2 b b l c l \\
& - 5 a^2 b b_2 c l - 4 a a l b^2 c l - 4 a a l b^2 c_2 + 4 a a_2 b^2 c l + 6 a b^2 c c l \\
& - a a_2 b c l - 4 a a_2 b c_2 + a a_2 b c_3 - 3 a a_3 b c l + 7 a a_3 b c_2 \\
& - 4 a b b l c_2 - 2 a b b_2 c l + 6 a b b_2 c_2 + 2 a b c c_3 - 4 a b c l c_2 \\
& + a b c l c_3 - 2 a l b c c_2 - a l b c c_3 + 2 a_2 b c c l - a_3 b c c l \\
& + 2 b b l c c_2 - 4 b b_2 c c l + 2 a a l a_2 b c + 2 a a l a_3 b c - 2 a a l b c c l
\end{aligned}$$

$$\begin{aligned}
& -2 a a_2 b b_1 c - 3 a^2 a_1 b b_1 c - 2 b^3 b_2 - b^2 b_{23} + a^2 b c c_{11} \\
& + 4 a^2 b c c_2 + a a_1^2 b c - 3 a a_1 a_3 b^2 - 3 a a_1 b^2 b_2 - 4 a a_1 b c^2 \\
& + a a_1 b_1 c^2 - 2 a a_2^2 b c + a a_2 b^2 b_1 - 2 a a_2 b c^2 + a a_{13} b c \\
& + a a_2 b b_3 - 2 a a_{23} b c + 5 a a_3 b b_2 + a b b_3 c_1 - b b_1 c_2 + 2 a a_2 c \\
& + 2 a b_1 c - a_2 a_3 b - a_2 b b_2 - 2 a_2 b c - 2 a^2 b b_1 - 2 a^2 b b_2 \\
& - 14 a^2 b c - a^2 b c_{12} + a^2 b c_{22} + 5 a b^2 b_2 + 18 a b^2 c + 2 a b b_1 \\
& - a b b_2 + 4 a b c - a_2 b c_2 + 2 a_3 b c + a^2 a_2 b - a^2 a_3 b + 4 a a_1 b^2 \\
& - a a_2 b^2 - a_1 b^2 c_1 + 3 a_1 b c^2 + 8 a^2 a_1 b^2 - 2 a^2 a_1 b + a_1 a_3 b \\
& + 2 a a_3 b^2 - a_1 a_3 b^2 + a_2^2 b c - 6 a_2 b^2 c - 9 a_2 b c^2 - a b_2 c - 2 b b_1 c \\
& + a_1 b_2 c + a_1 c c_2 - a_2 a_3 c - a_2 b_2 c - a_3 b_1 c - 4 a^2 a_2 c + 4 a^2 a_3 c \\
& + a_1 b_1 c^2 - a a_1 a_3 - a^2 a_2 b_1 + 7 a a_2 c^2 - 2 a^3 a_1 c - 5 a a_1 c^2 \\
& - a a_1 b_2 + a^2 a_1 b_1 + 5 a a_1 b c_2 + 6 a a_2 b c + a_1 b b_1 c - 3 a a_2 a_3 b \\
& + a a_2 b b_1 - 2 a a_2 b b_2 + 3 a^2 a_1 b c + 2 a^2 a_2 b b_1 + 6 a^2 b b_1 c \\
& + a a_1 b^2 b_1 - 4 a^2 a_1 b b_1 + 4 a a_1 a_3 b - a a_1 b b_1 + 3 a a_1 b b_2 \\
& - a a_1 b c + a a_1 b c_1 - 4 a a_3 b b_1 + 8 a b b_1 c + 8 a b b_2 c - a a_3 b c \\
& - a_1 a_2 b c - a_1 a_3 b c + 2 a_1 b b_2 c - 5 a a_1 b^2 c - a a_1 b b_3 - b^3 \\
& + 4 a a_1 b b_1 c + a^3 c^2 + 2 a^3 c + 2 a c^2 + a_1 c^2 + 2 a_1 c^3 - 9 a^2 c^2 \\
& - a a_1 b_2 c + 2 a^2 a_1 b b_2 - 3 a^2 b b_{11} c - 2 a b b_1 b_2 - 2 a b b_{12} c \\
& + b c_2 c_3 - 9 a^2 b^2 c_1 + 10 a^2 b^2 c_2 + 5 a b^3 c_1 + 4 a b^2 c_1^2 + 3 a^2 b c_1 \\
& - 4 a^2 b c_2 - a^2 b c_{23} - 2 a^2 b c_3 - 4 a b^2 c_1 + a b^2 c_2 + 2 a b^2 c_3 \\
& - a b c_1^2 + 4 a b c_2^2 - 2 a_1 b^2 c_2 - a_1 b^2 c_3 + 2 a_2 b^2 c_1 - a_3 b^2 c_1 \\
& + 4 b^2 c c_2 - 3 b c^2 c_1 + 2 b c^2 c_2 + b c c_1^2 + a^2 c c_3 + 4 a c^2 c_1 - a c^2 c_2 \\
& - b_1 c^2 c_1 + b_1 c^2 c_2 - 2 b_2 c^2 c_1 + a c c_{23} + a_3 c c_3 - b_2 c c_1 \\
& + 2 b_2 c c_2 + b_2 c c_3 - c c_1 c_2 + c c_2 c_3 - a_3 c c_1 + 2 a_3 c c_2 - 2 a^2 c c_1 \\
& - a^2 b_1 c_1 - a a_3 c_3 + 2 a b c_1 - a b c_2 + a b c_{23} - a b c_3 - a b_2 c_3 \\
& + 2 a c c_1 - a c c_2 - a c c_3 - a c_2 c_3 - a_3 b c_1 + 2 a_3 b c_2 + a_3 b c_3 \\
& - b b_2 c_1 + 2 b b_2 c_2 + b b_2 c_3 - 2 b c c_1 - 2 b c c_{23} - b c_1 c_2 \\
& + 4 a^2 a_1 c + 2 a_1 b_2 c^2 - a_2 b_1 c^2 + a_1 a_3 c + 2 a_3 b_2 c - b_1 c c_2 \\
& + 2 a b_1^2 c + 8 a b_1 c^2 + 3 a b_2 c^2 - 7 a^2 b_1 c + 3 a^2 b_2 c - a^3 b_1 c \\
& - a^2 b_1^2 c - b_1 b_2 c - 2 a a_3 c + a b_1 b_2 + a b_1 c_2 - 2 a^3 b_1 b_2 \\
& + 10 a^3 b c + 2 a^3 b c_1 - a^2 b^2 b_1 - 12 a^2 b^2 c + a^2 b^2 c_{11} + a^3 a_2 b \\
& + a_1^2 b^2 c + 27 a b c^2 - 3 b^2 b_1 c + b^2 b_1 c_1 + 2 a_3 b b_2 - 2 a a_1 b \\
& + 2 a a_2 b + a_1 b b_2 + 2 a_1 b c + a_1 b c_2 + a^2 c^2 c_1 + 5 a^2 a_1 c^2 \\
& + 2 a a_3 c c_2 - a b_1 b_3 c + 2 a b_2 c c_2 + a a_2 b_1 c^2 - 2 a b_1 c^2 c_1 \\
& - 2 a c c_1 c_2 - a a_1 b_3 c - a a_2 a_3 c - 2 a a_2 c c_2 - a a_3 c c_1 - a^2 a_2 b_2 c \\
& - a^2 b_1 c c_2 - a^2 b_2 c c_1 - a a_1 b_2 c^2 + a^2 a_3 b_1 c + 3 a^2 b_1 c c_1 \\
& + a a_1 c c_2 + a a_2 c c_1 - a^2 a_1 b_1 c + 2 a^2 a_1 b_2 c - a a_1 a_2 c \\
& + 2 a b c c_1^2 - a_1 b b_1 c^2 + 3 a^2 b b_{12} c - 8 a^2 b b_2 c - 3 a^2 b c c_1
\end{aligned}$$

$$\begin{aligned}
& +a^2 a l a_2 b - a^2 a l a_3 b + a^2 a l b b_3 - 2 a^2 a l b c_2 + 2 a^2 a_2 a_3 b - a^4 c \\
& - a b^2 b l c + a b^2 b l l c - 2 a b^2 c c l l - 4 a b b l c^2 - a^2 a_2 b b_2 \\
& - 6 a^2 a_2 b c - 2 a^2 a_2 b c l + 4 a^2 a_2 b c_2 - 2 a^2 a_3 b c l - 3 a^2 b b l b_2 \\
& - 2 a^3 a l b b_2 - a^3 a l b c + a^3 b b l c + a^3 b b l c l + a^3 b b l l c \\
& + 4 a^2 a l b^2 c + 4 a^2 a l b^2 c l - 2 a a l^2 b^2 c + 2 a^3 a l b b l + 2 a b c c l_2 \\
& - 2 a b c c_2 l_2 - a_2 a_3 b c - 4 a_2 b b_2 c + 3 a_3 b b l c - 2 b b l b_2 c \\
& + 2 a b b l l c^2 + a b c^2 c l - a b c^2 c l l - c_3 a^3 + b^3 c l + 2 b^3 c_2 + b^2 c l^2 \\
& + c_3 a^2 - b^2 c l - b^2 c_2 l_2 + b c_2^2 - 2 c^3 c l - c^2 c l - c^2 c_2 l_2 + c c_2^2 \\
& - 4 a b b l c c l + 12 a c^3 + 2 a b b_2^2 - 2 a_2 b^2 b_2 - a^2 b b_2 l_2 - 2 b b_2 l_2 c \\
& + a b b_2 l_2 - 2 b^2 b_2 c l + a b_2 l_2 c + a^2 b l c_3 + a^2 c c_2 - a_2 c c_2 - 2 a a l c \\
& - 2 a^3 c c l - a^2 c + 2 a b^2 b l c l - 2 a b b l^2 c - 2 a l b^2 b l c - 2 a b b_3 c \\
& + a l b b_3 c + b_2^2 c - a^2 b l^2 + a^3 b l^2 + a_3^2 b - 3 b^2 c - 3 b c^2 + 4 a^3 b^2 \\
& - 5 a^2 b^2 + 3 a b^3 - 8 b^3 c - 18 b^2 c^2 - 16 b c^3 + 2 a b^2 - a l b^3 + a l b^2 \\
& - a_2 b^2 + a_3 b^2 + a_3^2 c - a_2 c^2 + a_3 c^2 - b l^2 c^2 - 3 b l c^3 - b l c^2 \\
& - a a l c_2 - c_2 a_3 a^2 + c l b_2 a^2 + c_2 c l a^2 + a_3 a_2 a + b_2 a_2 a + c_2 a_2 a \\
& - 2 b_2 a_3 a + c l a_3 a - 2 c_2 a_3 a + b_2 a_3 a^2 + c l b_2 a - 2 c_2 b_2 a \\
& + c_2 c l a + c l a_3 a^2 - c_2 b_3 a - b_3 a_3 a - b_3 b_2 a + a l_3 b^3 + a^5 b \\
& - a^4 b^2 + 4 a^3 b^3 + b^3 b l_2 - a_3 b^2 + 4 a b^4 - 2 a l b^4 - a^5 b l - 4 a_2 c^3 \\
& + b l_2 c^3 - 4 b_2 c^3 - a_3 c^2 + a^3 b_2^2 + a^4 b l^2 - 6 a^2 b c^2 - a^2 b c l^2 \\
& + 2 a a_2 b^3 + 2 a b^3 b l + 8 a b^3 c - a b^3 c l l + a_3 b b_3 - 2 a_3 b c \\
& + b b_2 b_3 + b b_3 c_2 + a a_3 b + 2 a l_3 b^2 c + a l_3 b c^2 - a_2 a_3 b^2 \\
& + a_3 b^2 b l - b^2 b l b_2 + b^2 b l c_2 + 3 b^2 b l_2 c - 8 b^2 b_2 c + 3 b b l_2 c^2 \\
& - 10 b b_2 c^2 + 3 a a_3^2 b + a b^2 c l_2 - a b^2 c_2 l_2 - a^2 a_3 b + 4 a b^2 c^2 \\
& - a l b^3 b l - 4 a l b^3 c - 2 a l b^2 c^2 + a^2 a l_3 b^2 - a^2 a_2^2 b + 6 a^2 a_3 b^2 \\
& + 2 a^2 b^2 b l_2 + a c^2 c l_2 - a c^2 c_2 l_2 + 2 a c c_2^2 + a l b_3 c^2 - 2 a_2 b_2 c^2 \\
& + 2 a_3 b l c^2 - b l b_2 c^2 + a a_3 c + a^2 b l_2 c^2 - 2 a^2 b_2 c^2 + a^3 a_3 b_2 \\
& + a^3 b_2 c_2 - a^4 b l b_2 - a a_2 b_3^2 + a^3 a l_3 b - a^3 a_2 b_3 + 6 a^3 b b_2 \\
& - 2 a^3 b b_3 + a^3 b c l_2 - a^3 b c_2 - a^3 b c_2 l_2 - 2 a^3 a l b^2 + 2 a^3 a_2 b^2 \\
& - 3 a^3 b^2 c l - a^3 b^2 c l l - a^2 a l^2 b^2 - 2 a^2 a l b^3 + a^4 a l b - a^4 a_2 b \\
& - a^4 b b l - a^4 b b l l + a^4 b b l_2 - a^4 b c l - a^2 c c l_2 + a^2 c c_2 l_2 + a a_2^2 c \\
& + 2 a^3 a_2 c + 3 a^3 b_2 c - 3 a^2 a_2 c^2 + a^4 b l c + a a l_3 c^2 - a a_2 b_3 c^2 \\
& - 3 a a_3 c^2 - 2 a b_3 c^2 + a_3 b_3 c + b_2 b_3 c + b_3 c c_2 - 3 a a l c^3 - a b l c^3 \\
& + a b l l c^3 - a^3 b l^2 c + a^3 b l l c - a^3 b l_2 c + 2 a^2 b l c^2 - 2 a^2 b l l c^2 \\
& + 2 a^3 c c_2 - a^3 b l c l - a^3 a_3 b l - a^2 a l_3 c + a^2 a_2 b_3 c + 3 a^2 b_3 c - b^4 \\
& - a^2 b^2 b l l + 2 a^2 b b l^2 + a^2 b l b_3 - a b b_3 - a b_3 c - 6 a^2 b^3 + a l^2 b^3 \\
& + a_2^2 b^2 - a_2 b^3 - b^2 b l + b b_2^2 + 3 a^3 b - a^2 b - 3 a^4 b + a_2 b^2 b l \\
& - b b l^2 c - 6 b b l c^2 - a b^2 b l_2 + a b b l^2 + a^2 a_2 b - a l a_2 b^2 \\
& - 8 a^2 a_2 b^2 - 4 a a l b^3 - 2 a^3 b b l + a^3 b b l l - a^3 b b l_2 - 2 a a_3 b
\end{aligned}$$

$$\begin{aligned}
& -a^3 b b l - a^2 a l 3 b - b b l b 2 - a b l 2 c^2 - c^3, a^2 - a a l + 2 a b - a l b \\
& - a l l b - a + a l 3 + a 2 + a 2 l - a 2 2 + 2 a 3 + b + c, -2 a^2 a l b^2 \\
& + 2 a a l^2 b^2 + a^3 a l - a^3 a 2 + a^3 a 3 + a^2 a l b - a^2 a l b l - 3 a^2 a l c \\
& - a^2 a l 3 b - a^2 a 2 b + a^2 a 2 b l + 2 a^2 a 2 c + a^2 a 3 b - a^2 a 3 b l \\
& + a^2 a 3 l b - 2 a a l a 2 b - 3 a a l a 3 b - 4 a a l b^2 + 2 a a l b b l \\
& - 2 a a l b b 2 - 2 a a l b c - a a l b c l - 2 a a l b c 2 + 3 a a l b l c \\
& + 2 a a l c^2 + 2 a a 2^2 b + 4 a a 2 b^2 + 4 a a 2 b c + 2 a a 2 b c l - 2 a a 2 b l c \\
& - a l^2 b^2 - a l^2 b c + 2 a l b^3 + 4 a l b^2 c + 2 a l b^2 c l - 2 a l b b l c \\
& + 2 a l b c^2 + 2 a l b c c l - 2 a l b l c^2 - a^2 a l + a^2 a 2 - a^2 a 3 + a a l a 3 \\
& + 2 a a l b + a a l b 2 + 2 a a l c + a a l c 2 + a a l 3 b + a a l 3 c - a a 2 a 3 \\
& - 2 a a 2 b - a a 2 b 2 - 2 a a 2 c - a a 2 c 2 + a a 3^2 + 2 a a 3 b + a a 3 b 2 \\
& + 2 a a 3 c + a a 3 c 2 - a a 3 l b - a a 3 l c + a l a 2 b + a l a 2 c - a l b^2 \\
& - a l b b 2 - 2 a l b c - a l b c 2 - a l b 2 c - a l c^2 - a l c c 2 - a l 3 b^2 \\
& - 2 a l 3 b c - a l 3 c^2 - a 2^2 b - a 2^2 c + a 2 a 3 b + a 2 a 3 c + a 2 b^2 \\
& - a 2 b b l + 2 a 2 b b 2 + 2 a 2 b c - a 2 b c l + 2 a 2 b c 2 - a 2 b l c \\
& + 2 a 2 b 2 c + a 2 c^2 - a 2 c c l + 2 a 2 c c 2 - a 3 b^2 - a 3 b b l - 2 a 3 b c \\
& - a 3 b c l - a 3 b l c - a 3 c^2 - a 3 c c l + a 3 l b^2 + 2 a 3 l b c + a 3 l c^2, \\
& -5 a^2 a l b^2 + 2 a^2 a l b b l - 2 a^2 a l b b 2 + 2 a^2 a 2 b^2 + a a l^2 b^2 \\
& + 4 a a l b^3 + 4 a a l b^2 c + 2 a a l b^2 c l - 2 a a l b b l c - 2 a l^2 b^3 \\
& - 2 a l^2 b^2 c + a^3 a l - a^3 a 2 + a^3 a 3 + a^2 a l b - a^2 a l b l - 4 a^2 a l c \\
& - a^2 a 2 b + a^2 a 2 b l + 3 a^2 a 2 c - a^2 a 2 3 b + a^2 a 3 b - a^2 a 3 b l - a^2 a 3 c \\
& + a^2 a 3 2 b - a a l a 2 b - 3 a a l a 3 b - 3 a a l b^2 + a a l b b l - a a l b b 2 \\
& + 2 a a l b c - a a l b c l - 3 a a l b c 2 + 2 a a l b l c + 2 a a l b 2 c \\
& + 5 a a l c^2 + a a 2^2 b + a a 2 a 3 b + 4 a a 2 b^2 - 2 a a 2 b b l + 2 a a 2 b b 2 \\
& + 2 a a 2 b c + a a 2 b c l + 2 a a 2 b c 2 - 3 a a 2 b l c - 2 a a 2 c^2 - 2 a a 3 b^2 \\
& - 2 a a 3 b c - a a 3 b c l + a a 3 b l c + 2 a l a 2 b^2 + 2 a l a 2 b c \\
& + 3 a l a 3 b^2 + 3 a l a 3 b c + a l b^3 + a l b^2 c l + 2 a l b^2 c 2 - a l b b l c \\
& - 2 a l b b 2 c - 3 a l b c^2 + a l b c c l + 2 a l b c c 2 - a l b l c^2 - 2 a l b 2 c^2 \\
& - 2 a l c^3 - 2 a 2^2 b^2 - 2 a 2^2 b c - 2 a 2 b^3 - 4 a 2 b^2 c - 2 a 2 b^2 c l \\
& + 2 a 2 b b l c - 2 a 2 b c^2 - 2 a 2 b c c l + 2 a 2 b l c^2 - a^2 a l + a^2 a 2 \\
& - a^2 a 3 + a a l a 3 + 2 a a l b + a a l b 2 + 2 a a l c + a a l c 2 - a a 2 a 3 \\
& - 2 a a 2 b - a a 2 b 2 - 2 a a 2 c - a a 2 c 2 + a a 2 3 b + a a 2 3 c + a a 3^2 \\
& + 2 a a 3 b + a a 3 b 2 + 2 a a 3 c + a a 3 c 2 - a a 3 2 b - a a 3 2 c - a l a 3 b \\
& - a l a 3 c - a l b^2 - a l b b 2 - 2 a l b c - a l b c 2 - a l b 2 c - a l c^2 \\
& - a l c c 2 + a 2 a 3 b + a 2 a 3 c + a 2 b^2 + a 2 b b 2 + 2 a 2 b c + a 2 b c 2 \\
& + a 2 b 2 c + a 2 c^2 + a 2 c c 2 - a 2 3 b^2 - 2 a 2 3 b c - a 2 3 c^2 - a 3^2 b - a 3^2 c \\
& - a 3 b^2 - a 3 b b 2 - 2 a 3 b c - a 3 b c 2 - a 3 b 2 c - a 3 c^2 - a 3 c c 2 \\
& + a 3 2 b^2 + 2 a 3 2 b c + a 3 2 c^2, -5 a^2 b^2 c l + 2 a^2 b^2 c 2 + 2 a^2 b b l c l
\end{aligned}$$



$$\begin{aligned}
& -2a^2b b2 c1 + a a1 b^2 c1 - 2a a1 b^2 c2 + 2a a2 b^2 c1 + 4a b^3 c1 \\
& + 4a b^2 c c1 + 2a b^2 c l^2 - 2a b b1 c c1 - 2a1 b^3 c1 - 2a1 b^2 c c1 \\
& + a^3 c1 - a^3 c2 + a^3 c3 + a^2 b c1 - a^2 b c2 - a^2 b c23 + a^2 b c3 + a^2 b c32 \\
& - a^2 b1 c1 + a^2 b1 c2 - a^2 b1 c3 - 4a^2 c c1 + 3a^2 c c2 - a^2 c c3 \\
& - a a2 b c1 + a a2 b c2 - a a2 b c3 - 3a a3 b c1 + 2a a3 b c2 - 3a b^2 c1 \\
& + 4a b^2 c2 - 2a b^2 c3 + a b b1 c1 - 2a b b1 c2 - a b b2 c1 + 2a b b2 c2 \\
& + 2a b c c1 + 2a b c c2 - 2a b c c3 - a b c l^2 - 2a b c1 c2 - a b c1 c3 \\
& + 2a b c2^2 + 2a b1 c c1 - 3a b1 c c2 + a b1 c c3 + 2a b2 c c1 + 5a c^2 c1 \\
& - 2a c^2 c2 + a1 b^2 c2 + a1 b^2 c3 + a1 b c c2 + a1 b c c3 + a2 b^2 c1 \\
& - 2a2 b^2 c2 + a2 b c c1 - 2a2 b c c2 + 2a3 b^2 c1 + 2a3 b c c1 + b^3 c1 \\
& - 2b^3 c2 - 4b^2 c c2 + b^2 c l^2 - b b1 c c1 + 2b b1 c c2 - 2b b2 c c1 \\
& - 3b c^2 c1 - 2b c^2 c2 + b c c l^2 - b1 c^2 c1 + 2b1 c^2 c2 - 2b2 c^2 c1 \\
& - 2c^3 c1 - a^2 c1 + a^2 c2 - a^2 c3 + a a3 c1 - a a3 c2 + a a3 c3 + 2a b c1 \\
& - 2a b c2 + a b c23 + 2a b c3 - a b c32 + a b2 c1 - a b2 c2 + a b2 c3 \\
& + 2a c c1 - 2a c c2 + a c c23 + 2a c c3 - a c c32 + a c1 c2 - a c2^2 \\
& + a c2 c3 - a3 b c1 + a3 b c2 - a3 b c3 - a3 c c1 + a3 c c2 - a3 c c3 \\
& - b^2 c1 + b^2 c2 - b^2 c23 - b^2 c3 + b^2 c32 - b b2 c1 + b b2 c2 - b b2 c3 \\
& - 2b c c1 + 2b c c2 - 2b c c23 - 2b c c3 + 2b c c32 - b c1 c2 + b c2^2 \\
& - b c2 c3 - b2 c c1 + b2 c c2 - b2 c c3 - c^2 c1 + c^2 c2 - c^2 c23 - c^2 c3 \\
& + c^2 c32 - c c1 c2 + c c2^2 - c c2 c3, a^4 b - a^4 b1 + a^4 b2 + a^3 a1 b \\
& - a^3 a2 b + 2a^3 b^2 - a^3 b b1 - a^3 b b11 + a^3 b b12 - a^3 b c1 + a^3 b l^2 \\
& - a^3 b1 b2 + a^3 b1 c - 4a^2 a1 b^2 + 2a^2 a1 b b1 - 2a^2 a1 b b2 - a^2 a1 b c \\
& + 2a^2 a2 b^2 - 2a^2 b^2 b1 - 3a^2 b^2 c1 - a^2 b^2 c11 + a^2 b b1 c + a^2 b b1 c1 \\
& + a^2 b b11 c - a^2 b l^2 c - a a l^2 b^2 + 4a a1 b^3 + a a1 b^2 b1 + 4a a1 b^2 c \\
& + 4a a1 b^2 c1 - 3a a1 b b1 c - 2a l^2 b^3 - 2a l^2 b^2 c - 2a^3 b + 2a^3 b1 \\
& - 2a^3 b2 - a^3 c + a^3 c1 - a^3 c2 - a^2 a1 b - 2a^2 a1 c + a^2 a13 b + a^2 a2 b \\
& + 2a^2 a2 c - a^2 a23 b + 2a^2 a3 b - a^2 a3 b1 + a^2 a3 b2 - a^2 b b1 \\
& + a^2 b b11 + 2a^2 b b2 - a^2 b b22 + a^2 b c + 2a^2 b c1 + a^2 b c12 - a^2 b c2 \\
& - a^2 b c22 - a^2 b l^2 - 5a^2 b1 c - a^2 b1 c1 + a^2 b11 c - a^2 b12 c + a^2 b2^2 \\
& + 5a^2 b2 c + a^2 b2 c2 + a^2 c^2 - 2a^2 c c1 + 2a^2 c c2 + a a1 a2 b \\
& - a a1 a3 b + 3a a1 b^2 - a a1 b b1 + 8a a1 b c - 2a a1 b c2 - a a1 b1 c \\
& + 2a a1 b2 c + 5a a1 c^2 - a a2^2 b + 2a a2 a3 b - a a2 b^2 - 2a a2 b b1 \\
& + 3a a2 b b2 - 4a a2 b c - 2a a2 b c1 + 4a a2 b c2 - a a2 b2 c \\
& - 3a a2 c^2 - a a3 b b1 - 2a a3 b c1 + a a3 b1 c + 2a b^3 - a b^2 b1 \\
& - a b^2 b11 + a b^2 b12 + 2a b^2 b2 + 4a b^2 c - 4a b^2 c1 + a b^2 c11 \\
& + 4a b^2 c2 + 2a b b l^2 - 2a b b1 b2 + 3a b b1 c + a b b1 c1 - a b b1 c2 \\
& - 3a b b11 c + 2a b b12 c - a b b2 c1 + 2a b c^2 - 3a b c c1 + a b c c11 \\
& + 4a b c c2 - a b c l^2 + 3a b l^2 c - 2a b1 b2 c + 4a b1 c^2 + 3a b1 c c1
\end{aligned}$$

$$\begin{aligned}
& -a b l c c 2 - 2 a b l 1 c^2 + a b l 2 c^2 - 2 a b 2 c^2 - a b 2 c c 1 + a c^2 c l \\
& + a l^2 b^2 + a l^2 b c + 2 a l a 2 b^2 + 2 a l a 2 b c + 2 a l a 3 b^2 + 2 a l a 3 b c \\
& - 2 a l b^3 - a l b^2 b 1 - a l b^2 b 2 - 7 a l b^2 c - 2 a l b^2 c 1 - 2 a l b b 2 c \\
& - 8 a l b c^2 - 2 a l b c c 1 + a l b 1 c^2 - a l b 2 c^2 - 3 a l c^3 - 2 a 2^2 b^2 \\
& - 2 a 2^2 b c - 2 a 2 b^3 + a 2 b^2 b 1 - 4 a 2 b^2 c + 2 a 2 b b 1 c - 2 a 2 b c^2 \\
& + a 2 b 1 c^2 + b^3 c 1 - b^3 c 1 1 - b^2 b 1 c + 2 b^2 b 1 c 1 + b^2 b 1 1 c + 2 b^2 c c 1 \\
& - 2 b^2 c c 1 1 + 2 b^2 c l^2 - 2 b b l^2 c - 2 b b 1 c^2 + 2 b b 1 1 c^2 + b c^2 c 1 \\
& - b c^2 c 1 1 + 2 b c c l^2 - 2 b l^2 c^2 - b l c^3 - 2 b l c^2 c 1 + b 1 1 c^3 + a^2 b \\
& - a^2 b 1 + a^2 b 2 + a^2 c - a^2 c 1 + a^2 c 2 - a a l 3 b - a a l 3 c + a a 2 3 b \\
& + a a 2 3 c - 2 a a 3 b + a a 3 b 1 - a a 3 b 2 - 2 a a 3 c + a a 3 c 1 - a a 3 c 2 \\
& - 2 a b^2 + 2 a b b 1 - a b b 1 2 - 2 a b b 2 + a b b 2 2 - 4 a b c + 2 a b c 1 \\
& - a b c 1 2 - 2 a b c 2 + a b c 2 2 + a b 1 b 2 + 2 a b 1 c + a b 1 c 2 - a b 1 2 c \\
& - a b 2^2 - 2 a b 2 c + a b 2 c 1 - 2 a b 2 c 2 + a b 2 2 c - 2 a c^2 + 2 a c c 1 \\
& - a c c 1 2 - 2 a c c 2 + a c c 2 2 + a c 1 c 2 - a c 2^2 - a l a 2 b - a l a 2 c \\
& + a l b b 2 + a l b c 2 + a l b 2 c + a l c c 2 + a l 3 b^2 + 2 a l 3 b c + a l 3 c^2 \\
& + a 2^2 b + a 2^2 c - a 2 a 3 b - a 2 a 3 c + a 2 b b 1 - 2 a 2 b b 2 + a 2 b c 1 \\
& - 2 a 2 b c 2 + a 2 b 1 c - 2 a 2 b 2 c + a 2 c c 1 - 2 a 2 c c 2 - a 2 3 b^2 \\
& - 2 a 2 3 b c - a 2 3 c^2 + 2 a 3 b^2 - a 3 b b 1 + 2 a 3 b b 2 + 4 a 3 b c - a 3 b c 1 \\
& + 2 a 3 b c 2 - a 3 b 1 c + 2 a 3 b 2 c + 2 a 3 c^2 - a 3 c c 1 + 2 a 3 c c 2 + b^3 \\
& - b^2 b 1 + b^2 b 1 2 + b^2 b 2 - b^2 b 2 2 + 3 b^2 c - b^2 c 1 + b^2 c 1 2 + b^2 c 2 \\
& - b^2 c 2 2 - 2 b b 1 b 2 - 2 b b 1 c - 2 b b 1 c 2 + 2 b b 1 2 c + 2 b b 2^2 \\
& + 2 b b 2 c - 2 b b 2 c 1 + 4 b b 2 c 2 - 2 b b 2 2 c + 3 b c^2 - 2 b c c 1 \\
& + 2 b c c 1 2 + 2 b c c 2 - 2 b c c 2 2 - 2 b c 1 c 2 + 2 b c 2^2 - 2 b 1 b 2 c - b 1 c^2 \\
& - 2 b 1 c c 2 + b 1 2 c^2 + 2 b 2^2 c + b 2 c^2 - 2 b 2 c c 1 + 4 b 2 c c 2 - b 2 2 c^2 \\
& + c^3 - c^2 c 1 + c^2 c 1 2 + c^2 c 2 - c^2 c 2 2 - 2 c c 1 c 2 + 2 c c 2^2, a^4 b 1 - a^4 b 2 \\
& - 2 a^3 a 1 b + a^3 a 2 b + 2 a^3 b^2 - 2 a^3 b c - a^3 b c 1 - a^3 b l^2 + a^3 b 1 b 2 \\
& - a^3 b 1 c - a^2 a 1 b^2 + 2 a^2 a 1 b b 1 + 3 a^2 a 1 b c - a^2 a 2 b b 1 - 2 a^2 b^2 b 1 \\
& - 4 a^2 b^2 c - 5 a^2 b^2 c 1 - a^2 b^2 c 1 1 + 2 a^2 b b 1 c + a^2 b l^2 c + a a 1 b^2 b 1 \\
& + 8 a a 1 b^2 c + 4 a a 1 b^2 c 1 - 3 a a 1 b b 1 c - 4 a l^2 b^2 c + a^3 a 1 - a^3 a 2 \\
& + a^3 a 3 - 3 a^3 b 1 + 3 a^3 b 2 + a^3 c 3 + 5 a^2 a 1 b - a^2 a 1 b 1 - 3 a^2 a 1 c \\
& - 3 a^2 a 2 b + a^2 a 2 b 1 + 3 a^2 a 2 c + a^2 a 3 b - a^2 a 3 b 2 - 3 a^2 a 3 c \\
& - 4 a^2 b^2 + a^2 b b 1 - a^2 b b 2 - a^2 b c + a^2 b c 1 2 + a^2 b c 1 3 - a^2 b c 2 2 \\
& + 2 a^2 b c 3 + 2 a^2 b l^2 - a^2 b 1 b 2 + 9 a^2 b 1 c + a^2 b 1 c 2 - a^2 b 1 c 3 \\
& - a^2 b 2^2 - 7 a^2 b 2 c - a^2 b 2 c 2 + 2 a^2 c^2 + a^2 c c 1 - 2 a a 1 a 3 b - a a 1 b^2 \\
& - 3 a a 1 b b 1 - 2 a a 1 b b 2 - 16 a a 1 b c - a a 1 b c 1 - 4 a a 1 b c 2 \\
& - a a 1 b c 3 + 3 a a 1 b 1 c + 3 a a 1 c^2 + a a 2 a 3 b + a a 2 b^2 + 2 a a 2 b b 1 \\
& + a a 2 b b 2 + 10 a a 2 b c + 4 a a 2 b c 2 - 4 a a 2 b 1 c + a a 2 b 2 c \\
& - 3 a a 2 c^2 + 2 a a 3 b^2 - a a 3 b b 1 - 6 a a 3 b c - 3 a a 3 b c 1
\end{aligned}$$

$$\begin{aligned}
& + 2 a a^3 b l c + 2 a b^3 + 2 a b^2 b l + 2 a b^2 b^2 + 6 a b^2 c - 4 a b^2 c l \\
& + a b^2 c l l + 8 a b^2 c^2 + 4 a b b l c + 5 a b b l c l - a b b l c^2 - 4 a b b^2 c \\
& - 3 a b b^2 c l + 2 a b c^2 + 7 a b c c l + a b c c l l - 6 a b l^2 c + 4 a b l b^2 c \\
& - 10 a b l c^2 - a b l c c l - a b l c c^2 + 2 a b^2 c^2 + a b^2 c c l - 2 a c^3 \\
& - a c^2 c l + a l^2 b c + 4 a l a^2 b c - a l a^3 b^2 + 7 a l a^3 b c - a l b^3 \\
& - a l b^2 b^2 + 9 a l b^2 c - 4 a l b^2 c l - 4 a l b^2 c^2 + 2 a l b b l c \\
& + 6 a l b b^2 c + 9 a l b c^2 + 4 a l b c c^2 - 2 a l b l c^2 - a l b^2 c^2 - a l c^3 \\
& - 4 a^2 b c - 8 a^2 b^2 c + 4 a^2 b^2 c l - 4 a^2 b b l c - 8 a^2 b c^2 - 4 a^2 b c c l \\
& + 4 a^2 b l c^2 - 4 b^3 c + 3 b^3 c l - b^3 c l l - 4 b^2 b l c + b^2 b l c l - 8 b^2 c^2 \\
& - 2 b^2 c c l - 2 b^2 c c l l + 4 b^2 c l^2 - 6 b b l c c l - 4 b c^3 - 5 b c^2 c l \\
& - b c^2 c l l + 4 b l^2 c^2 + 4 b l c^3 + b l c^2 c l - 2 a^2 a l + 2 a^2 a^2 - 2 a^2 a^3 \\
& + 3 a^2 b l - 3 a^2 b^2 + a^2 c l - a^2 c^2 - a^2 c^3 + a a l a^3 - 2 a a l b + a a l b l \\
& + a a l b^2 + 6 a a l c + a a l c^2 - a a^2 a^3 + a a^2 b - a a^2 b l - a a^2 b^2 \\
& - 6 a a^2 c - a a^2 c^2 + a a^3^2 - a a^3 b l + 3 a a^3 b^2 + 6 a a^3 c + a a^3 c^2 \\
& + a a^3 c^3 + 2 a b^2 - 2 a b b l + 2 a b b^2 + 3 a b c + 3 a b c l - a b c l^2 \\
& - a b c l^3 - 2 a b c^2 + a b c^2 l + a b c^3 - a b l^2 - a b l b^2 - 9 a b l c \\
& - a b l c l - a b l c^2 + 2 a b^2^2 + 8 a b^2 c + 2 a b^2 c^2 + a b^2 c^3 + a c^2 \\
& - 4 a c c l - a c c l^2 - a c c l^3 + 4 a c c^2 + a c c^2 l + a c c^3 + a c^2 c^3 \\
& - a l a^2 c + 3 a l a^3 b - 3 a l a^3 c + 3 a l b^2 + 3 a l b b^2 - a l b c + a l b c l \\
& + 5 a l b c^2 + a l b c^3 - a l b l c - 3 a l b^2 c - 4 a l c^2 - a l c c^2 + a l c c^3 \\
& + a^2^2 c - 2 a^2 a^3 b + 2 a^2 a^3 c - 2 a^2 b^2 - 2 a^2 b b^2 + 2 a^2 b c - a^2 b c l \\
& - 4 a^2 b c^2 - a^2 b c^3 + 2 a^2 b l c + 2 a^2 b^2 c + 4 a^2 c^2 + a^2 c c l \\
& - a^2 c c^3 + a^3^2 b - 3 a^3^2 c - a^3 b^2 + a^3 b b^2 - 6 a^3 b c - 2 a^3 b c l \\
& + 5 a^3 b c^2 + 4 a^3 b l c - 7 a^3 b^2 c - 5 a^3 c^2 + 2 a^3 c c l - 3 a^3 c c^2 \\
& - 2 b^3 - 2 b^2 b^2 - 5 b^2 c - 3 b^2 c l + b^2 c l^2 + b^2 c l^3 - b^2 c^2 l + 6 b b l c \\
& - b b l c l - 2 b b l c^2 - b b l c^3 - 8 b b^2 c - 2 b b^2 c l + 4 b b^2 c^2 - 4 b c^2 \\
& + 2 b c c l^2 + 2 b c c l^3 - 4 b c c^2 - 2 b c c^2 l - b c l^2 - 4 b c l c^2 - b c l c^3 \\
& + 4 b c^2^2 + b l^2 c + 4 b l b^2 c + 6 b l c^2 + b l c c l + 2 b l c c^2 - b l c c^3 \\
& - 4 b^2^2 c - 6 b^2 c^2 + 2 b^2 c c l - 4 b^2 c c^2 - c^3 + 3 c^2 c l + c^2 c l^2 + c^2 c l^3 \\
& - 4 c^2 c^2 - c^2 c^2 l - c c l c^3 + a a l - a a^2 + a a^3 - a b l + a b^2 - a c l \\
& + a c^2 - a l a^3 - a l b - a l b^2 - a l c - a l c^2 + a^2 a^3 + a^2 b + a^2 b^2 \\
& + a^2 c + a^2 c^2 - a^3^2 - a^3 b + a^3 b l - 2 a^3 b^2 - a^3 c + a^3 c l - 2 a^3 c^2 \\
& + b b l - b b^2 + b c l - b c^2 + b l b^2 + b l c + b l c^2 - b^2^2 - b^2 c + b^2 c l \\
& - 2 b^2 c^2 + c c l - c c^2 + c l c^2 - c^2^2, a^4 b l - a^4 b^2 - 2 a^3 a l b + a^3 a^2 b \\
& + 2 a^3 b^2 - 2 a^3 b c - a^3 b c l - a^3 b l^2 + a^3 b l b^2 - a^3 b l c - a^2 a l b^2 \\
& + 2 a^2 a l b b l + 3 a^2 a l b c - a^2 a^2 b b l - 2 a^2 b^2 b l - 4 a^2 b^2 c \\
& - 7 a^2 b^2 c l - a^2 b^2 c l l + 2 a^2 b b l c + a^2 b l^2 c + a a l b^2 b l + 8 a a l b^2 c \\
& + 6 a a l b^2 c l - 3 a a l b b l c - 4 a l^2 b^2 c + a^3 a l - a^3 a^2 + a^3 a^3
\end{aligned}$$

$$\begin{aligned}
& -3a^3b1 + 3a^3b2 + a^3c1 - a^3c2 + 2a^3c3 + 5a^2a1b - a^2a1b1 \\
& -3a^2a1c - 3a^2a2b + a^2a2b1 + 3a^2a2c + a^2a3b - a^2a3b2 \\
& -3a^2a3c - 4a^2b^2 + a^2b1b1 - a^2b1b2 - a^2b1c + a^2b1c1 + a^2b1c2 \\
& -a^2b1c2 - a^2b1c22 + 3a^2b1c3 + a^2b1c31 + 2a^2b1^2 - a^2b1b2 \\
& + 9a^2b1c - a^2b1c1 + 2a^2b1c2 - 2a^2b1c3 - a^2b2^2 - 7a^2b2c \\
& -a^2b2c2 + 2a^2c^2 - 2a^2cc1 + 2a^2cc2 - 2a1a1a3b - a1a1b^2 \\
& -3a1a1b1b1 - 2a1a1b1b2 - 16a1a1b1c - a1a1b1c1 - 5a1a1b1c2 \\
& -2a1a1b1c3 + 3a1a1b1c + 3a1a1c^2 + a1a2a3b + a1a2b^2 + 2a1a2b1b1 \\
& + a1a2b1b2 + 10a1a2b1c - a1a2b1c1 + 6a1a2b1c2 - 4a1a2b1c3 \\
& + a1a2b2c - 3a1a2c^2 + 2a1a3b^2 - a1a3b1b1 - 6a1a3b1c - 5a1a3b1c1 \\
& + 2a1a3b1c2 + 2a1b^3 + 2a1b^2b1 + 2a1b^2b2 + 6a1b^2c - 8a1b^2c1 \\
& + a1b^2c11 + 12a1b^2c2 + 4a1b1b1c + 7a1b1b1c1 - a1b1b1c2 - 4a1b1b2c \\
& - 5a1b1b2c1 + 2a1b1c^2 + 5a1b1cc1 + a1b1cc11 + 4a1b1cc2 - a1b1c1^2 \\
& - 6a1b1^2c + 4a1b1b2c - 10a1b1c^2 + 2a1b1cc1 - 3a1b1cc2 \\
& + 2a1b2c^2 + a1b2cc1 - 2a1c^3 + a1c^2c1 + a1^2b1c + 4a1a2b1c \\
& - a1a3b^2 + 7a1a3b1c - a1b^3 - a1b^2b2 + 9a1b^2c - 5a1b^2c1 \\
& - 6a1b^2c2 + 2a1b1b1c + 6a1b1b2c + 9a1b1c^2 - a1b1cc1 \\
& + 2a1b1cc2 - 2a1b1c^2 - a1b2c^2 - a1c^3 - 4a2^2b1c - 8a2^2b2c \\
& + 6a2^2b2c1 - 4a2b1b1c - 8a2b1c^2 - 2a2b1cc1 + 4a2b1c^2 - 4b^3c \\
& + 5b^3c1 - b^3c11 - 4b^2b1c + b^2b1c1 - 8b^2c^2 + 2b^2cc1 - 2b^2cc11 \\
& + 6b^2c1^2 - 8b1b1cc1 - 4b1c^3 - 3b1c^2c1 - b1c^2c11 + 2b1cc1^2 \\
& + 4b1^2c^2 + 4b1c^3 - b1c^2c1 - 2a^2a1 + 2a^2a2 - 2a^2a3 + 3a^2b1 \\
& - 3a^2b2 - 2a^2c3 + a1a1a3 - 2a1a1b + a1a1b1 + a1a1b2 + 6a1a1c \\
& + a1a1c2 - a1a2a3 + a1a2b - a1a2b1 - a1a2b2 - 6a1a2c - a1a2c2 \\
& + a1a3^2 - a1a3b1 + 3a1a3b2 + 6a1a3c + a1a3c1 + 2a1a3c3 + 2a1b^2 \\
& - 2a1b1b1 + 2a1b1b2 + 3a1b1c + 5a1b1c1 - a1b1c2 - 4a1b1c3 + a1b1c22 \\
& + 3a1b1c3 - a1b1c31 - a1b1^2 - a1b1b2 - 9a1b1c - a1b1c1 - a1b1c2 \\
& + 2a1b2^2 + 8a1b2c + a1b2c1 + a1b2c2 + 2a1b2c3 + a1c^2 - 2a1cc1 \\
& - a1cc12 + 2a1cc2 + a1cc22 + 3a1cc3 - a1cc31 + a1c1c2 - a1c2^2 \\
& + 2a1c2c3 - a1a2c + 3a1a3b - 3a1a3c + 3a1b^2 + 3a1b1b2 \\
& - a1b1c + a1b1c1 + 6a1b1c2 + 2a1b1c3 - a1b1c - 3a1b2c - 4a1c^2 \\
& + 2a1c1c3 + a2^2c - 2a2a3b + 2a2a3c - 2a2b^2 - 2a2b1b2 \\
& + 2a2b1c - a2b1c1 - 5a2b1c2 - 2a2b1c3 + 2a2b1c + 2a2b2c \\
& + 4a2c^2 + a2cc1 - a2cc2 - 2a2cc3 + a3^2b - 3a3^2c - a3b^2 \\
& + a3b1b2 - 6a3b1c - 3a3b1c1 + 7a3b1c2 + 4a3b1c3 - 7a3b2c \\
& - 5a3c^2 + a3cc1 - a3cc2 - 2b^3 - 2b^2b2 - 5b^2c - 4b^2c1 + b^2c12 \\
& + b^2c2 - b^2c22 - b^2c3 + b^2c31 + 6b1b1c - b1b1c1 - 3b1b1c2 \\
& - 2b1b1c3 - 8b1b2c - 3b1b2c1 + 6b1b2c2 - 4b1c^2 - 2b1cc1
\end{aligned}$$

$$\begin{aligned}
& + 2 b c c l 2 - 2 b c c 2 - 2 b c c 2 2 - 2 b c c 3 + 2 b c c 3 1 - b c l^2 \\
& - 6 b c l c 2 - 2 b c l c 3 + 6 b c 2^2 + b l^2 c + 4 b l b 2 c + 6 b l c^2 + b l c c l \\
& + b l c c 2 - 2 b l c c 3 - 4 b 2^2 c - 6 b 2 c^2 + b 2 c c l - 2 b 2 c c 2 - c^3 \\
& + 2 c^2 c l + c^2 c l 2 - 3 c^2 c 2 - c^2 c 2 2 - c^2 c 3 + c^2 c 3 1 - 2 c c l c 2 \\
& - 2 c c l c 3 + 2 c c 2^2 + a a l - a a 2 + a a 3 - a b l + a b 2 - a c l + a c 2 \\
& - a l a 3 - a l b - a l b 2 - a l c - a l c 2 + a 2 a 3 + a 2 b + a 2 b 2 + a 2 c \\
& + a 2 c 2 - a 3^2 - a 3 b + a 3 b l - 2 a 3 b 2 - a 3 c + a 3 c l - 2 a 3 c 2 + b b l \\
& - b b 2 + b c l - b c 2 + b l b 2 + b l c + b l c 2 - b 2^2 - b 2 c + b 2 c l \\
& - 2 b 2 c 2 + c c l - c c 2 + c l c 2 - c 2^2, a^4 b + a^4 b l - a^4 b 2 - a^3 a l b \\
& + a^3 a 2 b - 2 a^3 b b l + a^3 b b l 1 - a^3 b b l 2 + a^3 b c l - a^3 b l^2 + a^3 b l b 2 \\
& - a^3 b l c + 4 a^2 a l b^2 - 2 a^2 a l b b l + 2 a^2 a l b b 2 + a^2 a l b c \\
& - 2 a^2 a 2 b^2 - 4 a^2 b^3 + a^2 b^2 b l - a^2 b^2 b l 1 + 3 a^2 b^2 c l + a^2 b^2 c l 1 \\
& + a^2 b b l^2 - a^2 b b l c - a^2 b b l c l - a^2 b b l 1 c + a^2 b l^2 c + a a l^2 b^2 \\
& + 4 a a l b^3 - a a l b^2 b l - 4 a a l b^2 c - 4 a a l b^2 c l + 3 a a l b b l c \\
& - 2 a l^2 b^3 + 2 a l^2 b^2 c - 2 a^3 b + a^3 b 3 - a^3 c - a^3 c l + a^3 c 2 - 2 a^2 a l b \\
& + 2 a^2 a l c - a^2 a l 3 b + a^2 a 2 b - 2 a^2 a 2 c + a^2 a 2 3 b - a^2 a 3 b \\
& + a^2 a 3 b l - a^2 a 3 b 2 + 4 a^2 b^2 + 7 a^2 b b l - a^2 b b l 1 + a^2 b b l 2 \\
& + a^2 b b l 3 - 4 a^2 b b 2 + 2 a^2 b b 3 + 4 a^2 b c - a^2 b c l 2 + a^2 b c 2 \\
& + a^2 b c 2 2 - a^2 b l^2 + 2 a^2 b l b 2 - a^2 b l b 3 + 2 a^2 b l c + a^2 b l c l \\
& - a^2 b l 1 c + a^2 b l 2 c - a^2 b 2^2 - a^2 b 2 c - a^2 b 2 c 2 + a^2 c^2 + 2 a^2 c c l \\
& - 2 a^2 c c 2 - a a l a 2 b + a a l a 3 b - 13 a a l b^2 + 6 a a l b b l \\
& - 2 a a l b b 2 - a a l b b 3 + 2 a a l b c 2 + a a l b l c - 2 a a l b 2 c \\
& - 5 a a l c^2 + a a 2^2 b - 2 a a 2 a 3 b + 9 a a 2 b^2 - 4 a a 2 b b l + a a 2 b b 2 \\
& + 2 a a 2 b c l - 4 a a 2 b c 2 + a a 2 b 2 c + 3 a a 2 c^2 - 8 a a 3 b^2 + a a 3 b b l \\
& + 2 a a 3 b c l - a a 3 b l c + 4 a b^3 - 5 a b^2 b l + 2 a b^2 b l 1 - a b^2 b l 2 \\
& - 2 a b^2 b 2 + 4 a b^2 c + 12 a b^2 c l - a b^2 c l 1 - 12 a b^2 c 2 - 3 a b b l^2 \\
& + 2 a b b l b 2 - 20 a b b l c - 7 a b b l c l + a b b l c 2 + 4 a b b l 1 c \\
& - 2 a b b l 2 c + 8 a b b 2 c + 5 a b b 2 c l - a b c c l - a b c c l 1 - 4 a b c c 2 \\
& + a b c l^2 + 2 a b l^2 c - 2 a b l b 2 c - 3 a b l c^2 - 3 a b l c c l + a b l c c 2 \\
& + 2 a b l 1 c^2 - a b l 2 c^2 + 2 a b 2 c^2 + a b 2 c c l - a c^2 c l - a l^2 b c \\
& + 2 a l a 2 b^2 - 2 a l a 2 b c + 6 a l a 3 b^2 - 2 a l a 3 b c + 10 a l b^3 \\
& - a l b^2 b l + 5 a l b^2 b 2 + 11 a l b^2 c + 6 a l b^2 c l + 8 a l b^2 c 2 \\
& - 6 a l b b l c - 2 a l b b 2 c + 4 a l b c^2 + 2 a l b c c l - a l b l c^2 + a l b 2 c^2 \\
& + 3 a l c^3 - 2 a 2^2 b^2 + 2 a 2^2 b c - 6 a 2 b^3 - a 2 b^2 b l - 4 a 2 b^2 c \\
& - 8 a 2 b^2 c l + 6 a 2 b b l c + 2 a 2 b c^2 - a 2 b l c^2 - 4 b^4 - b^3 b l - b^3 b l 1 \\
& - 8 b^3 c - 9 b^3 c l + b^3 c l 1 + b^2 b l^2 + 7 b^2 b l c - 2 b^2 b l c l - 3 b^2 b l 1 c \\
& - 4 b^2 c^2 - 10 b^2 c c l + 2 b^2 c c l 1 - 6 b^2 c l^2 + 4 b b l^2 c + 9 b b l c^2 \\
& + 8 b b l c c l - 3 b b l 1 c^2 - b c^2 c l + b c^2 c l 1 - 2 b c c l^2 - b l^2 c^2 + b l c^3
\end{aligned}$$

$$\begin{aligned}
& + 2 b l c^2 c l - b l l c^3 + a^2 a l - a^2 a 2 + a^2 a 3 + a^2 b - 2 a^2 b l + 2 a^2 b 2 \\
& - a^2 b 3 + a^2 c + 5 a a l b - a a l b l - 3 a a l c + a a l 3 b + a a l 3 c \\
& - 4 a a 2 b + a a 2 b l + 3 a a 2 c - a a 2 3 b - a a 2 3 c + 3 a a 3 b - a a 3 b 2 \\
& + a a 3 b 3 - 3 a a 3 c - a a 3 c l + a a 3 c 2 - 4 a b^2 - a b b l - a b b l 3 \\
& + a b b 3 - 7 a b c - 6 a b c l + a b c l 2 + 4 a b c 2 - a b c 2 2 + a b l^2 \\
& + 6 a b l c + a b l c l - a b l 3 c - a b 2^2 + a b 2 b 3 - 6 a b 2 c - a b 2 c l \\
& + a b 3 c + a b 3 c 2 - 3 a c^2 + a c c l + a c c l 2 - 2 a c c 2 - a c c 2 2 \\
& - a c l c 2 + a c 2^2 + a l a 2 c - 6 a l a 3 b - 5 a l b^2 - 5 a l b b 2 + a l b b 3 \\
& - 3 a l b c - a l b c l - 7 a l b c 2 + a l b l c + a l b 2 c + a l b 3 c + 2 a l c^2 \\
& - a l c c 2 - a l 3 b^2 - 2 a l 3 b c - a l 3 c^2 - a 2^2 c + 5 a 2 a 3 b + a 2 a 3 c \\
& + 4 a 2 b^2 + 4 a 2 b b 2 - a 2 b b 3 + 2 a 2 b c + a 2 b c l + 6 a 2 b c 2 \\
& - 2 a 2 b l c - a 2 b 3 c - 2 a 2 c^2 - a 2 c c l + 2 a 2 c c 2 + a 2 3 b^2 + 2 a 2 3 b c \\
& + a 2 3 c^2 - 4 a 3^2 b - a 3 b^2 + 3 a 3 b b l - 6 a 3 b b 2 + 2 a 3 b c + 5 a 3 b c l \\
& - 10 a 3 b c 2 - a 3 b l c + 2 a 3 b 2 c + 3 a 3 c^2 + a 3 c c l - 2 a 3 c c 2 + 3 b^3 \\
& + 2 b^2 b l + b^2 b l 3 + b^2 b 2 + 8 b^2 c + 5 b^2 c l - b^2 c l 2 - b^2 c 2 + b^2 c 2 2 \\
& + 2 b b l b 2 - b b l b 3 - 2 b b l c + b b l c l + 4 b b l c 2 + 2 b b l 3 c \\
& - 2 b b 2^2 + 6 b b 2 c + 4 b b 2 c l - 8 b b 2 c 2 - b b 3 c l + 7 b c^2 + 4 b c c l \\
& - 2 b c c l 2 + 2 b c c 2 + 2 b c c 2 2 + b c l^2 + 6 b c l c 2 - 6 b c 2^2 - b l^2 c \\
& - 2 b l b 2 c - b l b 3 c - 4 b l c^2 - b l c c l + b l 3 c^2 + 2 b 2^2 c + 5 b 2 c^2 \\
& - b 3 c c l + 2 c^3 - c^2 c l - c^2 c l 2 + 3 c^2 c 2 + c^2 c 2 2 + 2 c c l c 2 - 2 c c 2^2 \\
& - a a l + a a 2 - a a 3 + a b l - a b 2 + a c l - a c 2 + a l a 3 + a l b + a l b 2 \\
& + a l c + a l c 2 - a 2 a 3 - a 2 b - a 2 b 2 - a 2 c - a 2 c 2 + a 3^2 + a 3 b \\
& - a 3 b l + 2 a 3 b 2 + a 3 c - a 3 c l + 2 a 3 c 2 - b b l + b b 2 - b c l + b c 2 \\
& - b l b 2 - b l c - b l c 2 + b 2^2 + b 2 c - b 2 c l + 2 b 2 c 2 - c c l + c c 2 \\
& - c l c 2 + c 2^2, a^4 b + a^4 b l - a^4 b 2 - a^3 a l b + a^3 a 2 b - 2 a^3 b b l \\
& + a^3 b b l l - a^3 b b l 2 + a^3 b c l - a^3 b l^2 + a^3 b l b 2 - a^3 b l c + 4 a^2 a l b^2 \\
& - 2 a^2 a l b b l + 2 a^2 a l b b 2 + a^2 a l b c - 2 a^2 a 2 b^2 - 4 a^2 b^3 - a^2 b^2 b l \\
& - a^2 b^2 b l l + 3 a^2 b^2 c l + a^2 b^2 c l l + a^2 b b l^2 - a^2 b b l c - a^2 b b l c l \\
& - a^2 b b l l c + a^2 b l^2 c + a a l^2 b^2 + 4 a a l b^3 + a a l b^2 b l - 4 a a l b^2 c \\
& - 4 a a l b^2 c l + 3 a a l b b l c - 2 a l^2 b^3 + 2 a l^2 b^2 c - 2 a^3 b + a^3 b l \\
& - a^3 b 2 + 2 a^3 b 3 - a^3 c - a^3 c l + a^3 c 2 - 2 a^2 a l b + 2 a^2 a l c - a^2 a l 3 b \\
& + a^2 a 2 b - 2 a^2 a 2 c + a^2 a 2 3 b - a^2 a 3 b + a^2 a 3 b l - a^2 a 3 b 2 + 4 a^2 b^2 \\
& + 8 a^2 b b l - a^2 b b l l + a^2 b b l 2 - 5 a^2 b b 2 + 3 a^2 b b 3 + a^2 b b 3 l \\
& + 4 a^2 b c - a^2 b c l 2 + a^2 b c 2 + a^2 b c 2 2 - 2 a^2 b l^2 + 3 a^2 b l b 2 \\
& - 2 a^2 b l b 3 - a^2 b l c + a^2 b l c l - a^2 b l l c + a^2 b l 2 c - a^2 b 2^2 + a^2 b 2 c \\
& - a^2 b 2 c 2 + a^2 c^2 + 2 a^2 c c l - 2 a^2 c c 2 - a a l a 2 b + a a l a 3 b \\
& - 13 a a l b^2 + 6 a a l b b l - 3 a a l b b 2 - 2 a a l b b 3 + 2 a a l b c 2 \\
& + a a l b l c - 2 a a l b 2 c - 5 a a l c^2 + a a 2^2 b - 2 a a 2 a 3 b + 9 a a 2 b^2
\end{aligned}$$

$$\begin{aligned}
& -5 a^2 b b_1 + 3 a^2 b b_2 + 2 a^2 b c_1 - 4 a^2 b c_2 + a^2 b_2 c \\
& + 3 a^2 c^2 - 8 a^3 b^2 - a^3 b b_1 + 2 a^3 b c_1 - a^3 b_1 c + 4 a^3 b^3 \\
& - 9 a^2 b_1 + 2 a^2 b_{11} - a^2 b_{12} + 2 a^2 b_2 + 4 a^2 c + 12 a^2 c_1 \\
& - a^2 c_{11} - 12 a^2 c_2 - a b b_1^2 - 22 a b b_1 c - 8 a b b_1 c_1 - a b b_1 c_2 \\
& + 4 a b b_{11} c - 2 a b b_{12} c + 12 a b b_2 c + 7 a b b_2 c_1 - a b c c_1 \\
& - a b c c_{11} - 4 a b c c_2 + a b c_1^2 + 5 a b_1^2 c - 4 a b_1 b_2 c - a b_1 c^2 \\
& - 3 a b_1 c c_1 + a b_1 c c_2 + 2 a b_{11} c^2 - a b_{12} c^2 + 2 a b_2 c^2 + a b_2 c c_1 \\
& - a c^2 c_1 - a_1^2 b c + 2 a_1 a^2 b^2 - 2 a_1 a^2 b c + 6 a_1 a^3 b^2 - 2 a_1 a^3 b c \\
& + 10 a_1 b^3 - 2 a_1 b^2 b_1 + 3 a_1 b^2 b_2 + 11 a_1 b^2 c + 6 a_1 b^2 c_1 + 8 a_1 b^2 c_2 \\
& - 7 a_1 b b_1 c - 4 a_1 b b_2 c + 4 a_1 b c^2 + 2 a_1 b c c_1 - a_1 b_1 c^2 + a_1 b_2 c^2 \\
& + 3 a_1 c^3 - 2 a^2 b^2 + 2 a^2 b c - 6 a^2 b^3 + a^2 b^2 b_1 - 4 a^2 b^2 c \\
& - 8 a^2 b^2 c_1 + 8 a^2 b b_1 c + 2 a^2 b c^2 - a^2 b_1 c^2 - 4 b^4 + b^3 b_1 - b^3 b_{11} \\
& - 8 b^3 c - 9 b^3 c_1 + b^3 c_{11} + b^2 b_1^2 + 11 b^2 b_1 c - 3 b^2 b_{11} c - 4 b^2 c^2 \\
& - 10 b^2 c c_1 + 2 b^2 c c_{11} - 6 b^2 c_1^2 + 2 b b_1^2 c + 11 b b_1 c^2 + 10 b b_1 c c_1 \\
& - 3 b b_{11} c^2 - b c^2 c_1 + b c^2 c_{11} - 2 b c c_1^2 - 3 b_1^2 c^2 + b_1 c^3 + 2 b_1 c^2 c_1 \\
& - b_{11} c^3 + a^2 a_1 - a^2 a_2 + a^2 a_3 + a^2 b - 3 a^2 b_1 + 3 a^2 b_2 - 2 a^2 b_3 \\
& + a^2 c + 5 a a_1 b - a a_1 b_1 - 3 a a_1 c + a a_1^3 b + a a_1^3 c - 4 a a_2 b \\
& + a a_2 b_1 + 3 a a_2 c - a a_2^3 b - a a_2^3 c + 3 a a_3 b + a a_3 b_1 - 2 a a_3 b_2 \\
& + 2 a a_3 b_3 - 3 a a_3 c - a a_3 c_1 + a a_3 c_2 - 4 a b^2 + a b b_1 - 2 a b b_2 \\
& + 3 a b b_3 - a b b_{11} - 7 a b c - 6 a b c_1 + a b c_{12} + 4 a b c_2 - a b c_{22} \\
& + a b_1^2 + a b_1 b_2 + 8 a b_1 c + a b_1 c_1 + a b_1 c_2 - 2 a b_2^2 + 2 a b_2 b_3 \\
& - 8 a b_2 c - a b_2 c_1 - a b_2 c_2 + 3 a b_3 c + 2 a b_3 c_2 - a b_{11} c - 3 a c^2 \\
& + a c c_1 + a c c_{12} - 2 a c c_2 - a c c_{22} - a c_1 c_2 + a c_2^2 + a_1 a_2 c \\
& - 6 a_1 a^3 b - 5 a_1 b^2 - 4 a_1 b b_2 + 2 a_1 b b_3 - 3 a_1 b c - a_1 b c_1 \\
& - 7 a_1 b c_2 + a_1 b_1 c + 2 a_1 b_2 c + 2 a_1 b_3 c + 2 a_1 c^2 - a_1 c c_2 - a_{13} b^2 \\
& - 2 a_{13} b c - a_{13} c^2 - a_2^2 c + 5 a_2 a^3 b + a_2 a^3 c + 4 a_2 b^2 + 3 a_2 b b_2 \\
& - 2 a_2 b b_3 + 2 a_2 b c + a_2 b c_1 + 6 a_2 b c_2 - 2 a_2 b_1 c - a_2 b_2 c \\
& - 2 a_2 b_3 c - 2 a_2 c^2 - a_2 c c_1 + 2 a_2 c c_2 + a_{23} b^2 + 2 a_{23} b c + a_{23} c^2 \\
& - 4 a_3^2 b - a_3 b^2 + 2 a_3 b b_1 - 4 a_3 b b_2 + 2 a_3 b c + 5 a_3 b c_1 \\
& - 10 a_3 b c_2 - 2 a_3 b_1 c + 4 a_3 b_2 c + 3 a_3 c^2 + a_3 c c_1 - 2 a_3 c c_2 + 3 b^3 \\
& + b^2 b_1 + 2 b^2 b_2 - b^2 b_3 + b^2 b_{11} + 8 b^2 c + 5 b^2 c_1 - b^2 c_{12} - b^2 c_2 \\
& + b^2 c_{22} - 2 b b_1 b_3 - 4 b b_1 c + b b_1 c_1 + 3 b b_1 c_2 + 8 b b_2 c \\
& + 3 b b_2 c_1 - 6 b b_2 c_2 - 2 b b_3 c - 2 b b_3 c_1 + 2 b b_{11} c + 7 b c^2 \\
& + 4 b c c_1 - 2 b c c_{12} + 2 b c c_2 + 2 b c c_{22} + b c_1^2 + 6 b c_1 c_2 - 6 b c_2^2 \\
& - b_1^2 c - 4 b_1 b_2 c - 2 b_1 b_3 c - 5 b_1 c^2 - b_1 c c_1 - b_1 c c_2 + 4 b_2^2 c \\
& + 6 b_2 c^2 - b_2 c c_1 + 2 b_2 c c_2 - b_3 c^2 - 2 b_3 c c_1 + b_{11} c^2 + 2 c^3 - c^2 c_1 \\
& - c^2 c_{12} + 3 c^2 c_2 + c^2 c_{22} + 2 c c_1 c_2 - 2 c c_2^2 - a a_1 + a a_2 - a a_3 \\
& + a b_1 - a b_2 + a c_1 - a c_2 + a_1 a_3 + a_1 b + a_1 b_2 + a_1 c + a_1 c_2
\end{aligned}$$

$$\begin{aligned}
& -a_2 a_3 - a_2 b - a_2 b_2 - a_2 c - a_2 c_2 + a_3^2 + a_3 b - a_3 b_1 + 2 a_3 b_2 \\
& + a_3 c - a_3 c_1 + 2 a_3 c_2 - b b_1 + b b_2 - b c_1 + b c_2 - b_1 b_2 - b_1 c \\
& - b_1 c_2 + b_2^2 + b_2 c - b_2 c_1 + 2 b_2 c_2 - c c_1 + c c_2 - c_1 c_2 + c_2^2 \}
\end{aligned}$$

We do the same without taking double derivatives two times. Now we get only five syzygies. They can be viewed in the "results"-subsection below

```

> A := Pullback(T2, I1) : B := Pullback(T2, I2) : C := Pullback(T2, I3) :
> for i from 1 to 3 do
  A || i := Pullback(T3, D || i(A)); B || i := Pullback(T3, D || i(B)); C || i := Pullback(T3,
    D || i(C));
  od:
> for k from 1 to 3 do
  for j from k to 3 do
    A || k || j := Pullback(T4, D || j(D || k(A))); B || k || j := Pullback(T4, D || j(D || k(B)));
    C || k || j := Pullback(T4, D || j(D || k(C)));
  od:od:
> eq1 := eliminate( {seq(seq(A || k || j - a || k || j, j = k..3), k = 1..3), seq(seq(B || k || j - b
  || k || j, j = k..3), k = 1..3), seq(seq(C || k || j - c || k || j, j = k..3), k = 1..3) }, {u[1,
  1, 1, 1], u[1, 1, 1, 2], u[1, 1, 1, 3], u[1, 1, 2, 2], u[1, 1, 2, 3], u[1, 2, 2, 2], u[1,
  2, 2, 3], u[2, 2, 2, 2], u[2, 2, 2, 3], v[1, 1, 1, 1], v[1, 1, 1, 2], v[1, 1, 1, 3], v[1, 1,
  2, 2], v[1, 1, 2, 3], v[1, 2, 2, 2], v[1, 2, 2, 3], v[2, 2, 2, 2], v[2, 2, 2, 3] } ) [2] :
> nops(invariants4); nops(eq1); nops( {u[1, 1, 1, 1], u[1, 1, 1, 2], u[1, 1, 1, 3], u[1, 1,
  2, 2], u[1, 1, 2, 3], u[1, 2, 2, 3], u[1, 2, 2, 2], u[2, 2, 2, 2], u[2, 2, 2, 3], v[1, 1, 1,
  1], v[1, 1, 1, 2], v[1, 1, 1, 3], v[1, 1, 2, 2], v[1, 1, 2, 3], v[1, 2, 2, 2], v[1, 2, 2, 3],
  v[2, 2, 2, 2], v[2, 2, 2, 3] } );
1
5
18 (7.1.11)
> fourjets := {seq(seq(seq(seq(op( [u[i1, i2, i3, i4], v[i1, i2, i3, i4]] ), i4 = i3..3), i3 = i2
  ..3), i2 = i1..3), i1 = 1..3) } : nops(%)
30 (7.1.12)
> tmpp := { } :for j to nops(eq1) do for i to nops(fourjets) do tmpp := tmpp
  union {diff(eq1[j], fourjets[i]) } :od:od: tmpp
{0} (7.1.13)
> eq2 := eliminate( {op(simplify(eq1)), seq(A || i - a || i, i = 1..3), seq(B || i - b || i, i = 1
  ..3), seq(C || i - c || i, i = 1..3) }, {u[1, 1, 1], u[1, 1, 2], u[1, 1, 3], u[1, 2, 2], u[1,
  2, 3], u[2, 2, 2], u[2, 2, 3], v[1, 1, 1], v[1, 1, 2], v[1, 1, 3], v[1, 2, 2], v[1, 2, 3],
  v[2, 2, 2], v[2, 2, 3] } ) [2] :
> smpleq2 := simplify(eq2) :
> threejets := {seq(seq(seq(op( [u[i1, i2, i3], v[i1, i2, i3]] ), i3 = i2..3), i2 = i1..3), i1
  = 1..3) } : nops(%)
20 (7.1.14)
> tmpp := { } :for j to nops(eq2) do for i to nops(threejets) do tmpp := tmpp
  union {diff(eq2[j], threejets[i]) } :od:od: tmpp
{0} (7.1.15)
> nops(smpleq2)
5 (7.1.16)
> eq3 := eliminate( {op(smpleq2), A - a, B - b, C - c}, {u[1, 1], u[1, 2], u[1, 3],
  u[2, 2], u[2, 3], v[1, 1], v[1, 2], v[1, 3], v[2, 2], v[2, 3] } ) [2] :

```



## Results

> eq3[2]

$$a^2 - a a l + 2 a b - a l b - a l l b - a + a l 2 + a l 3 - a 2 2 + 2 a 3 + b + c \quad (7.1.2.1)$$

> eq3[3]

$$a^4 b - a^4 b l + a^4 b 2 + a^3 a l b - a^3 a 2 b + 2 a^3 b^2 - a^3 b b l - a^3 b b l l \quad (7.1.2.2)$$

$$\begin{aligned} & + a^3 b b l 2 - a^3 b c l + a^3 b l^2 - a^3 b l b 2 + a^3 b l c - 4 a^2 a l b^2 \\ & + 2 a^2 a l b b l - 2 a^2 a l b b 2 - a^2 a l b c + 2 a^2 a 2 b^2 - 2 a^2 b^2 b l \\ & - 3 a^2 b^2 c l - a^2 b^2 c l l + a^2 b b l c + a^2 b b l c l + a^2 b b l l c - a^2 b l^2 c \\ & - a a l^2 b^2 + 4 a a l b^3 + a a l b^2 b l + 4 a a l b^2 c + 4 a a l b^2 c l \\ & - 3 a a l b b l c - 2 a l^2 b^3 - 2 a l^2 b^2 c - 2 a^3 b + 2 a^3 b l - 2 a^3 b 2 - a^3 c \\ & + a^3 c l - a^3 c 2 - a^2 a l b - 2 a^2 a l c + a^2 a l 3 b + a^2 a 2 b + 2 a^2 a 2 c \\ & - a^2 a 2 3 b + 2 a^2 a 3 b - a^2 a 3 b l + a^2 a 3 b 2 - a^2 b b l + a^2 b b l l \\ & + 2 a^2 b b 2 - a^2 b b 2 2 + a^2 b c + 2 a^2 b c l + a^2 b c l 2 - a^2 b c 2 - a^2 b c 2 2 \\ & - a^2 b l^2 - 5 a^2 b l c - a^2 b l c l + a^2 b l l c - a^2 b l 2 c + a^2 b 2^2 + 5 a^2 b 2 c \\ & + a^2 b 2 c 2 + a^2 c^2 - 2 a^2 c c l + 2 a^2 c c 2 + a a l a 2 b - a a l a 3 b \\ & + 3 a a l b^2 - a a l b b l + 8 a a l b c - 2 a a l b c 2 - a a l b l c \\ & + 2 a a l b 2 c + 5 a a l c^2 - a a 2^2 b + 2 a a 2 a 3 b - a a 2 b^2 - 2 a a 2 b b l \\ & + 3 a a 2 b b 2 - 4 a a 2 b c - 2 a a 2 b c l + 4 a a 2 b c 2 - a a 2 b 2 c \\ & - 3 a a 2 c^2 - a a 3 b b l - 2 a a 3 b c l + a a 3 b l c + 2 a b^3 - a b^2 b l \\ & - a b^2 b l l + a b^2 b l 2 + 2 a b^2 b 2 + 4 a b^2 c - 4 a b^2 c l + a b^2 c l l \\ & + 4 a b^2 c 2 + 2 a b b l^2 - 2 a b b l b 2 + 3 a b b l c + a b b l c l - a b b l c 2 \\ & - 3 a b b l l c + 2 a b b l 2 c - a b b 2 c l + 2 a b c^2 - 3 a b c c l + a b c c l l \\ & + 4 a b c c 2 - a b c l^2 + 3 a b l^2 c - 2 a b l b 2 c + 4 a b l c^2 + 3 a b l c c l \\ & - a b l c c 2 - 2 a b l l c^2 + a b l 2 c^2 - 2 a b 2 c^2 - a b 2 c c l + a c^2 c l \\ & + a l^2 b^2 + a l^2 b c + 2 a l a 2 b^2 + 2 a l a 2 b c + 2 a l a 3 b^2 + 2 a l a 3 b c \\ & - 2 a l b^3 - a l b^2 b l - a l b^2 b 2 - 7 a l b^2 c - 2 a l b^2 c l - 2 a l b b 2 c \\ & - 8 a l b c^2 - 2 a l b c c l + a l b l c^2 - a l b 2 c^2 - 3 a l c^3 - 2 a 2^2 b^2 \\ & - 2 a 2^2 b c - 2 a 2 b^3 + a 2 b^2 b l - 4 a 2 b^2 c + 2 a 2 b b l c - 2 a 2 b c^2 \\ & + a 2 b l c^2 + b^3 c l - b^3 c l l - b^2 b l c + 2 b^2 b l c l + b^2 b l l c + 2 b^2 c c l \\ & - 2 b^2 c c l l + 2 b^2 c l^2 - 2 b b l^2 c - 2 b b l c^2 + 2 b b l l c^2 + b c^2 c l \\ & - b c^2 c l l + 2 b c c l^2 - 2 b l^2 c^2 - b l c^3 - 2 b l c^2 c l + b l l c^3 + a^2 b \\ & - a^2 b l + a^2 b 2 + a^2 c - a^2 c l + a^2 c 2 - a a l 3 b - a a l 3 c + a a 2 3 b \\ & + a a 2 3 c - 2 a a 3 b + a a 3 b l - a a 3 b 2 - 2 a a 3 c + a a 3 c l - a a 3 c 2 \\ & - 2 a b^2 + 2 a b b l - a b b l 2 - 2 a b b 2 + a b b 2 2 - 4 a b c + 2 a b c l \\ & - a b c l 2 - 2 a b c 2 + a b c 2 2 + a b l b 2 + 2 a b l c + a b l c 2 - a b l 2 c \\ & - a b 2^2 - 2 a b 2 c + a b 2 c l - 2 a b 2 c 2 + a b 2 2 c - 2 a c^2 + 2 a c c l \\ & - a c c l 2 - 2 a c c 2 + a c c 2 2 + a c l c 2 - a c 2^2 - a l a 2 b - a l a 2 c \\ & + a l b b 2 + a l b c 2 + a l b 2 c + a l c c 2 + a l 3 b^2 + 2 a l 3 b c + a l 3 c^2 \\ & + a 2^2 b + a 2^2 c - a 2 a 3 b - a 2 a 3 c + a 2 b b l - 2 a 2 b b 2 + a 2 b c l \end{aligned}$$

$$\begin{aligned}
& -2 a^2 b c^2 + a^2 b l c - 2 a^2 b^2 c + a^2 c c l - 2 a^2 c c^2 - a^2 b^3 \\
& -2 a^2 b^3 c - a^2 b^3 c^2 + 2 a^3 b^2 - a^3 b b l + 2 a^3 b b^2 + 4 a^3 b c - a^3 b c l \\
& + 2 a^3 b c^2 - a^3 b l c + 2 a^3 b^2 c + 2 a^3 c^2 - a^3 c c l + 2 a^3 c c^2 + b^3 \\
& - b^2 b l + b^2 b l^2 + b^2 b^2 - b^2 b^2 c + 3 b^2 c - b^2 c l + b^2 c l^2 + b^2 c^2 \\
& - b^2 c^2 c - 2 b b l b^2 - 2 b b l c - 2 b b l c^2 + 2 b b l^2 c + 2 b b^2 \\
& + 2 b b^2 c - 2 b b^2 c l + 4 b b^2 c^2 - 2 b b^2 c^2 c + 3 b c^2 - 2 b c c l \\
& + 2 b c c l^2 + 2 b c c^2 - 2 b c c^2 c - 2 b c l c^2 + 2 b c^2 - 2 b l b^2 c - b l c^2 \\
& - 2 b l c c^2 + b l^2 c^2 + 2 b^2 c^2 + b^2 c^2 - 2 b^2 c c l + 4 b^2 c c^2 - b^2 c^2 \\
& + c^3 - c^2 c l + c^2 c l^2 + c^2 c^2 - c^2 c^2 c - 2 c c l c^2 + 2 c c^2
\end{aligned}$$

> eq3[4]

$$\begin{aligned}
& a^4 b l - a^4 b^2 - 2 a^3 a l b + a^3 a^2 b + 2 a^3 b^2 - 2 a^3 b c - a^3 b c l - a^3 b l^2 \quad (7.1.2.3) \\
& + a^3 b l b^2 - a^3 b l c - a^2 a l b^2 + 2 a^2 a l b b l + 3 a^2 a l b c - a^2 a^2 b b l \\
& - 2 a^2 b^2 b l - 4 a^2 b^2 c - 5 a^2 b^2 c l - a^2 b^2 c l^2 + 2 a^2 b b l c + a^2 b l^2 c \\
& + a a l b^2 b l + 8 a a l b^2 c + 4 a a l b^2 c l - 3 a a l b b l c - 4 a l^2 b^2 c \\
& + a^3 a l - a^3 a^2 + a^3 a^3 - 3 a^3 b l + 3 a^3 b^2 + a^3 c^3 + 5 a^2 a l b - a^2 a l b l \\
& - 3 a^2 a l c - 3 a^2 a^2 b + a^2 a^2 b l + 3 a^2 a^2 c + a^2 a^3 b - a^2 a^3 b^2 \\
& - 3 a^2 a^3 c - 4 a^2 b^2 + a^2 b b l - a^2 b b^2 - a^2 b c + a^2 b c l^2 + a^2 b c l^3 \\
& - a^2 b c^2 c + 2 a^2 b c^3 + 2 a^2 b l^2 - a^2 b l b^2 + 9 a^2 b l c + a^2 b l c^2 \\
& - a^2 b l c^3 - a^2 b^2 c^2 - 7 a^2 b^2 c - a^2 b^2 c^2 + 2 a^2 c^2 + a^2 c c l - 2 a a l a^3 b \\
& - a a l b^2 - 3 a a l b b l - 2 a a l b b^2 - 16 a a l b c - a a l b c l \\
& - 4 a a l b c^2 - a a l b c^3 + 3 a a l b l c + 3 a a l c^2 + a a^2 a^3 b + a a^2 b^2 \\
& + 2 a a^2 b b l + a a^2 b b^2 + 10 a a^2 b c + 4 a a^2 b c^2 - 4 a a^2 b l c \\
& + a a^2 b^2 c - 3 a a^2 c^2 + 2 a a^3 b^2 - a a^3 b b l - 6 a a^3 b c - 3 a a^3 b c l \\
& + 2 a a^3 b l c + 2 a b^3 + 2 a b^2 b l + 2 a b^2 b^2 + 6 a b^2 c - 4 a b^2 c l \\
& + a b^2 c l^2 + 8 a b^2 c^2 + 4 a b b l c + 5 a b b l c l - a b b l c^2 - 4 a b b^2 c \\
& - 3 a b b^2 c l + 2 a b c^2 + 7 a b c c l + a b c c l^2 - 6 a b l^2 c + 4 a b l b^2 c \\
& - 10 a b l c^2 - a b l c c l - a b l c c^2 + 2 a b^2 c^2 + a b^2 c c l - 2 a c^3 \\
& - a c^2 c l + a l^2 b c + 4 a l a^2 b c - a l a^3 b^2 + 7 a l a^3 b c - a l b^3 \\
& - a l b^2 b^2 + 9 a l b^2 c - 4 a l b^2 c l - 4 a l b^2 c^2 + 2 a l b b l c \\
& + 6 a l b b^2 c + 9 a l b c^2 + 4 a l b c c^2 - 2 a l b l c^2 - a l b^2 c^2 - a l c^3 \\
& - 4 a^2 b^2 c - 8 a^2 b^2 c + 4 a^2 b^2 c l - 4 a^2 b b l c - 8 a^2 b c^2 - 4 a^2 b c c l \\
& + 4 a^2 b l c^2 - 4 b^3 c + 3 b^3 c l - b^3 c l^2 - 4 b^2 b l c + b^2 b l c l - 8 b^2 c^2 \\
& - 2 b^2 c c l - 2 b^2 c c l^2 + 4 b^2 c l^2 - 6 b b l c c l - 4 b c^3 - 5 b c^2 c l \\
& - b c^2 c l^2 + 4 b l^2 c^2 + 4 b l c^3 + b l c^2 c l - 2 a^2 a l + 2 a^2 a^2 - 2 a^2 a^3 \\
& + 3 a^2 b l - 3 a^2 b^2 + a^2 c l - a^2 c^2 - a^2 c^3 + a a l a^3 - 2 a a l b + a a l b l \\
& + a a l b^2 + 6 a a l c + a a l c^2 - a a^2 a^3 + a a^2 b - a a^2 b l - a a^2 b^2 \\
& - 6 a a^2 c - a a^2 c^2 + a a^3 - a a^3 b l + 3 a a^3 b^2 + 6 a a^3 c + a a^3 c^2 \\
& + a a^3 c^3 + 2 a b^2 - 2 a b b l + 2 a b b^2 + 3 a b c + 3 a b c l - a b c l^2 \\
& - a b c l^3 - 2 a b c^2 + a b c^2 c + a b c^3 - a b l^2 - a b l b^2 - 9 a b l c
\end{aligned}$$

$$\begin{aligned}
& -a b l c l - a b l c 2 + 2 a b 2^2 + 8 a b 2 c + 2 a b 2 c 2 + a b 2 c 3 + a c^2 \\
& -4 a c c l - a c c l 2 - a c c l 3 + 4 a c c 2 + a c c 2 2 + a c c 3 + a c 2 c 3 \\
& -a l a 2 c + 3 a l a 3 b - 3 a l a 3 c + 3 a l b^2 + 3 a l b b 2 - a l b c + a l b c l \\
& + 5 a l b c 2 + a l b c 3 - a l b l c - 3 a l b 2 c - 4 a l c^2 - a l c c 2 + a l c c 3 \\
& + a 2^2 c - 2 a 2 a 3 b + 2 a 2 a 3 c - 2 a 2 b^2 - 2 a 2 b b 2 + 2 a 2 b c - a 2 b c l \\
& - 4 a 2 b c 2 - a 2 b c 3 + 2 a 2 b l c + 2 a 2 b 2 c + 4 a 2 c^2 + a 2 c c l \\
& - a 2 c c 3 + a 3^2 b - 3 a 3^2 c - a 3 b^2 + a 3 b b 2 - 6 a 3 b c - 2 a 3 b c l \\
& + 5 a 3 b c 2 + 4 a 3 b l c - 7 a 3 b 2 c - 5 a 3 c^2 + 2 a 3 c c l - 3 a 3 c c 2 \\
& - 2 b^3 - 2 b^2 b 2 - 5 b^2 c - 3 b^2 c l + b^2 c l 2 + b^2 c l 3 - b^2 c 2 2 + 6 b b l c \\
& - b b l c l - 2 b b l c 2 - b b l c 3 - 8 b b 2 c - 2 b b 2 c l + 4 b b 2 c 2 - 4 b c^2 \\
& + 2 b c c l 2 + 2 b c c l 3 - 4 b c c 2 - 2 b c c 2 2 - b c l^2 - 4 b c l c 2 - b c l c 3 \\
& + 4 b c 2^2 + b l^2 c + 4 b l b 2 c + 6 b l c^2 + b l c c l + 2 b l c c 2 - b l c c 3 \\
& - 4 b 2^2 c - 6 b 2 c^2 + 2 b 2 c c l - 4 b 2 c c 2 - c^3 + 3 c^2 c l + c^2 c l 2 + c^2 c l 3 \\
& - 4 c^2 c 2 - c^2 c 2 2 - c c l c 3 + a a l - a a 2 + a a 3 - a b l + a b 2 - a c l \\
& + a c 2 - a l a 3 - a l b - a l b 2 - a l c - a l c 2 + a 2 a 3 + a 2 b + a 2 b 2 \\
& + a 2 c + a 2 c 2 - a 3^2 - a 3 b + a 3 b l - 2 a 3 b 2 - a 3 c + a 3 c l - 2 a 3 c 2 \\
& + b b l - b b 2 + b c l - b c 2 + b l b 2 + b l c + b l c 2 - b 2^2 - b 2 c + b 2 c l \\
& - 2 b 2 c 2 + c c l - c c 2 + c l c 2 - c 2^2
\end{aligned}$$

> eq3[5]

$$\begin{aligned}
& a^4 b + a^4 b l - a^4 b 2 - a^3 a l b + a^3 a 2 b - 2 a^3 b b l + a^3 b b l l - a^3 b b l 2 \quad (7.1.2.4) \\
& + a^3 b c l - a^3 b l^2 + a^3 b l b 2 - a^3 b l c + 4 a^2 a l b^2 - 2 a^2 a l b b l \\
& + 2 a^2 a l b b 2 + a^2 a l b c - 2 a^2 a 2 b^2 - 4 a^2 b^3 + a^2 b^2 b l - a^2 b^2 b l l \\
& + 3 a^2 b^2 c l + a^2 b^2 c l l + a^2 b b l^2 - a^2 b b l c - a^2 b b l c l - a^2 b b l l c \\
& + a^2 b l^2 c + a a l^2 b^2 + 4 a a l b^3 - a a l b^2 b l - 4 a a l b^2 c - 4 a a l b^2 c l \\
& + 3 a a l b b l c - 2 a l^2 b^3 + 2 a l^2 b^2 c - 2 a^3 b + a^3 b 3 - a^3 c - a^3 c l \\
& + a^3 c 2 - 2 a^2 a l b + 2 a^2 a l c - a^2 a l 3 b + a^2 a 2 b - 2 a^2 a 2 c + a^2 a 2 3 b \\
& - a^2 a 3 b + a^2 a 3 b l - a^2 a 3 b 2 + 4 a^2 b^2 + 7 a^2 b b l - a^2 b b l l \\
& + a^2 b b l 2 + a^2 b b l 3 - 4 a^2 b b 2 + 2 a^2 b b 3 + 4 a^2 b c - a^2 b c l 2 \\
& + a^2 b c 2 + a^2 b c 2 2 - a^2 b l^2 + 2 a^2 b l b 2 - a^2 b l b 3 + 2 a^2 b l c \\
& + a^2 b l c l - a^2 b l l c + a^2 b l 2 c - a^2 b 2^2 - a^2 b 2 c - a^2 b 2 c 2 + a^2 c^2 \\
& + 2 a^2 c c l - 2 a^2 c c 2 - a a l a 2 b + a a l a 3 b - 13 a a l b^2 + 6 a a l b b l \\
& - 2 a a l b b 2 - a a l b b 3 + 2 a a l b c 2 + a a l b l c - 2 a a l b 2 c \\
& - 5 a a l c^2 + a a 2^2 b - 2 a a 2 a 3 b + 9 a a 2 b^2 - 4 a a 2 b b l + a a 2 b b 2 \\
& + 2 a a 2 b c l - 4 a a 2 b c 2 + a a 2 b 2 c + 3 a a 2 c^2 - 8 a a 3 b^2 + a a 3 b b l \\
& + 2 a a 3 b c l - a a 3 b l c + 4 a b^3 - 5 a b^2 b l + 2 a b^2 b l l - a b^2 b l 2 \\
& - 2 a b^2 b 2 + 4 a b^2 c + 12 a b^2 c l - a b^2 c l l - 12 a b^2 c 2 - 3 a b b l^2 \\
& + 2 a b b l b 2 - 20 a b b l c - 7 a b b l c l + a b b l c 2 + 4 a b b l l c \\
& - 2 a b b l 2 c + 8 a b b 2 c + 5 a b b 2 c l - a b c c l - a b c c l l - 4 a b c c 2 \\
& + a b c l^2 + 2 a b l^2 c - 2 a b l b 2 c - 3 a b l c^2 - 3 a b l c c l + a b l c c 2
\end{aligned}$$

$$\begin{aligned}
& + 2 a b l l c^2 - a b l 2 c^2 + 2 a b 2 c^2 + a b 2 c c l - a c^2 c l - a l^2 b c \\
& + 2 a l a 2 b^2 - 2 a l a 2 b c + 6 a l a 3 b^2 - 2 a l a 3 b c + 10 a l b^3 \\
& - a l b^2 b l + 5 a l b^2 b 2 + 11 a l b^2 c + 6 a l b^2 c l + 8 a l b^2 c 2 \\
& - 6 a l b b l c - 2 a l b b 2 c + 4 a l b c^2 + 2 a l b c c l - a l b l c^2 + a l b 2 c^2 \\
& + 3 a l c^3 - 2 a 2^2 b^2 + 2 a 2^2 b c - 6 a 2 b^3 - a 2 b^2 b l - 4 a 2 b^2 c \\
& - 8 a 2 b^2 c l + 6 a 2 b b l c + 2 a 2 b c^2 - a 2 b l c^2 - 4 b^4 - b^3 b l - b^3 b l l \\
& - 8 b^3 c - 9 b^3 c l + b^3 c l l + b^2 b l^2 + 7 b^2 b l c - 2 b^2 b l c l - 3 b^2 b l l c \\
& - 4 b^2 c^2 - 10 b^2 c c l + 2 b^2 c c l l - 6 b^2 c l^2 + 4 b b l^2 c + 9 b b l c^2 \\
& + 8 b b l c c l - 3 b b l l c^2 - b c^2 c l + b c^2 c l l - 2 b c c l^2 - b l^2 c^2 + b l c^3 \\
& + 2 b l c^2 c l - b l l c^3 + a^2 a l - a^2 a 2 + a^2 a 3 + a^2 b - 2 a^2 b l + 2 a^2 b 2 \\
& - a^2 b 3 + a^2 c + 5 a a l b - a a l b l - 3 a a l c + a a l 3 b + a a l 3 c \\
& - 4 a a 2 b + a a 2 b l + 3 a a 2 c - a a 2 3 b - a a 2 3 c + 3 a a 3 b - a a 3 b 2 \\
& + a a 3 b 3 - 3 a a 3 c - a a 3 c l + a a 3 c 2 - 4 a b^2 - a b b l - a b b l 3 \\
& + a b b 3 - 7 a b c - 6 a b c l + a b c l 2 + 4 a b c 2 - a b c 2 2 + a b l^2 \\
& + 6 a b l c + a b l c l - a b l 3 c - a b 2^2 + a b 2 b 3 - 6 a b 2 c - a b 2 c l \\
& + a b 3 c + a b 3 c 2 - 3 a c^2 + a c c l + a c c l 2 - 2 a c c 2 - a c c 2 2 \\
& - a c l c 2 + a c 2^2 + a l a 2 c - 6 a l a 3 b - 5 a l b^2 - 5 a l b b 2 + a l b b 3 \\
& - 3 a l b c - a l b c l - 7 a l b c 2 + a l b l c + a l b 2 c + a l b 3 c + 2 a l c^2 \\
& - a l c c 2 - a l 3 b^2 - 2 a l 3 b c - a l 3 c^2 - a 2^2 c + 5 a 2 a 3 b + a 2 a 3 c \\
& + 4 a 2 b^2 + 4 a 2 b b 2 - a 2 b b 3 + 2 a 2 b c + a 2 b c l + 6 a 2 b c 2 \\
& - 2 a 2 b l c - a 2 b 3 c - 2 a 2 c^2 - a 2 c c l + 2 a 2 c c 2 + a 2 3 b^2 + 2 a 2 3 b c \\
& + a 2 3 c^2 - 4 a 3^2 b - a 3 b^2 + 3 a 3 b b l - 6 a 3 b b 2 + 2 a 3 b c + 5 a 3 b c l \\
& - 10 a 3 b c 2 - a 3 b l c + 2 a 3 b 2 c + 3 a 3 c^2 + a 3 c c l - 2 a 3 c c 2 + 3 b^3 \\
& + 2 b^2 b l + b^2 b l 3 + b^2 b 2 + 8 b^2 c + 5 b^2 c l - b^2 c l 2 - b^2 c 2 + b^2 c 2 2 \\
& + 2 b b l b 2 - b b l b 3 - 2 b b l c + b b l c l + 4 b b l c 2 + 2 b b l 3 c \\
& - 2 b b 2^2 + 6 b b 2 c + 4 b b 2 c l - 8 b b 2 c 2 - b b 3 c l + 7 b c^2 + 4 b c c l \\
& - 2 b c c l 2 + 2 b c c 2 + 2 b c c 2 2 + b c l^2 + 6 b c l c 2 - 6 b c 2^2 - b l^2 c \\
& - 2 b l b 2 c - b l b 3 c - 4 b l c^2 - b l c c l + b l 3 c^2 + 2 b 2^2 c + 5 b 2 c^2 \\
& - b 3 c c l + 2 c^3 - c^2 c l - c^2 c l 2 + 3 c^2 c 2 + c^2 c 2 2 + 2 c c l c 2 - 2 c c 2^2 \\
& - a a l + a a 2 - a a 3 + a b l - a b 2 + a c l - a c 2 + a l a 3 + a l b + a l b 2 \\
& + a l c + a l c 2 - a 2 a 3 - a 2 b - a 2 b 2 - a 2 c - a 2 c 2 + a 3^2 + a 3 b \\
& - a 3 b l + 2 a 3 b 2 + a 3 c - a 3 c l + 2 a 3 c 2 - b b l + b b 2 - b c l + b c 2 \\
& - b l b 2 - b l c - b l c 2 + b 2^2 + b 2 c - b 2 c l + 2 b 2 c 2 - c c l + c c 2 \\
& - c l c 2 + c 2^2
\end{aligned}$$

> eq3[1]

$$\begin{aligned}
& - 2 a a l c + 2 a c c l + 4 a^2 a l c - 2 a^2 c c l - 2 a^3 a l c - 2 a^3 c c l - 5 a a l c^2 \quad (7.1.2.5) \\
& + 4 a c^2 c l + 5 a^2 a l c^2 + a^2 c^2 c l + a^2 a l - a^2 c l - a^2 a 2 - a^2 b l + c c 2^2 \\
& - a^2 b l c l + a b b l^2 - a b c l^2 - a l a 2 b^2 - c c l c 2 + a^2 c c 2 - a b l 2 c^2 \\
& - a 2 c c 2 + a 2 b^2 b l - a^2 a l 3 b + a^2 a 2 3 b + 3 a^2 b c l - 4 a^2 b c 2
\end{aligned}$$

$$\begin{aligned}
& -8a^2a_2b^2 - 4aa_1b^3 - 2a^3bb_1 + a^3bb_{11} - a^3bb_{12} - a_3bb_1 \\
& -bb_1b_2 - 2bcc_1 - 2aa_3b - bbl^2c - 6bb_1c^2 + bcc_1^2 - ab^2b_{12} \\
& -aa_1b_2c - a_1bcc_1 - aa_2b_1c - 2abb_1b_2 - 2abb_{12}c \\
& + 5a^2bb_1c_1 - 3a^2bb_{11}c + 2a^2a_1bb_2 - a^2b - b^2b_1 + bb_2^2 \\
& - 3a^4b + a_1^2b^3 + 3a^3b + a_2^2b^2 - a_2b^3 - c^3 + b_2a^5 - a_3^2a - b_2^2a \\
& - c_2^2a + b_2^2a^2 - c_2^2a^2 + b_2a^2 + c_2a^2 + a_3a^2 - a_3a^3 - 2b_2a^3 \\
& + c_1a^4 - c_2a^4 + a_2a^3 - b_3a^3 + b_3a^2 + b_2a_3a^2 + c_1a_3a^2 - c_2a_3a^2 \\
& + c_1b_2a^2 + c_2c_1a^2 + a_3a_2a + b_2a_2a + c_2a_2a - 2b_2a_3a + c_1a_3a \\
& - 2c_2a_3a + c_1b_2a - 2c_2b_2a + c_2c_1a - b_3a_3a - b_3b_2a - c_2b_3a \\
& + 12a^3c^2 + a^3c^2 + 2a_1c^3 - a^2c - a^4c + 2a^3c + 2a^2c^2 - c^2c_1 - 9a^2c^2 \\
& + a_1c^2 - aa_1b_2 + a^2a_1b_1 + 2a^3b_1 - a^3a_1 - a^5b_1 + 4a^3b^3 + 4ab^4 \\
& - 2a_1b^4 + a^5b - a^4b^2 + a^3b_2^2 + a^4b_1^2 - 4b_2c^3 - 2c^3c_1 - a_3c^2 \\
& - b_2c^2 - c^2c_{23} - 4a_2c^3 + b_{12}c^3 + a_{13}b^3 + b^3b_{12} - 2b^3b_2 + 2b^3c_2 \\
& - a_3b^2 - b^2b_{23} - b^2c_{23} + 4a^3b^2 - 5a^2b^2 + 3ab^3 - a_1b^3 - 8b^3c \\
& + b^3c_1 - 18b^2c^2 + b^2c_1^2 - 16bc^3 + a_3^2c - a^3c_3 + a^2c_3 + 2ab^2 \\
& + a_1b^2 - a_2b^2 + a_3^2b + a_3b^2 - 3b^2c - b^2c_1 - 3bc^2 + bc_2^2 + a_3c^2 \\
& - b_1c^2 + b_2^2c - b_1^2c^2 - 3b_1c^3 - a^2b_1^2 + a^3b_1^2 - a_2c^2 - 2a^3a_1bb_2 \\
& - a^3a_1bc + a^3bb_1c + a^3bb_1c_1 + a^3bb_{11}c - 2bb_1b_2c \\
& + 2bb_1cc_2 - 4bb_2cc_1 + 6abb_2c_2 - 2abb_3c + abb_3c_1 \\
& + 2abcc_{12} - 2abcc_{22} + 2abcc_3 - 4abcl_2c + abcl_3c \\
& + a_1bb_3c - a_1bcc_3 - a_2a_3bc - 4a_2bb_2c - a^3b_1c_1 + 2a_3b_1c^2 \\
& - b_1b_2c^2 + b_1c^2c_2 - 2b_2c^2c_1 + 3a^2b_3c + a^2b_{12}c^2 - 2a^2b_2c^2 \\
& + acc_{23} + a^2cc_3 + a_1a_3c^2 - aa_2c^2 - 3aa_3c^2 - 2ab_3c^2 + a^2c_1c_2 \\
& - a^2c^2c_2 - a^2c^2c_{22} + 2acc_2^2 + a_3b_3c + a_3cc_3 + b_2b_3c + b_2cc_3 \\
& + b_3cc_2 + cc_2c_3 + aa_3c - 3aa_1c^3 - ab_1c^3 + ab_{11}c^3 - a^3b_1^2c \\
& + a_1b_3c^2 - a^4b_1b_2 + a^3a_3b_2 + a^3b_2c_2 + ab_{23}c - a^2bc_1^2 \\
& + 2aa_2b^3 + 2ab^3b_1 + 8ab^3c + 5ab^3c_1 - ab^3c_{11} + 4ab^2c^2 \\
& + 4ab^2c_1^2 - a_1b^3b_1 - 4a_1b^3c - 2a_1b^2c^2 - a^3a_2b + 6a^3bb_2 \\
& - 2a^3bb_3 + a^3bc_{12} - a^3bc_2 - a^3bc_{22} + a^3a_{13}b - 2a^2a_1b^3 \\
& + a^4a_1b - a^4a_2b - a^4bb_1 - a^4bb_{11} + a^4bb_{12} - a^4bcl - 2a^3a_1b^2 \\
& + 2a^3a_2b^2 - 3a^3b^2c_1 - a^3b^2c_{11} - a^2a_1^2b^2 - 2b^2b_2c_1 + 4b^2cc_2 \\
& + 3bb_{12}c^2 - 10bb_2c^2 + 2bc^2c_2 - aa_2b^2 + 3aa_3^2b + ab^2c_{12} \\
& - ab^2c_{22} + 2ab^2c_3 + 3a^3b_2c - 3a^2a_2c^2 + a_3bb_3 + a_3bc_3 \\
& - 2a_3b_3c + bb_2b_3 + bb_2c_3 - 2bb_{23}c + bb_3c_2 - 2bcc_{23} \\
& + bc_2c_3 + aa_3b + abb_{23} + abc_{23} - a_2a_3b^2 - 2a_2b^2b_2 \\
& + a_3b^2b_1 - a_3b^2c_1 - b^2b_1b_2 + b^2b_1c_2 + 3b^2b_{12}c - 8b^2b_2c \\
& + 2abb_2^2 + 4abb_2c^2 - a_1b^2c_3 + 2a_{13}b^2c + a_{13}bc^2 - a^2a_3b \\
& - a^2bb_{23} - a^2bc_{23} + a^2a_{13}b^2 - a^2a_2^2b + 6a^2a_3b^2 + 2a^2b^2b_{12} \\
& + 10a^2b^2c_2 - 6a^2bc^2 + 2a^3cc_2 - a^2cc_{12} + a^2cc_{22} + aa_2^2c
\end{aligned}$$

$$\begin{aligned}
& + a^4 b l c + 2 a^3 a 2 c + a^2 a 2 3 c + 2 a^2 b l c^2 - 2 a^2 b l 1 c^2 - a^2 a l 3 c \\
& + a^3 b l 1 c - a^3 b l 2 c - a a l b b 3 - 2 a a 3 c + a l b 2 c + a l c c 2 - a 2 a 3 c \\
& - a 2 b 2 c + 2 b 2 c c 2 + 7 a a 2 c^2 + 2 a b l^2 c - b^3 - 6 a^2 b^3 - 3 a a 2 a 3 b \\
& + a a 2 b b l - 4 a^2 a l b b l + 3 a^2 a l b c + 2 a^2 a 2 b b l + 6 a^2 b b l c \\
& + a a l b^2 b l - 2 a a l b l c + 3 a a 2 b l c - 2 a a 3 b l c + 2 a b l c c l \\
& - 2 a b l c c 2 - 5 a a l b^2 c - 4 a a l b^2 c l - 2 a a 2 b b 2 + 6 a a 2 b c \\
& - 4 a a 2 b c 2 - 4 a a 3 b b l - a a 3 b c - 3 a a 3 b c l + 8 a b b l c \\
& - 4 a b b l c 2 + 8 a b b 2 c - 2 a b b 2 c l - a l a 2 b c - a l a 3 b c \\
& + a l b b l c + 2 a l b b 2 c - 2 a l b c c 2 + 2 a 2 b c c l + 4 a a l a 3 b \\
& - a a l b b l + 3 a a l b b 2 - a a l b c + a a l b c l + 5 a a l b c 2 - b^4 \\
& + a^2 b l b 3 - a^2 b^2 b l 1 + 2 a^2 b b l^2 - a b b 3 - a b 3 c - 5 c^4 - a a l a 2 c \\
& + a a l c c 2 + a a 2 c c l - a^2 a l b l c + 2 a^2 a l b 2 c + 3 a^2 b l c c l \\
& - a^2 a 2 b 2 c + a^2 a 3 b l c - a^2 b l c c 2 - a^2 b 2 c c l - a a l b 2 c^2 \\
& + a a 2 b l c^2 - 2 a b l c^2 c l - a a 2 a 3 c - 2 a a 2 c c 2 - a a 3 c c l \\
& + 2 a a 3 c c 2 - a b l b 3 c - a b l c c 3 + 2 a b 2 c c 2 - 2 a c c l c 2 \\
& - 2 a 2 b 2 c^2 - a^3 a 3 b l - a c 2 c 3 - a a 3 c 3 - a b 2 c 3 + 2 a a 2 c \\
& + 2 a b l c + a a 3 b l - a a l a 3 + 4 a a l b b l c - 3 a^2 a l b b l c \\
& + 2 a a l a 2 b c + 2 a a l a 3 b c - 2 a a l b c c l - 2 a a 2 b b l c \\
& - 4 a b b l c c l + 8 a b l c^2 + 3 a b 2 c^2 + a l b l c^2 + 2 a l b 2 c^2 - a 2 b l c^2 \\
& - b l c^2 c l - a^2 b l^2 c - 4 a^2 a 2 c + 4 a^2 a 3 c - 7 a^2 b l c + 3 a^2 b 2 c \\
& - a^3 b l c - a 3 b l c + 2 a 3 b 2 c - a 3 c c l + 2 a 3 c c 2 - b l b 2 c - b l c c 2 \\
& - b 2 c c l - a a l c 2 + a b l b 2 + a b l c 2 - 2 a^3 b l b 2 - a^2 a 2 b l - b c l c 2 \\
& + 2 a b b l - a b b 2 + 4 a b c - a^2 a 2 b b 2 - 6 a^2 a 2 b c - 2 a^2 a 2 b c l \\
& + 4 a^2 a 2 b c 2 - 2 a^2 a 3 b c l - 3 a^2 b b l b 2 + 3 a^2 b b l 2 c - 8 a^2 b b 2 c \\
& - 5 a^2 b b 2 c l - 3 a^2 b c c l + a^2 b c c l 1 + a^2 a l a 2 b + 2 a^3 a l b b l \\
& + 4 a^2 a l b^2 c + 4 a^2 a l b^2 c l - 2 a a l^2 b^2 c + a a l^2 b c - 3 a a l a 3 b^2 \\
& + 2 a b c l - a b c 2 - a b c 3 + a l a 3 b - a b 2 c - a c c 2 - b b l c 2 \\
& - 2 a a l b + 2 a a 2 b + 4 a a l b^2 - a a 2 b^2 + 2 a a 3 b^2 + 5 a b^2 b 2 \\
& + 18 a b^2 c - 4 a b^2 c l + a b^2 c 2 + 27 a b c^2 - a l a 3 b^2 - a l b^2 c l \\
& - 2 a l b^2 c 2 + 3 a l b c^2 + a 2^2 b c - 6 a 2 b^2 c + 2 a 2 b^2 c l - 9 a 2 b c^2 \\
& - 3 b^2 b l c + b^2 b l c l - 3 b c^2 c l - 2 a^2 a l b + a^2 a 2 b - a^2 a 3 b \\
& - 2 a^2 b b l - 2 a^2 b b 2 - 14 a^2 b c + 3 a 3 b b l c - a 3 b c c l - a a l b 3 c \\
& + a a l 3 b c + a a 2 b b 3 + a a 2 b c 3 - 2 a a 2 3 b c + 5 a a 3 b b 2 \\
& + 7 a a 3 b c 2 + 4 a^2 b c c 2 - 3 a a l b^2 b 2 - 4 a a l b^2 c 2 - 4 a a l b c^2 \\
& + a a l b l c^2 - 2 a a 2^2 b c + a a 2 b^2 b l + 4 a a 2 b^2 c l - 2 a a 2 b c^2 \\
& - a b^2 b l c + 2 a b^2 b l c l + a b^2 b l 1 c + 6 a b^2 c c l - 2 a b^2 c c l 1 \\
& - 2 a b b l^2 c - 4 a b b l c^2 + 2 a b b l 1 c^2 + a b c^2 c l - a b c^2 c l 1 \\
& + 2 a b c c l^2 - 2 a l b^2 b l c - a l b b l c^2 - a^2 a l a 3 b + a^2 a l b b 3 \\
& - 2 a^2 a l b c 2 + 2 a^2 a 2 a 3 b - a^2 b c l 2 + a^2 b c 2 2 - b b 2 c l + 2 b b 2 c 2
\end{aligned}$$

$$\begin{aligned}
& -2a^2bc^3 + a^2b^1c^3 + a^3a^2b + 10a^3bc + 2a^3bc^1 + 8a^2a^1b^2 \\
& -a^2b^2b^1 - 12a^2b^2c - 9a^2b^2c^1 + a^2b^2c^1 + a^1b^2c + a^1bb^2 \\
& + 2a^1bc + a^1bc^2 - a^2a^3b - a^2bb^2 - 2a^2bc - a^2bc^2 + 2a^3bb^2 \\
& + 2a^3bc - a^3bc^1 + 2a^3bc^2 - 2bb^1c - ac^3 + a^1a^3c
\end{aligned}$$

## EW structure written in terms of three simple invariants

We take the simplest invariants we know about and express our EW-structure in terms of them.

```

> J1 :=  $\frac{u_{2,3} + v_{2,2}}{u_2^2}$  : J2 :=  $\frac{u_2 u_{2,2,2}}{u_{2,2}^2}$  : J3 :=  $\frac{u_{2,2,3} + v_{2,2,2}}{u_{2,2} u_2}$  :
=
> simplify(map(LieDerivative, map(Prolong, [seq(Z||i, i=1..5)], 3), [J1, J2, J3]))
  [[0, 0, 0], [0, 0, 0], [0, 0, 0], [0, 0, 0], [0, 0, 0]] (7.2.1)
=
> TotalJac := Matrix([simplify(TotalDiff([J1, J2, J3], t)), simplify(TotalDiff([J1, J2,
  J3], x)), simplify(TotalDiff([J1, J2, J3], y))]) :
=
> TresseCoeffs := MatrixInverse(TotalJac) :
> D1 := proc(funct)
  (TresseCoeffs[1, 1]·TotalDiff(funct, t) + TresseCoeffs[1, 2]·TotalDiff(funct, x)
  + TresseCoeffs[1, 3]·TotalDiff(funct, y))
end proc:
D2 := proc(funct)
  (TresseCoeffs[2, 1]·TotalDiff(funct, t) + TresseCoeffs[2, 2]·TotalDiff(funct, x)
  + TresseCoeffs[2, 3]·TotalDiff(funct, y))
end proc:
D3 := proc(funct)
  (TresseCoeffs[3, 1]·TotalDiff(funct, t) + TresseCoeffs[3, 2]·TotalDiff(funct, x)
  + TresseCoeffs[3, 3]·TotalDiff(funct, y))
end proc:
=
>
> B := TotalJac :
>
> V3 := D3(x) D_x + D3(t) D_t + D3(y) D_y : V2 := D2(x) D_x + D2(t) D_t
  + D2(y) D_y : V1 := D1(x) D_x + D1(t) D_t + D1(y) D_y :
=
> alpha[1] := B[1, 1] dt + B[2, 1] dx + B[3, 1] dy : alpha[2] := B[1, 2] dt + B[2,
  2] dx + B[3, 2] dy : alpha[3] := B[1, 3] dt + B[2, 3] dx + B[3, 3] dy :
> Hook(V1, alpha[1]); Hook(V1, alpha[2]); Hook(V1, alpha[3]);
  1
  0
  0 (7.2.2)
=
> Hook(V2, alpha[1]); Hook(V2, alpha[2]); Hook(V2, alpha[3]);
  0
  1
  0 (7.2.3)
=
> Hook(V3, alpha[1]); Hook(V3, alpha[2]); Hook(V3, alpha[3]);
  0
  0
  1 (7.2.4)

```

The polynomials defining the singular set S.

> Generators(Simplify(⟨numer(op(DGinfo(evalDG(alpha[1] &w alpha[2]  
&w alpha[3])), "CoefficientSet"))), u[2], u[2, 2]))

$$\begin{aligned} & \{u_2, u_{2,2}, -4u_{1,2}u_{2,3}u_{2,2}^2u_{2,2,3,3} - 4u_{1,2}u_{2,3}u_{2,2}^2v_{2,2,2,3} \\ & + 6u_{1,2}u_{2,3}u_{2,2,2}u_{2,2,3}u_{2,2,2,3} + 4u_{1,2}u_{2,3}u_{2,2,2}u_{2,2,3}v_{2,2,2,2} \\ & + 2u_{1,2}u_{2,3}u_{2,2,2}u_{2,2,2,3}v_{2,2,2} - 2u_{1,2}u_{2,3}u_{2,2,3}^2u_{2,2,2,2} \\ & - 2u_{1,2}u_{2,3}u_{2,2,2,3}u_{2,2,2,2}v_{2,2,2} + 3u_{1,2}u_{2,2,2}^2u_{2,2,3}u_{2,3,3} + 3u_{1,2} \\ & u_{2,2,2}^2u_{2,2,3}v_{2,2,3} + 3u_{1,2}u_{2,2,2}^2u_{2,3,3}v_{2,2,2} - 4u_{1,2}u_{2,2,2}^2u_{2,2,3,3}v_{2,2} \\ & - 4u_{1,2}u_{2,2,2}^2v_{2,2}v_{2,2,2,3} + 3u_{1,2}u_{2,2,2}^2v_{2,2,2}v_{2,2,3} - 3u_{1,2}u_{2,2,2}u_{2,2,3}^3 \\ & - 6u_{1,2}u_{2,2,2}u_{2,2,3}^2v_{2,2,2} + 6u_{1,2}u_{2,2,2}u_{2,2,3}u_{2,2,2,3}v_{2,2} \\ & + 4u_{1,2}u_{2,2,2}u_{2,2,3}v_{2,2}v_{2,2,2,2} - 3u_{1,2}u_{2,2,2}u_{2,2,3}v_{2,2,2}^2 \\ & + 2u_{1,2}u_{2,2,2}u_{2,2,2,3}v_{2,2}v_{2,2,2} - 2u_{1,2}u_{2,2,3}^2u_{2,2,2,2}v_{2,2} \\ & - 2u_{1,2}u_{2,2,3}u_{2,2,2,2}v_{2,2}v_{2,2,2} - 4u_{2,3}^2u_{1,2,2}u_{2,2,2}u_{2,2,3} - 4 \\ & u_{2,3}^2u_{1,2,2}u_{2,2,2}v_{2,2,2,2} + 2u_{2,3}^2u_{1,2,2}u_{2,2,3}u_{2,2,2,2} + 2 \\ & u_{2,3}^2u_{1,2,2}u_{2,2,2,2}v_{2,2,2} + 4u_{2,3}^2u_{2,2,2}^2u_{1,2,2,3} + 4u_{2,3}^2u_{2,2,2}^2v_{1,2,2,2} - 2 \\ & u_{2,3}^2u_{2,2,2}^2u_{2,2,3}u_{1,2,2,2} - 2u_{2,3}^2u_{2,2,2}u_{1,2,2,2}v_{2,2,2} + 3u_{2,3}u_{1,2,2}u_{2,2,2} \\ & u_{2,2,3}^2 + 6u_{2,3}u_{1,2,2}u_{2,2,2}u_{2,2,3}v_{2,2,2} - 4u_{2,3}u_{1,2,2}u_{2,2,2}u_{2,2,3}v_{2,2} \\ & - 4u_{2,3}u_{1,2,2}u_{2,2,2}v_{2,2}v_{2,2,2,2} + 3u_{2,3}u_{1,2,2}u_{2,2,2}v_{2,2,2}^2 \\ & + 2u_{2,3}u_{1,2,2}u_{2,2,3}u_{2,2,2,2}v_{2,2} + 2u_{2,3}u_{1,2,2}u_{2,2,2,2}v_{2,2}v_{2,2,2} \\ & - 3u_{2,3}u_{1,2,3}u_{2,2,2}^2u_{2,2,3} - 3u_{2,3}u_{1,2,3}u_{2,2,2}^2v_{2,2,2} - 3u_{2,3} \\ & u_{2,2,2}^2u_{2,2,3}v_{1,2,2} + 4u_{2,3}u_{2,2,2}^2u_{1,2,2,3}v_{2,2} + 4u_{2,3}u_{2,2,2}^2v_{2,2}v_{1,2,2,2} \\ & - 3u_{2,3}u_{2,2,2}^2v_{1,2,2}v_{2,2,2} - 2u_{2,3}u_{2,2,2}u_{2,2,3}u_{1,2,2,2}v_{2,2} \\ & - 2u_{2,3}u_{2,2,2}u_{1,2,2,2}v_{2,2}v_{2,2,2}\} \end{aligned} \quad (7.2.5)$$

>  
> g := 4 dt &s dx + 2 u[ ] dt &s dy - (u[ ]^2 + 4 v[ ]) dt &s dt - dy &s dy :  
> G := Matrix( [ [Hook( [V1, V1], g), Hook( [V1, V2], g), Hook( [V1, V3], g) ],  
[Hook( [V2, V1], g), Hook( [V2, V2], g), Hook( [V2, V3], g) ], [Hook( [V3, V1],  
g), Hook( [V3, V2], g), Hook( [V3, V3], g) ] ) :  
> ans := Pullback(T4, LieDerivative(Prolong(ZI, 4), G[1, 2]) G[1, 1]  
- LieDerivative(Prolong(ZI, 4), G[1, 1]) G[1, 2] ) :

> var4 := DGinfo(MM, "FrameJetVariables")[1..73]  
var4 := [t, x, y, u[], v[], u<sub>1</sub>, u<sub>2</sub>, u<sub>3</sub>, v<sub>1</sub>, v<sub>2</sub>, v<sub>3</sub>, u<sub>1,1</sub>, u<sub>1,2</sub>, u<sub>1,3</sub>, u<sub>2,2</sub>, u<sub>2,3</sub>, u<sub>3,3</sub>, v<sub>1,1</sub>, v<sub>1,2</sub>,  
v<sub>1,3</sub>, v<sub>2,2</sub>, v<sub>2,3</sub>, v<sub>3,3</sub>, u<sub>1,1,1</sub>, u<sub>1,1,2</sub>, u<sub>1,1,3</sub>, u<sub>1,2,2</sub>, u<sub>1,2,3</sub>, u<sub>1,3,3</sub>, u<sub>2,2,2</sub>, u<sub>2,2,3</sub>,  
u<sub>2,3,3</sub>, u<sub>3,3,3</sub>, v<sub>1,1,1</sub>, v<sub>1,1,2</sub>, v<sub>1,1,3</sub>, v<sub>1,2,2</sub>, v<sub>1,2,3</sub>, v<sub>1,3,3</sub>, v<sub>2,2,2</sub>, v<sub>2,2,3</sub>, v<sub>2,3,3</sub>,  
v<sub>3,3,3</sub>, u<sub>1,1,1,1</sub>, u<sub>1,1,1,2</sub>, u<sub>1,1,1,3</sub>, u<sub>1,1,2,2</sub>, u<sub>1,1,2,3</sub>, u<sub>1,1,3,3</sub>, u<sub>1,2,2,2</sub>, u<sub>1,2,2,3</sub>,  
u<sub>1,2,3,3</sub>, u<sub>1,3,3,3</sub>, u<sub>2,2,2,2</sub>, u<sub>2,2,2,3</sub>, u<sub>2,2,3,3</sub>, u<sub>2,3,3,3</sub>, v<sub>1,1,1,1</sub>, v<sub>1,1,1,2</sub>,  
v<sub>1,1,1,3</sub>, v<sub>1,1,2,2</sub>, v<sub>1,1,2,3</sub>, v<sub>1,1,3,3</sub>, v<sub>1,2,2,2</sub>, v<sub>1,2,2,3</sub>, v<sub>1,2,3,3</sub>, v<sub>1,3,3,3</sub>,  
v<sub>2,2,2,2</sub>, v<sub>2,2,2,3</sub>, v<sub>2,2,3,3</sub>, v<sub>2,3,3,3</sub>, v<sub>3,3,3,3</sub>]

(7.2.6)



```

v1, 1, 1, 3, v1, 1, 2, 2, v1, 1, 2, 3, v1, 1, 3, 3, v1, 2, 2, 2, v1, 2, 2, 3, v1, 2, 3, 3, v1, 3, 3, 3, v2, 2, 2, 2,
v2, 2, 2, 3, v2, 2, 3, 3, v2, 3, 3, 3, v3, 3, 3, 3]
> subs(seq(var4[i] = Generate(rational), i = 1 .. nops(var4)), ans)
0 (7.2.7)
>
> omega := evalDG((u[ ] u[2] + 2 u[3] + 4 v[2]) dt - u[2] dy);
ω := (u[ ] u2 + 2 u3 + 4 v2) dt - (u2 dy) (7.2.8)
>
> om1 := Hook(V1, omega) - D1(log(G[1, 1])) : om2 := Hook(V2, omega)
- D2(log(G[1, 1])) : om3 := Hook(V3, omega) - D3(log(G[1, 1])) :
> subs(seq(var4[i] = Generate(rational), i = 1 .. nops(var4)), Pullback(T4,
LieDerivative(Prolong(Z1, 4), om1)))
> L1 := G[1, 2] / G[1, 1] : L2 := G[1, 3] / G[1, 1] : L3 := G[2, 2] / G[1, 1] : L4 := G[2, 3] / G[1, 1] : L5
:= G[3, 3] / G[1, 1] :
[>

```

## 4 Some particular Einstein-Weyl spaces

[>

### 4.1 u\_x=0

#### The dKP equation

[We add the equation u[2]=0 to Manakov-Santini system.

```

> eval(E1, [u[2]=0, u[1, 2]=0, u[2, 2]=0, u[2, 3]=0])
-u3,3 (8.1.1.1)

```

[We show that all solutions of this are equivalent to u=0, by using the following symmetry.

```

> phi := Transformation(MM, MM, [t=t, x=e(t)^2 x + e(t) diff(e(t), t) y^2, y
= e(t) y + b(t), u[ ] = e(t) u[ ] - y / e(t)^2 diff(e(t)^3, t) + diff(b(t), t), v[ ]
= e(t)^2 v[ ] + 2 e(t) diff(e(t), t) y u[ ] + (e(t) diff(e(t), t)
- 3 diff(e(t), t)^2) y^2 + 2 e(t) diff(e(t), t) x])
φ := [t=t, x=e(t)^2 x + e(t) ȧ(t) y^2, y=e(t) y + b(t), u[ ] = e(t) u[ ] - 3 y (8.1.1.2)
ȧ(t) + ḃ(t), v[ ] = e(t)^2 v[ ] + 2 e(t) ȧ(t) y u[ ] + (e(t) ȧ(t) - 3 ȧ(t)^2) y^2
+ 2 e(t) ȧ(t) x , ]

```

```

> simplify(Pullback(T2, Pullback(Prolong(phi, 2), [E1, E2])))
[0, 0] (8.1.1.3)

```

```

> expand((Pullback(phi, u[ ] - 0) / e(t))
u[ ] - 3 y (d/dt e(t)) / e(t) + d/dt b(t) / e(t) (8.1.1.4)

```

```

> eval(E2, [u[ ]=0, u[1]=0, u[2]=0, u[3]=0])
(8.1.1.5)

```

$$v_{[1]} v_{2,2} + v_2^2 + v_{1,2} - v_{3,3} \quad (8.1.1.5)$$

### Orbit of lowest dimension

We find the singular orbit in  $J^2$  of lowest dimension. It is given by the ideal  $\langle u_2, u_{1,2}, u_{2,2}, u_{2,3}, v_{2,2}, v_{2,3}, E1, E2 \rangle$ . These computations are quite time consuming.

```
> with(LinearAlgebra) : with(PolynomialIdeals) :
> var := DGinfo(MM, "FrameJetVariables") [4..23]
var := [u[ ], v[ ], u1, u2, u3, v1, v2, v3, u1,1, u1,2, u1,3, u2,2, u2,3, u3,3, v1,1, v1,2,
        v1,3, v2,2, v2,3, v3,3]
```

(8.1.2.1)

```
> nops([Y1seq(3), Y2seq(2), Y3seq(3), Y4seq(2), Y5seq(3)])
18
```

(8.1.2.2)

```
> DGSimplify([Y1seq(3), Y2seq(2), Y3seq(3), Y4seq(2), Y5seq(3)]); nops(%);
```

$$\begin{aligned} & \left[ D_{-t}, t D_{-t} + \frac{y D_{-y}}{2} - \frac{u[ ] D_{-u[ ]}}{2} - (v[ ] D_{-v[ ]}), t^2 D_{-t} + t y D_{-y} \right. \\ & \quad - ((t u[ ] - y) D_{-u[ ]}) - (2 t v[ ] D_{-v[ ]}), t^3 D_{-t} + \frac{3 t^2 y D_{-y}}{2} \\ & \quad - \left( \left( \frac{3}{2} u[ ] t^2 - 3 t y \right) D_{-u[ ]} \right) - (3 t^2 v[ ] D_{-v[ ]}), 2 x D_{-x} + y D_{-y} \\ & \quad + u_{[1]} D_{-u[ ]} + 2 v_{[1]} D_{-v[ ]}, (2 t x + y^2) D_{-x} + t y D_{-y} + (t u_{[1]} \\ & \quad - 3 y) D_{-u[ ]} + (2 t v_{[1]} + 2 y u_{[1]} + 2 x) D_{-v[ ]}, (2 t^2 x + 2 t y^2) D_{-x} \\ & \quad + t^2 y D_{-y} + (t^2 u_{[1]} - 6 t y) D_{-u[ ]} + (2 t^2 v_{[1]} + 4 t y u_{[1]} + 4 t x \\ & \quad + 2 y^2) D_{-v[ ]}, D_{-y}, t D_{-y} + D_{-u[ ]}, t^2 D_{-y} + 2 t D_{-u[ ]}, t^3 D_{-y} \\ & \quad + 3 t^2 D_{-u[ ]}, y D_{-x} - 2 D_{-u[ ]} + u_{[1]} D_{-v[ ]}, t y D_{-x} - 2 t D_{-u[ ]} + (t u_{[1]} \\ & \quad + y) D_{-v[ ]}, t^2 y D_{-x} - 2 t^2 D_{-u[ ]} + (t^2 u_{[1]} + 2 t y) D_{-v[ ]}, D_{-x}, t D_{-x} \\ & \quad + D_{-v[ ]}, t^2 D_{-x} + 2 t D_{-v[ ]}, t^3 D_{-x} + 3 t^2 D_{-v[ ]}] \end{aligned}$$

18

(8.1.2.3)

```
> sym := [t D_{-y} + D_{-u[ ]}, t D_{-x} + D_{-v[ ]}, t D_{-t} + \frac{y D_{-y}}{2} - \frac{u[ ] D_{-u[ ]}}{2}
        - (v[ ] D_{-v[ ]}), t^2 D_{-t} + t y D_{-y} - ((u[ ] t - y) D_{-u[ ]}) - (2 t v[ ] D_{-v[ ]}),
        t^3 D_{-t} + \frac{3 t^2 y D_{-y}}{2} - \left( \left( \frac{3}{2} u[ ] t^2 - 3 t y \right) D_{-u[ ]} \right) - (3 t^2 v[ ] D_{-v[ ]}),
        2 x D_{-x} + y D_{-y} + u_{[1]} D_{-u[ ]} + 2 v_{[1]} D_{-v[ ]}, (2 t x + y^2) D_{-x} + t y D_{-y}
        + (t u_{[1]} - 3 y) D_{-u[ ]} + (2 t v_{[1]} + 2 y u_{[1]} + 2 x) D_{-v[ ]}, (2 t^2 x
        + 2 t y^2) D_{-x} + t^2 y D_{-y} + (t^2 u_{[1]} - 6 t y) D_{-u[ ]} + (2 t^2 v_{[1]} + 4 t y u_{[1]}
        + 4 t x + 2 y^2) D_{-v[ ]}, t^2 D_{-y} + 2 t D_{-u[ ]}, t^3 D_{-y} + 3 t^2 D_{-u[ ]}, y D_{-x}
        - 2 D_{-u[ ]} + u_{[1]} D_{-v[ ]}, t y D_{-x} - 2 t D_{-u[ ]} + (t u_{[1]} + y) D_{-v[ ]}, t^2 y D_{-x}
        - 2 t^2 D_{-u[ ]} + (t^2 u_{[1]} + 2 t y) D_{-v[ ]}, t^2 D_{-x} + 2 t D_{-v[ ]}, t^3 D_{-x}
        + 3 t^2 D_{-v[ ]}]: nops(sym);
```

15

(8.1.2.4)

```

> A := eval(Matrix(Pullback(T2, map(LieDerivative, map(Prolong, sym, 2), var))),
  {x=0, y=0, t=0})

```

$$A := \begin{bmatrix} 15 \times 20 \text{ Matrix} \\ \text{Data Type: anything} \\ \text{Storage: rectangular} \\ \text{Order: Fortran\_order} \end{bmatrix} \quad (8.1.2.5)$$

```

> Rank(A); Rank(subs(seq(var[i]=0, i=1..nops(var)), A));
15
12

```

(8.1.2.6)

```

> mat13 := [seq(seq(seq(seq(seq(seq(seq(DeleteColumn(DeleteRow(A,
[i1, i2]), [j1, j2, j3, j4, j5, j6, j7]), i1=1..i2-1), i2=2..15), j1=1..j2-1),
j2=2..j3-1), j3=3..j4-1), j4=4..j5-1), j5=5..j6-1), j6=6..j7-1)
, j7=7..20)]: nops(mat13)
8139600

```

(8.1.2.7)

```

> singset13 := {op(map(Determinant, mat13))}:
> ideal := Simplify(<op(singset13)>):
> ideal

```

$$\langle u_2, u_1, 2, u_2, 2, u_2, 3, v_2, 2, v_2, 3 \rangle \quad (8.1.2.8)$$

```

> eval([E1, E2], [u[2]=0, u[1, 2]=0, u[2, 2]=0, u[2, 3]=0, v[2, 2]=0, v[2, 3]
=0])

```

$$[-u_3, 3, 2 u_3 v_2 + v_2^2 + v_{1, 2} - v_{3, 3}] \quad (8.1.2.9)$$

```

> pdsolve(FromJet({u[2], u[1, 2], u[2, 2], u[2, 3], v[2, 2], v[2, 3], E1, E2}, {u(t,
x, y), v(t, x, y)}))

```

$$\left\{ u(t, x, y) = \_F1(t) y + \_F2(t), v(t, x, y) = \_F5(t) x + \frac{1}{2} \left( 2 \_F1(t) \_F5(t) + \_F5(t)^2 + \frac{d}{dt} \_F5(t) \right) y^2 + \_F6(t) y + \_F7(t) \right\} \quad (8.1.2.10)$$

```

> pdsolve(FromJet({u[2], u[1, 2], u[2, 2], u[2, 3], v[2, 2], v[2, 3], u[1], u[3],
u[ ], E1, E2}, {u(t, x, y), v(t, x, y)}))

```

$$\left\{ u(t, x, y) = 0, v(t, x, y) = \_F3(t) x + \frac{1}{2} \left( \_F3(t)^2 + \frac{d}{dt} \_F3(t) \right) y^2 + \_F4(t) y + \_F5(t) \right\} \quad (8.1.2.11)$$

```

> phi := simplify(Transformation(MM, MM, [t=d(t), x=e(t)^2 x
+ e(t) diff(e(t), t) y^2 + c(t) y + a(t), y=sqrt(diff(d(t), t)) e(t) y + b(t),
u[ ] = \frac{e(t) u[ ]}{sqrt(diff(d(t), t))} - \frac{y}{e(t)^2} diff\left(\frac{e(t)^3}{sqrt(diff(d(t), t))}, t\right)
+ \frac{diff(b(t), t)}{diff(d(t), t)} - \frac{2 c(t)}{e(t) sqrt(diff(d(t), t))}, v[ ] = \frac{e(t)^2}{diff(d(t), t)} v[ ]

```

$$\begin{aligned}
& + \frac{(c(t) + 2 e(t) \operatorname{diff}(e(t), t) y)}{\operatorname{diff}(d(t), t)} u[ ] \\
& + \frac{(e(t) \operatorname{diff}(e(t), t, t) - 3 \operatorname{diff}(e(t), t)^2)}{\operatorname{diff}(d(t), t)} y^2 + \frac{e(t)^4}{\operatorname{diff}(d(t), t)} \operatorname{diff}\left(\frac{c(t)}{e(t)^4}, \right. \\
& \left. t\right) y + \frac{2 e(t) \operatorname{diff}(e(t), t)}{\operatorname{diff}(d(t), t)} x + \frac{(e(t)^2 \operatorname{diff}(a(t), t) - c(t)^2)}{\operatorname{diff}(d(t), t) e(t)^2} \left. \right] \left. \right) \left. \right) \\
\phi := & \left[ t = d(t), x = e(t)^2 x + e(t) \dot{e}(t) y^2 + c(t) y + a(t), y = \sqrt{d(t)} e(t) y \right. \quad (8.1.2.12)
\end{aligned}$$

$$\begin{aligned}
& + b(t), u[ ] = \frac{1}{2 \dot{d}(t)^{3/2} e(t)} \left( 2 \dot{d}(t) e(t)^2 u[ ] + e(t)^2 \ddot{d}(t) y \right. \\
& \left. - 6 e(t) \dot{d}(t) \dot{e}(t) y + 2 \dot{b}(t) e(t) \sqrt{d(t)} - 4 c(t) \dot{d}(t) \right), v[ ] \\
& = \frac{1}{e(t)^2 \dot{d}(t)} \left( e(t)^3 \ddot{e}(t) y^2 - 3 e(t)^2 \dot{e}(t)^2 y^2 + 2 \left( (y u[ ] + x) e(t)^2 \right. \right. \\
& \left. \left. - 2 c(t) y \right) e(t) \dot{e}(t) + e(t)^4 v[ ] + e(t)^2 \dot{c}(t) y + e(t)^2 c(t) u[ ] + e(t)^2 \right. \\
& \left. \dot{a}(t) - c(t)^2 \right) \quad , \quad ]
\end{aligned}$$

$$\begin{aligned}
& \text{> simplify(Pullback(T2, Pullback(Prolong(phi, 2), [E1, E2])))} \\
& \quad [0, 0] \quad (8.1.2.13)
\end{aligned}$$

$$\begin{aligned}
& \text{> sol := collect(solve(Pullback(phi, [u[ ] - 0, v[ ] - 0]), {u[ ], v[ ]}), [u, v[ ], x, \\
& \quad y])
\end{aligned}$$

$$\begin{aligned}
\text{sol} := & \left\{ u[ ] = -\frac{1}{2} \frac{\left( e(t)^2 \left( \frac{d^2}{dt^2} d(t) \right) - 6 e(t) \left( \frac{d}{dt} d(t) \right) \left( \frac{d}{dt} e(t) \right) \right) y}{e(t)^2 \left( \frac{d}{dt} d(t) \right)} \right. \quad (8.1.2.14)
\end{aligned}$$

$$\begin{aligned}
& - \frac{1}{2} \frac{2 \left( \frac{d}{dt} b(t) \right) e(t) \sqrt{\frac{d}{dt} d(t)} - 4 c(t) \left( \frac{d}{dt} d(t) \right)}{e(t)^2 \left( \frac{d}{dt} d(t) \right)}, v[ ] =
\end{aligned}$$

$$\begin{aligned}
& - \frac{2 \left( \frac{d}{dt} e(t) \right) x}{e(t)}
\end{aligned}$$

$$\begin{aligned}
& - \frac{1}{2} \frac{1}{e(t)^4 \left( \frac{d}{dt} d(t) \right)} \left( \left( 2 e(t)^3 \left( \frac{d^2}{dt^2} e(t) \right) \left( \frac{d}{dt} d(t) \right) \right. \right.
\end{aligned}$$

$$\begin{aligned}
& \left. - 2 e(t)^3 \left( \frac{d^2}{dt^2} d(t) \right) \left( \frac{d}{dt} e(t) \right) + 6 e(t)^2 \left( \frac{d}{dt} e(t) \right)^2 \left( \frac{d}{dt} d(t) \right) \right)
\end{aligned}$$

$$\begin{aligned}
& y^2 \Big) - \frac{1}{2} \frac{1}{e(t)^4 \left( \frac{d}{dt} d(t) \right)} \Bigg( \Big( \\
& -4 e(t)^2 \left( \frac{d}{dt} e(t) \right) \left( \frac{d}{dt} b(t) \right) \sqrt{\frac{d}{dt} d(t)} - e(t)^2 \left( \frac{d^2}{dt^2} d(t) \right) c(t) \\
& + 2 e(t)^2 \left( \frac{d}{dt} c(t) \right) \left( \frac{d}{dt} d(t) \right) + 6 e(t) \left( \frac{d}{dt} e(t) \right) c(t) \left( \frac{d}{dt} d(t) \right) \Big) \\
& y \Big) - \frac{1}{2} \frac{1}{e(t)^4 \left( \frac{d}{dt} d(t) \right)} \Bigg( 2 e(t)^2 \left( \frac{d}{dt} a(t) \right) \left( \frac{d}{dt} d(t) \right) \\
& - 2 e(t) \left( \frac{d}{dt} b(t) \right) c(t) \sqrt{\frac{d}{dt} d(t)} + 2 c(t)^2 \left( \frac{d}{dt} d(t) \right) \Bigg) \Bigg\}
\end{aligned}$$

$$\begin{aligned}
& \text{> sol2} := \text{simplify} \left( \text{eval} \left( \text{eval} \left( \text{eval} \left( \text{sol}, \left\{ c(t) = \text{solve} \left( \begin{aligned} & \frac{1}{2} \frac{2 \left( \frac{d}{dt} b(t) \right) e(t) \sqrt{\frac{d}{dt} d(t)} - 4 c(t) \left( \frac{d}{dt} d(t) \right)}{e(t)^2 \left( \frac{d}{dt} d(t) \right)}, c(t) \right) \right\} \right) \right) \right) \right), \left\{ e(t) \right. \\
& \left. = cI e^{\int \left( -\frac{1}{2} f4(t) \right) dt} \right\}, \left\{ d(t) = c2 + \left( \int e^{\int (-2f2(t) - 3f4(t)) dt} dt \right) c3 \right\}, \text{symbolic} \right)
\end{aligned}$$

$$\text{sol2} := \left\{ u_{\square} = f2(t) y - fI(t), v_{\square} = \frac{1}{2} \frac{1}{c3^{3/2} cI^2} \left( \left( c3^{3/2} \left( \left( \frac{d}{dt} fI(t) \right) y \right. \right. \right. \quad (8.1.2.15)$$

$$+ \left( \frac{d}{dt} f4(t) \right) y^2 + f4(t)^2 y^2 + (2 f2(t) y^2 - fI(t) y + 2 x) f4(t)$$

$$+ fI(t) \left( f2(t) y - \frac{1}{2} fI(t) \right) \Big)$$

$$cI^2 e^{\frac{5}{2} \int f4(t) dt + 2 \left( \int (-2f2(t) - 3f4(t)) dt \right) + 2 \left( \int f2(t) dt \right)} + \frac{3}{2} \left( f4(t) y$$

$$+ \frac{2}{3} f2(t) y - \frac{2}{3} fI(t) \Big)$$

$$cI \left( \frac{d}{dt} b(t) \right) c3 e^{\frac{9}{2} \int f4(t) dt + 3 \left( \int f2(t) dt \right) + 2 \left( \int (-2f2(t) - 3f4(t)) dt \right)}$$

$$\begin{aligned}
& -2 e^{2 \left( \int (-2f2(t) - 3f4(t)) \, dt \right) + 2 \left( \int f2(t) \, dt \right) + \frac{7}{2} \int f4(t) \, dt} \left( \frac{d}{dt} a(t) \right) c3^{3/2} \\
& + e^{\int (-2f2(t) - 3f4(t)) \, dt + 2 \left( \int f2(t) \, dt \right) + \frac{7}{2} \int f4(t) \, dt} \left( \frac{d}{dt} b(t) \right)^2 \sqrt{c3} \\
& - \frac{9}{2} cI \left( \frac{2}{9} \left( \frac{d^2}{dt^2} b(t) \right) y + \left( \frac{d}{dt} b(t) \right) \left( f4(t) y + \frac{2}{3} f2(t) y \right. \right. \\
& \left. \left. - \frac{2}{9} fI(t) \right) \right) c3 e^{\frac{3}{2} \int f4(t) \, dt + \int f2(t) \, dt + \int (-2f2(t) - 3f4(t)) \, dt} \\
& - \frac{1}{2} \left( \frac{d}{dt} b(t) \right)^2 e^{\frac{1}{2} \int f4(t) \, dt} \sqrt{c3} \Bigg\} \\
& e^{-\frac{5}{2} \int f4(t) \, dt - 2 \left( \int f2(t) \, dt \right) - 2 \left( \int (-2f2(t) - 3f4(t)) \, dt \right)} \Bigg\}
\end{aligned}$$

> simplify(coeff(eval(v[ ], sol2[2]), y^2))

$$f2(t) f4(t) + \frac{1}{2} f4(t)^2 + \frac{1}{2} \frac{d}{dt} f4(t)$$

(8.1.2.16)

> simplify(coeff(eval(v[ ], sol2[2]), x))

$$f4(t)$$

(8.1.2.17)

> simplify(eval(eval(v[ ], sol2[2]), {x=0, y=0}))

$$\begin{aligned}
& -\frac{1}{4} \frac{1}{c3^{3/2} cI^2} \left( e^{-\frac{5}{2} \int f4(t) \, dt - 2 \left( \int f2(t) \, dt \right) - 2 \left( \int (-2f2(t) - 3f4(t)) \, dt \right)} \left( 2 \right. \right. \\
& e^{\frac{9}{2} \int f4(t) \, dt + 3 \left( \int f2(t) \, dt \right) + 2 \left( \int (-2f2(t) - 3f4(t)) \, dt \right)} fI(t) \left( \frac{d}{dt} b(t) \right) cI c3 \\
& + e^{\frac{5}{2} \int f4(t) \, dt + 2 \left( \int (-2f2(t) - 3f4(t)) \, dt \right) + 2 \left( \int f2(t) \, dt \right)} fI(t)^2 cI^2 c3^{3/2} \\
& + 4 e^{2 \left( \int (-2f2(t) - 3f4(t)) \, dt \right) + 2 \left( \int f2(t) \, dt \right) + \frac{7}{2} \int f4(t) \, dt} \left( \frac{d}{dt} a(t) \right) c3^{3/2} \\
& + \left( \frac{d}{dt} b(t) \right) \left( -2 cI e^{\frac{3}{2} \int f4(t) \, dt + \int f2(t) \, dt + \int (-2f2(t) - 3f4(t)) \, dt} c3 fI(t) \right. \\
& + \sqrt{c3} \left( \frac{d}{dt} b(t) \right) e^{\frac{1}{2} \int f4(t) \, dt} \\
& \left. \left. - 2 \sqrt{c3} \left( \frac{d}{dt} b(t) \right) e^{\int (-2f2(t) - 3f4(t)) \, dt + 2 \left( \int f2(t) \, dt \right) + \frac{7}{2} \int f4(t) \, dt} \right) \right) \Bigg)
\end{aligned}$$

(8.1.2.18)

> simplify(coeff(eval(v[ ], sol2[2]), y))

$$\begin{aligned}
& -\frac{3}{2} \frac{1}{\sqrt{c3} cI} \left( e^{-\frac{5}{2} \int f4(t) \, dt - 2 \left( \int f2(t) \, dt \right) - 2 \left( \int (-2f2(t) - 3f4(t)) \, dt \right)} \left( \right. \right. \\
& \left. \left. - \frac{1}{3} \sqrt{c3} cI \left( \frac{d}{dt} fI(t) - fI(t) f4(t) \right) \right) \right)
\end{aligned}$$

(8.1.2.19)

$$\begin{aligned}
& + f1(t) f2(t) \Big) e^{\frac{5}{2} \int f4(t) dt + 2 \left( \int (-2f2(t) - 3f4(t)) dt \right) + 2 \left( \int f2(t) dt \right)} \\
& - \frac{1}{3} \left( \frac{d}{dt} b(t) \right) \left( f2(t) \right. \\
& + \frac{3}{2} f4(t) \Big) e^{\frac{9}{2} \int f4(t) dt + 3 \left( \int f2(t) dt \right) + 2 \left( \int (-2f2(t) - 3f4(t)) dt \right)} \\
& + e^{\frac{3}{2} \int f4(t) dt + \int f2(t) dt + \int (-2f2(t) - 3f4(t)) dt} \left( \frac{1}{3} \frac{d^2}{dt^2} b(t) \right. \\
& + \left. \left( \frac{d}{dt} b(t) \right) \left( f2(t) + \frac{3}{2} f4(t) \right) \right) \Big) \Big)
\end{aligned}$$

## 4.2 The Martinez-Alonso Shabat equation

$$\begin{aligned}
& > \text{MAS} := \text{ToJet}(\text{eval}(\text{FromJet}([E1, E2], \{u(t, x, y), v(t, x, y)\}), \{u(t, x, y) = \text{diff}(w(t, x, y), x), v(t, x, y) = -\text{diff}(w(t, x, y), y)\}), w(t, x, y)) \\
& \text{MAS} := \left[ w_x w_{x, x, y} - w_y w_{x, x, x} + w_{t, x, x} - w_{x, y, y} - w_x w_{x, y, y} + w_y w_{x, x, y} + w_{x, x} w_{y, y} - \right. \quad (8.2.1) \\
& \quad \left. w_{x, y}^2 - w_{t, x, y} + w_{y, y, y} \right]
\end{aligned}$$

$$\begin{aligned}
& > \text{ToJet}(\text{diff}(\text{FromJet}(w[1, 2] + w[2] w[2, 3] - w[3] w[2, 2] - w[3, 3], w(t, x, y)), x), \\
& \quad w(t, x, y)) - \text{MAS}[1] \\
& \quad \quad \quad 0 \quad (8.2.2)
\end{aligned}$$

$$\begin{aligned}
& > \text{ToJet}(\text{diff}(\text{FromJet}(w[1, 2] + w[2] w[2, 3] - w[3] w[2, 2] - w[3, 3], w(t, x, y)), y), \\
& \quad w(t, x, y)) + \text{MAS}[2] \\
& \quad \quad \quad 0 \quad (8.2.3)
\end{aligned}$$

$$\begin{aligned}
& > \text{DGsetup}([t, x, y], [w], \text{NN}, 2) \\
& \quad \quad \quad \text{frame name: NN} \quad (8.2.4)
\end{aligned}$$

$$\begin{aligned}
& > \text{eq} := w[1, 2] + w[2] w[2, 3] - w[3] w[2, 2] - w[3, 3] \\
& \quad \quad \quad \text{eq} := w_2 w_{2, 3} - w_3 w_{2, 2} + w_{1, 2} - w_{3, 3} \quad (8.2.5)
\end{aligned}$$

We may add an arbitrary function of t to this equation by using a point transformation.

$$\begin{aligned}
& > \text{phi} := \text{Transformation}(\text{NN}, \text{NN}, [t=t, x=x, y=y, w[ ] = w[ ] + \text{integrate}(f(t), t) x]) \\
& \quad \quad \quad \phi := \left[ t=t, x=x, y=y, w[ ] = w[ ] + \left( \int f(t) dt \right) x \right] \quad (8.2.6)
\end{aligned}$$

$$\begin{aligned}
& > \text{eq2} := \text{simplify}(\text{Pullback}(\text{Prolong}(\text{phi}, 2), \text{eq})) \\
& \quad \quad \quad \text{eq2} := \left( \int f(t) dt + w_2 \right) w_{2, 3} - w_3 w_{2, 2} + f(t) + w_{1, 2} - w_{3, 3} \quad (8.2.7)
\end{aligned}$$

$$\begin{aligned}
& > \text{pdsolve}(\{ \text{LieDerivative}(D_t + \text{integrate}(f(t), t) D_y, T(t, y)) - 1, \text{LieDerivative}(D_t \\
& \quad + \text{integrate}(f(t), t) D_y, Y(t, y)), \text{LieDerivative}(D_y, Y(t, y)) - 1, \\
& \quad \text{LieDerivative}(D_y, T(t, y)) \}, \{T, Y\}) \\
& \quad \quad \quad \left\{ T(t, y) = t + \_C2, Y(t, y) = y + \int \left( - \left( \int f(t) dt \right) \right) dt + \_C1 \right\} \quad (8.2.8)
\end{aligned}$$

$$\begin{aligned}
& > \text{phi} := \text{Transformation}(\text{NN}, \text{NN}, [t=t, x=x, y=y + \text{integrate}(\text{integrate}(f(t), t), t), \\
& \quad w[ ] = w[ ]]) \\
& \quad \quad \quad \phi := \left[ t=t, x=x, y=y + \iint f(t) dt dt, w[ ] = w[ ] \right] \quad (8.2.9)
\end{aligned}$$

$$\begin{aligned}
& > \text{simplify}(\text{numer}(\text{Pullback}(\text{Prolong}(\text{phi}, 2), \text{eq2})) - \text{eq}) \\
& \quad \quad \quad (8.2.10)
\end{aligned}$$

### 4.3 I1=I2=I3=0

I1,I2,I3 as defined here are the numerators of those in the other sections.

$$\begin{aligned} &> I1 := u_{2,3} + v_{2,2} : I2 := u_2^2 u_{2,3} + u_2 v_2 u_{2,2} + u_{2,2} u_{3,3} - u_{2,3}^2 : I3 := u_2^2 v_{2,2} \\ &\quad - u_2 v_2 u_{2,2} + u_{2,2} v_{2,3} - u_{2,3} v_{2,2} : \end{aligned}$$

$$\begin{aligned} &> \text{simplify}(I2 + I3 + (u_{2,3} - u_2^2) I1 - u_{2,2} (u_{3,3} + v_{2,3})) \\ &\quad 0 \end{aligned}$$

(8.3.1)

We use rifsimp.

$$\begin{aligned} &> \text{sys} := \text{FromJet}(\{E1, E2, I1, I2, I3\}, \{u(t, x, y), v(t, x, y)\}) \end{aligned}$$

$$\begin{aligned} \text{sys} := & \left\{ \frac{\partial^2}{\partial y \partial x} u(t, x, y) + \frac{\partial^2}{\partial x^2} v(t, x, y), \left( \frac{\partial}{\partial x} u(t, x, y) \right)^2 \left( \frac{\partial^2}{\partial x^2} v(t, x, y) \right) \right. \\ & - \left( \frac{\partial}{\partial x} u(t, x, y) \right) \left( \frac{\partial^2}{\partial x^2} u(t, x, y) \right) \left( \frac{\partial}{\partial x} v(t, x, y) \right) + \left( \frac{\partial^2}{\partial x^2} u(t, x, \right. \\ & y) \left( \frac{\partial^2}{\partial y \partial x} v(t, x, y) \right) - \left( \frac{\partial^2}{\partial y \partial x} u(t, x, y) \right) \left( \frac{\partial^2}{\partial x^2} v(t, x, y) \right), \left( \frac{\partial}{\partial x} u(t, x, \right. \\ & y) \left. \right)^2 \left( \frac{\partial^2}{\partial y \partial x} u(t, x, y) \right) + \left( \frac{\partial}{\partial x} u(t, x, y) \right) \left( \frac{\partial^2}{\partial x^2} u(t, x, y) \right) \left( \frac{\partial}{\partial x} v(t, x, y) \right) \\ & + \left( \frac{\partial^2}{\partial x^2} u(t, x, y) \right) \left( \frac{\partial^2}{\partial y^2} u(t, x, y) \right) - \left( \frac{\partial^2}{\partial y \partial x} u(t, x, y) \right)^2, u(t, x, \\ & y) \left( \frac{\partial^2}{\partial y \partial x} u(t, x, y) \right) + \left( \frac{\partial}{\partial x} u(t, x, y) \right) \left( \frac{\partial}{\partial y} u(t, x, y) \right) + \left( \frac{\partial}{\partial x} u(t, x, \right. \\ & y) \left( \frac{\partial}{\partial x} v(t, x, y) \right) + \left( \frac{\partial^2}{\partial x^2} u(t, x, y) \right) v(t, x, y) + \frac{\partial^2}{\partial x \partial t} u(t, x, y) \\ & - \left( \frac{\partial^2}{\partial y^2} u(t, x, y) \right), u(t, x, y) \left( \frac{\partial^2}{\partial y \partial x} v(t, x, y) \right) - \left( \frac{\partial}{\partial x} u(t, x, y) \right) \left( \frac{\partial}{\partial y} v(t, \right. \\ & x, y) \left. \right) + 2 \left( \frac{\partial}{\partial y} u(t, x, y) \right) \left( \frac{\partial}{\partial x} v(t, x, y) \right) + v(t, x, y) \left( \frac{\partial^2}{\partial x^2} v(t, x, y) \right) \\ & \left. + \left( \frac{\partial}{\partial x} v(t, x, y) \right)^2 + \frac{\partial^2}{\partial x \partial t} v(t, x, y) - \left( \frac{\partial^2}{\partial y^2} v(t, x, y) \right) \right\} \end{aligned}$$

$$\begin{aligned} &> \text{with(DEtools)} : \end{aligned}$$

$$\begin{aligned} &> \text{cases} := \text{rifsimp}(\text{sys}, \text{casesplit}) : \end{aligned}$$

$$\begin{aligned} &> \text{cases}_{\text{casecount}} \end{aligned}$$

10

(8.3.3)

$$\begin{aligned} &> \text{caseplot}(\text{cases}) \end{aligned}$$



### Rif Case Tree

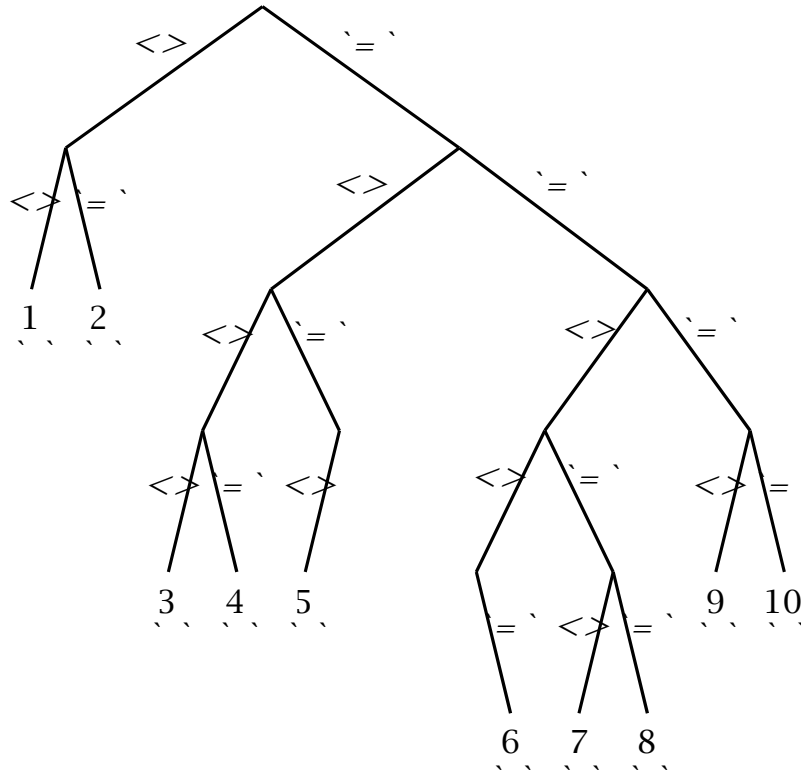

We analyze the first (main) branch.

> copy(cases<sub>1</sub>)

$$\begin{aligned}
 \text{table} \left( \left[ \begin{aligned} & \text{Case} = \left[ \left[ \frac{\partial^2}{\partial y^2} u(t, x, y) + \frac{\partial^2}{\partial y \partial x} v(t, x, y) \neq 0, \frac{\partial^2}{\partial x^2} u(t, x, y) \right], \left[ \frac{\partial}{\partial x} u(t, x, \right. \right. \\ & \left. \left. y) \neq 0, \frac{\partial^2}{\partial y \partial x} u(t, x, y) \right] \right], \text{Pivots} = \left[ \frac{\partial^2}{\partial y^2} u(t, x, y) + \frac{\partial^2}{\partial y \partial x} v(t, x, y) \neq 0, \right. \\ & \left. \frac{\partial}{\partial x} u(t, x, y) \neq 0 \right], \text{Solved} = \left[ \frac{\partial^4}{\partial y^4} v(t, x, y) = 2 \left( \frac{\partial}{\partial x} u(t, x, y) \right) \left( \frac{\partial}{\partial x} v(t, x, \right. \right. \\ & \left. \left. y) \right) \left( \frac{\partial^2}{\partial y^2} u(t, x, y) \right) + 2 \left( \frac{\partial}{\partial x} u(t, x, y) \right) \left( \frac{\partial}{\partial x} v(t, x, y) \right) \left( \frac{\partial^2}{\partial y \partial x} v(t, x, y) \right) \right. \\ & \left. - \left( \frac{\partial}{\partial x} u(t, x, y) \right) \left( \frac{\partial^3}{\partial y^3} v(t, x, y) \right) + 5 \left( \frac{\partial^2}{\partial y^2} u(t, x, y) \right) \left( \frac{\partial^2}{\partial y \partial x} v(t, x, y) \right) \right. \\ & \left. + 2 \left( \frac{\partial^2}{\partial y \partial x} v(t, x, y) \right)^2, \frac{\partial^3}{\partial y^2 \partial x} v(t, x, y) = 0, \frac{\partial^3}{\partial y^3} u(t, x, y) = \left( \frac{\partial}{\partial x} u(t, x, \right. \right. \\ & \left. \left. y) \right) \left( \frac{\partial^2}{\partial y^2} u(t, x, y) + \frac{\partial^2}{\partial y \partial x} v(t, x, y) \right), \frac{\partial^2}{\partial x \partial t} u(t, x, y) = - \left( \frac{\partial}{\partial x} u(t, x, \right. \right. \\ & \left. \left. y) \right) \left( \frac{\partial}{\partial x} v(t, x, y) \right) - \left( \frac{\partial}{\partial x} u(t, x, y) \right) \left( \frac{\partial}{\partial y} u(t, x, y) \right) + \frac{\partial^2}{\partial y^2} u(t, x, y), \right. \end{aligned} \right] \right) \quad (8.3.4)
 \end{aligned}$$

$$\begin{aligned} \frac{\partial^2}{\partial x \partial t} v(t, x, y) &= \left( \frac{\partial}{\partial x} u(t, x, y) \right) \left( \frac{\partial}{\partial y} v(t, x, y) \right) - \left( \frac{\partial}{\partial x} v(t, x, y) \right)^2 \\ &- 2 \left( \frac{\partial}{\partial y} u(t, x, y) \right) \left( \frac{\partial}{\partial x} v(t, x, y) \right) - u(t, x, y) \left( \frac{\partial^2}{\partial y \partial x} v(t, x, y) \right) \\ &+ \frac{\partial^2}{\partial y^2} v(t, x, y), \frac{\partial^2}{\partial x^2} u(t, x, y) = 0, \frac{\partial^2}{\partial x^2} v(t, x, y) = 0, \frac{\partial^2}{\partial y \partial x} u(t, x, y) = 0 \end{aligned} \Bigg] \Bigg]$$

> %Solved

$$\left[ \frac{\partial^4}{\partial y^4} v(t, x, y) = 2 \left( \frac{\partial}{\partial x} u(t, x, y) \right) \left( \frac{\partial}{\partial x} v(t, x, y) \right) \left( \frac{\partial^2}{\partial y^2} u(t, x, y) \right) \right. \quad (8.3.5)$$

$$\begin{aligned} &+ 2 \left( \frac{\partial}{\partial x} u(t, x, y) \right) \left( \frac{\partial}{\partial x} v(t, x, y) \right) \left( \frac{\partial^2}{\partial y \partial x} v(t, x, y) \right) - \left( \frac{\partial}{\partial x} u(t, x, \right. \\ &y) \left. \right) \left( \frac{\partial^3}{\partial y^3} v(t, x, y) \right) + 5 \left( \frac{\partial^2}{\partial y^2} u(t, x, y) \right) \left( \frac{\partial^2}{\partial y \partial x} v(t, x, y) \right) \\ &+ 2 \left( \frac{\partial^2}{\partial y \partial x} v(t, x, y) \right)^2, \frac{\partial^3}{\partial y^2 \partial x} v(t, x, y) = 0, \frac{\partial^3}{\partial y^3} u(t, x, y) = \left( \frac{\partial}{\partial x} u(t, x, \right. \\ &y) \left. \right) \left( \frac{\partial^2}{\partial y^2} u(t, x, y) + \frac{\partial^2}{\partial y \partial x} v(t, x, y) \right), \frac{\partial^2}{\partial x \partial t} u(t, x, y) = - \left( \frac{\partial}{\partial x} u(t, x, \right. \\ &y) \left. \right) \left( \frac{\partial}{\partial x} v(t, x, y) \right) - \left( \frac{\partial}{\partial x} u(t, x, y) \right) \left( \frac{\partial}{\partial y} u(t, x, y) \right) + \frac{\partial^2}{\partial y^2} u(t, x, y), \\ &\frac{\partial^2}{\partial x \partial t} v(t, x, y) = \left( \frac{\partial}{\partial x} u(t, x, y) \right) \left( \frac{\partial}{\partial y} v(t, x, y) \right) - \left( \frac{\partial}{\partial x} v(t, x, y) \right)^2 \\ &- 2 \left( \frac{\partial}{\partial y} u(t, x, y) \right) \left( \frac{\partial}{\partial x} v(t, x, y) \right) - u(t, x, y) \left( \frac{\partial^2}{\partial y \partial x} v(t, x, y) \right) \\ &+ \frac{\partial^2}{\partial y^2} v(t, x, y), \frac{\partial^2}{\partial x^2} u(t, x, y) = 0, \frac{\partial^2}{\partial x^2} v(t, x, y) = 0, \frac{\partial^2}{\partial y \partial x} u(t, x, y) = 0 \end{aligned}$$

$$\begin{aligned} &> pdsolve \left( \left[ \frac{\partial^3}{\partial y^2 \partial x} v(t, x, y) = 0, \frac{\partial^3}{\partial y^3} u(t, x, y) = \left( \frac{\partial}{\partial x} u(t, x, y) \right) \left( \frac{\partial^2}{\partial y^2} u(t, x, y) \right) \right. \right. \\ &\quad \left. \left. + \frac{\partial^2}{\partial y \partial x} v(t, x, y) \right), \frac{\partial^2}{\partial x^2} u(t, x, y) = 0, \frac{\partial^2}{\partial x^2} v(t, x, y) = 0, \frac{\partial^2}{\partial y \partial x} u(t, x, y) = 0 \right] \right) \end{aligned}$$

$$\left\{ u(t, x, y) = \_F7(t) x + \frac{\_F8(t) e^{-F7(t) y}}{\_F7(t)^2} - \frac{1}{2} \_F3(t) y^2 + \_F9(t) y + \_F10(t), v(t, \quad (8.3.6) \right.$$

$$\left. x, y) = \_F3(t) x y + \_F4(t) x + \_F2(t, y) \right\}$$

$$\begin{aligned} &> \text{phi} := \text{simplify} \left( \left( \text{Transformation} \left( MM, MM, \left[ t = d(t), x = e(t)^2 x + e(t) \text{diff}(e(t), \right. \right. \right. \right. \\ &\quad \left. \left. \left. t \right) y^2 + c(t) y + a(t), y = \text{sqrt}(\text{diff}(d(t), t)) e(t) y + b(t), u[ \right] \right. \right. \right. \right. \end{aligned}$$

$$= \frac{e(t) u[ ]}{\text{sqrt}(\text{diff}(d(t), t))} - \frac{y}{e(t)^2} \text{diff} \left( \frac{e(t)^3}{\text{sqrt}(\text{diff}(d(t), t))}, t \right) + \frac{\text{diff}(b(t), t)}{\text{diff}(d(t), t)}$$

$$\begin{aligned}
& - \frac{2 c(t)}{e(t) \sqrt{\text{diff}(d(t), t)}}, v[ ] = \frac{e(t)^2}{\text{diff}(d(t), t)} v[ ] \\
& + \frac{(c(t) + 2 e(t) \text{diff}(e(t), t) y)}{\text{diff}(d(t), t)} u[ ] \\
& + \frac{(e(t) \text{diff}(e(t), t, t) - 3 \text{diff}(e(t), t)^2)}{\text{diff}(d(t), t)} y^2 + \frac{e(t)^4}{\text{diff}(d(t), t)} \text{diff}\left(\frac{c(t)}{e(t)^4}, t\right) y \\
& + \frac{2 e(t) \text{diff}(e(t), t)}{\text{diff}(d(t), t)} x + \frac{(e(t)^2 \text{diff}(a(t), t) - c(t)^2)}{\text{diff}(d(t), t) e(t)^2} \left] \right) \left) \right) \\
\phi := & \left[ t = d(t), x = e(t)^2 x + e(t) \dot{e}(t) y^2 + c(t) y + a(t), y = \sqrt{d(t)} e(t) y + b(t), \right. \quad (8.3.7)
\end{aligned}$$

$$\begin{aligned}
u[ ] = & \frac{1}{2 \dot{d}(t)^{3/2} e(t)} \left( 2 e(t)^2 \dot{d}(t) u[ ] + e(t)^2 \ddot{d}(t) y - 6 e(t) \dot{d}(t) \dot{e}(t) y \right. \\
& + 2 e(t) \dot{b}(t) \sqrt{d(t)} - 4 \dot{d}(t) c(t) \left. \right), v[ ] = \frac{1}{e(t)^2 \dot{d}(t)} \left( \ddot{e}(t) e(t)^3 y^2 \right. \\
& - 3 e(t)^2 \dot{e}(t)^2 y^2 + 2 e(t) \left( (y u[ ] + x) e(t)^2 - 2 c(t) y \right) \dot{e}(t) + e(t)^4 v[ ] + \\
& \left. \dot{c}(t) e(t)^2 y + e(t)^2 c(t) u[ ] + e(t)^2 \dot{a}(t) - c(t)^2 \right),
\end{aligned}$$

$$\begin{aligned}
> \text{collect}(\text{solve}(\text{Pullback}(\phi, \text{eval}(u[ ] - x - \exp(y), \text{sol1})), u[ ]), [x, y]) \\
\sqrt{\frac{d}{dt} d(t)} e(t) x + \left( \frac{d}{dt} e(t) \right) \sqrt{\frac{d}{dt} d(t)} y^2 - \frac{1}{2} \frac{1}{e(t)^2 \left( \frac{d}{dt} d(t) \right)} \left( \left( \right. \quad (8.3.8) \\
- 2 c(t) \left( \frac{d}{dt} d(t) \right)^{3/2} e(t) + \left( \frac{d^2}{dt^2} d(t) \right) e(t)^2 \\
- 6 \left( \frac{d}{dt} e(t) \right) e(t) \left( \frac{d}{dt} d(t) \right) y \left. \right) - \frac{1}{2} \frac{1}{e(t)^2 \left( \frac{d}{dt} d(t) \right)} \left( \right. \\
- 2 a(t) \left( \frac{d}{dt} d(t) \right)^{3/2} e(t) - 2 e^{\sqrt{\frac{d}{dt} d(t)} e(t) y + b(t)} \left( \frac{d}{dt} d(t) \right)^{3/2} e(t) \\
\left. + 2 e(t) \left( \frac{d}{dt} b(t) \right) \sqrt{\frac{d}{dt} d(t)} - 4 \left( \frac{d}{dt} d(t) \right) c(t) \right)
\end{aligned}$$

$$\begin{aligned}
> \text{pdetest} \left( \left\{ u(t, x, y) = x + e^y, v(t, x, y) = -F4(t) x + -F2(t, y) \right\}, \left[ \frac{\partial^4}{\partial y^4} v(t, x, y) \right. \right. \\
= 2 \left( \frac{\partial^2}{\partial y^2} u(t, x, y) \right) \left( \frac{\partial}{\partial x} u(t, x, y) \right) \left( \frac{\partial}{\partial x} v(t, x, y) \right) + 2 \left( \frac{\partial}{\partial x} u(t, x, \right. \\
y) \left. \right) \left( \frac{\partial}{\partial x} v(t, x, y) \right) \left( \frac{\partial^2}{\partial y \partial x} v(t, x, y) \right) - \left( \frac{\partial^3}{\partial y^3} v(t, x, y) \right) \left( \frac{\partial}{\partial x} u(t, x, y) \right) \\
+ 5 \left( \frac{\partial^2}{\partial y^2} u(t, x, y) \right) \left( \frac{\partial^2}{\partial y \partial x} v(t, x, y) \right) + 2 \left( \frac{\partial^2}{\partial y \partial x} v(t, x, y) \right)^2, \frac{\partial^3}{\partial y^2 \partial x} v(t, x, \\
y) = 0, \frac{\partial^3}{\partial y^3} u(t, x, y) = \left( \frac{\partial}{\partial x} u(t, x, y) \right) \left( \frac{\partial^2}{\partial y^2} u(t, x, y) + \frac{\partial^2}{\partial y \partial x} v(t, x, y) \right),
\end{aligned}$$

$$\left[ \frac{\partial^2}{\partial x^2} u(t, x, y) = 0, \frac{\partial^2}{\partial x^2} v(t, x, y) = 0, \frac{\partial^2}{\partial y \partial x} u(t, x, y) = 0 \right] \\ \left[ \frac{\partial^4}{\partial y^4} \_F2(t, y) - 2 \_F4(t) e^y + \frac{\partial^3}{\partial y^3} \_F2(t, y), 0, 0, 0, 0, 0 \right] \quad (8.3.9)$$

$$> \text{pdsolve} \left( \frac{\partial^4}{\partial y^4} \_F2(t, y) - 2 \_F4(t) e^y + \frac{\partial^3}{\partial y^3} \_F2(t, y) \right) \\ \_F2(t, y) = \_F4(t) e^y - e^{-y} \_F5(t) + \frac{1}{2} \_F6(t) y^2 + \_F7(t) y + \_F8(t) \quad (8.3.10)$$

$$> \text{pdetest} \left( \left\{ u(t, x, y) = 0, v(t, x, y) = \frac{1}{12} y^4 + x y + h(t) \right\}, \text{sys} \right) \\ \{0\} \quad (8.3.11)$$

#### 4.4 K's and I2 are constant

Let us also consider the case, when all invariants I and K are constants

$$> I1 := \frac{u_{2,3} + v_{2,2}}{u_2^2} : I2 := \frac{u_2^2 u_{2,3} + u_2 u_{2,2} v_2 + u_{2,2} u_{3,3} - u_{2,3}^2}{u_2^4} : I3 \\ := \frac{u_2^2 v_{2,2} - u_2 u_{2,2} v_2 + u_{2,2} v_{2,3} - u_{2,3} v_{2,2}}{u_2^4} : K1 := \text{expand} \left( \frac{u_2 u_{2,2,2}}{u_{2,2}^2} - 3 \right) : \\ K2 := - \frac{u_{2,2} u_{2,2,3} - u_{2,3} u_{2,2,2}}{u_2 u_{2,2}^2} : \\ K3 := K2 \cdot \left( 1 - \frac{2 u[2,3]}{u[2]^2} \right) + 2 \cdot \frac{u[2,2] u[3,3] - u[2,3]^2}{u[2]^4} \\ + 2 \frac{(u[2,3] u[2,2,3] - u[2,2] u[2,3,3])}{u[2]^3 u[2,2]} : \\ K4 := - \text{simplify} \left( \frac{1}{u_2^5 u_{2,2}^2} (u_{2,2}^3 u_{2,3,3} - u_{2,2}^2 u_{2,3} u_{2,2,3} + u_{2,2}^2 u_{2,2,3}^2 - 2 u_{2,2}^2 u_{2,2} u_{2,3} u_{2,2,3} + u_{2,2}^2 u_{2,3}^2 u_{2,2,2} + u_{2,2}^3 u_{2,2,2} v_{2,3} - u_{2,2}^2 u_{2,2}^2 u_{2,3}^2 - u_{2,2}^2 u_{2,2} u_{2,3} v_{2,2} \right. \\ + u_{2,3}^3 u_{2,2} u_{2,3} + u_{2,2}^4 u_{2,3} v_3 - u_{2,2}^3 u_{2,3} v_2 + u_{2,2}^3 u_{2,2,3} v_{2,3} - u_{2,2}^2 u_{2,3} u_{2,2,2} v_{2,3} + u_{2,2}^3 u_{2,2,3}^2 + u_{2,2}^3 u_{2,3,3} - u_{2,2}^2 u_{2,3} u_{2,2,2} - 5 u_{2,2}^2 u_{2,3} u_{2,3,3} + 6 u_{2,2}^2 u_{2,3}^2 u_{2,2,3} \\ \left. - 2 u_{2,3}^3 u_{2,2,2} \right) \right) : \\ > D1 := \text{proc} (funct) \\ \text{simplify} \left( \frac{u_2}{u_{2,2}} \text{TotalDiff} (funct, x) \right); \\ \text{end proc}; \\ D2 := \text{proc} (funct) \\ \text{simplify} \left( \frac{u_{2,3}}{u_2 u_{2,2}} \text{TotalDiff} (funct, x) - \frac{1}{u_2} \text{TotalDiff} (funct, y) \right); \\ \text{end proc}; \\ D3 := \text{proc} (funct)$$

$$\text{simplify}\left(\frac{1}{u[2]^3} \left( u[2, 2] \text{TotalDiff}(\text{funct}, t) + (v[1] u_{2, 2} + v_2 u_2 + u[3, 3]) \text{TotalDiff}(\text{funct}, x) + (u[1] u_{2, 2} + u_2^2 - 2 u_{2, 3}) \text{TotalDiff}(\text{funct}, y) \right)\right);$$

**end proc;**

We compute syzygies. The computation is a little time-consuming, so if you just want to see the syzygies they are made available in a subsection.

```

> A := Pullback(T2, I1) : B := Pullback(T2, I2) : C := Pullback(T2, I3) :
> for i from 1 to 3 do
  A || i := Pullback(T3, D || i(A)); B || i := Pullback(T3, D || i(B)); C || i := Pullback(T3,
    D || i(C));
od:
> for j from 1 to 3 do
  for k from 1 to 3 do
    A || k || j := Pullback(T4, D || j(D || k(A))); B || k || j := Pullback(T4, D || j(D || k(B)));
    C || k || j := Pullback(T4, D || j(D || k(C)));
  od:od:
>
> for i from 1 to 4 do
  KK || i := Pullback(T3, K || i);
od:
> for j from 1 to 3 do
  for i from 1 to 4 do
    KK || i || j := Pullback(T4, D || j(K || i));
  od:od:
> fourjets := {seq(seq(seq(seq(op([u[i1, i2, i3, i4], v[i1, i2, i3, i4]]), i4 = i3 ..3), i3 = i2
  ..3), i2 = i1 ..3), i1 = 1 ..3) : nops(%)
  30 (8.4.1)
> threejets := {seq(seq(seq(op([u[i1, i2, i3], v[i1, i2, i3]]), i3 = i2 ..3), i2 = i1 ..3), i1
  = 1 ..3) : nops(%)
  20 (8.4.2)
> twojets := {seq(seq(op([u[i1, i2], v[i1, i2]]), i2 = i1 ..3), i1 = 1 ..3) : nops(%)
  12 (8.4.3)
> eq1K := eliminate( {seq(seq(A || k || j, k = 1 ..3), j = 1 ..3), seq(seq(B || k || j, k = 1 ..3), j
  = 1 ..3), seq(seq(C || k || j, k = 1 ..3), j = 1 ..3), seq(seq(KK || i || j, j = 1 ..3), i = 1
  ..4) }, fourjets)[2] :
> nops(eq1K)
  26 (8.4.4)
>
> tmpp := { } :for j to nops(eq1K) do for i to nops(fourjets) do tmpp := tmpp
  union {diff(eq1K[j], fourjets[i])} :od:od: tmpp
  {0} (8.4.5)
> eq2K := eliminate( {op(simplify(eq1K)), seq(A || i, i = 1 ..3), seq(B || i, i = 1 ..3), seq(C
  || i, i = 1 ..3), seq(K || i - k || i, i = 1 ..4) }, threejets)[2] :
> smpleq2 := simplify(eq2K) : nops(eq2K)
  21 (8.4.6)
> tmpp := { } :for j to nops(eq2K) do for i to nops(threejets) do tmpp := tmpp
  union {diff(eq2K[j], threejets[i])} :od:od: tmpp
  {0} (8.4.7)
> eq3K := eliminate(eq2K union {A - a, B - b, C - c}, twojets)[2] : nops(eq3K)
  (8.4.8)

```

> eq3K :

> tmpp := { } :for j to nops(eq3K) do for i to nops(twojets) do tmpp := tmpp  
     union {diff(eq3K[j], twojets[i])} :od:od: tmpp  
     {0}

(8.4.9)

> sysconst := [solve(eq3K)]

sysconst := [ {a=0, b=0, c=0, k1=k1, k2=0}, {a=0, b=b, c=-b, k1=0, k2  
     =0}, {a=- $\frac{3}{25}$ , b= $\frac{21}{100}$ , c=- $\frac{147}{500}$ , k1=1, k2=0} ]

(8.4.10)

> solve( $-\frac{3}{25} = \frac{k3}{2} - \frac{21}{100} \cdot 1, k3$ ); solve( $-\frac{147}{500} = \frac{\frac{3 \cdot 9}{50} + 2 k4}{4} + \frac{21}{100} \cdot (0 - 1$   
      $- 1), k4$ )

$$\frac{9}{50}$$

$$-\frac{9}{500}$$

(8.4.11)

> eq := FromJet( numer( eval( {A-a, B-b, C-c, K1-k1, K2-k2, K3-k3, K4  
     -k4}, {a=- $\frac{3}{25}$ , b= $\frac{21}{100}$ , c=- $\frac{147}{500}$ , k1=1, k2=0, k3= $\frac{9}{50}$ , k4=- $\frac{9}{500}$  } ) )  
     , {u(t, x, y), v(t, x, y)} ) :

> sol := pdsolve( FromJet( {I1=- $\frac{3}{25}$ , I2= $\frac{21}{100}$ , I3=- $\frac{147}{500}$ }, {u(t, x, y), v(t, x, y)} ) )

sol := { u(t, x, y) =  $\frac{10 x}{10 \_F3(t) - 3 y} + \_F2(t, y)$ , v(t, x, y) = - $\frac{21 x^2}{(10 \_F3(t) - 3 y)^2}$   
     +  $\_F4(t, y) x + \_F5(t, y)$  }

(8.4.12)

> phi := simplify( ( Transformation( MM, MM, [ t=d(t), x=e(t)<sup>2</sup> x + e(t) diff(e(t),

t) y<sup>2</sup> + c(t) y + a(t), y=sqrt(diff(d(t), t)) e(t) y + b(t), u[ ]

$$= \frac{e(t) u[ ]}{\sqrt{\text{diff}(d(t), t)}} - \frac{y}{e(t)^2} \text{diff}\left(\frac{e(t)^3}{\sqrt{\text{diff}(d(t), t)}}, t\right) + \frac{\text{diff}(b(t), t)}{\text{diff}(d(t), t)}$$

$$- \frac{2 c(t)}{e(t) \sqrt{\text{diff}(d(t), t)}}, v[ ] = \frac{e(t)^2}{\text{diff}(d(t), t)} v[ ]$$

$$+ \frac{(c(t) + 2 e(t) \text{diff}(e(t), t) y)}{\text{diff}(d(t), t)} u[ ]$$

$$+ \frac{(e(t) \text{diff}(e(t), t, t) - 3 \text{diff}(e(t), t)^2)}{\text{diff}(d(t), t)} y^2 + \frac{e(t)^4}{\text{diff}(d(t), t)} \text{diff}\left(\frac{c(t)}{e(t)^4}, t\right) y$$

$$+ \frac{2 e(t) \text{diff}(e(t), t)}{\text{diff}(d(t), t)} x + \frac{(e(t)^2 \text{diff}(a(t), t) - c(t)^2)}{\text{diff}(d(t), t) e(t)^2} \Bigg] \Bigg)$$



$$\begin{aligned} & \text{eval(sol, pdsolve(eval(eq2, f1(t, y) = 0)) \text{ union } \{f1(t, y) = 0\}) \\ & \left\{ u(t, x, y) = -\frac{10}{3} \frac{x}{y}, v(t, x, y) = -\frac{7}{3} \frac{x^2}{y^2} + \_F1(t) y^{7/3} + \_F2(t) y^2 \right\} \end{aligned} \quad (8.4.19)$$

The following symmetries preserve this form.

$$\begin{aligned} & \text{collect} \left( \text{simplify} \left( \text{eval} \left( \text{collect} \left( \text{solve} \left( \text{Pullback} \left( \text{phi}, \left[ u[] - \left( -\frac{10}{3} \frac{x}{y} \right), v[] - \left( -\frac{7}{3} \frac{x^2}{y^2} + f(t) y^{7/3} + h(t) y^2 \right) \right] \right), \{u[], v[]\} \right), [x, y] \right), \left\{ b(t) = 0, c(t) = 0, a(t) \right. \right. \right. \\ & \quad \left. \left. = 0, e(t) = \frac{-CI}{\left( \frac{d}{dt} d(t) \right)^{3/2}} \right\} \right), [x, y] \right) \\ & \left\{ u[] = -\frac{10}{3} \frac{x}{y}, v[] = -\frac{7}{3} \frac{x^2}{y^2} \right. \\ & \quad + \frac{1}{12} \frac{1}{\left( \frac{d}{dt} d(t) \right)^2} \left( \left( 12 \left( \frac{-CI y}{\frac{d}{dt} d(t)} \right)^{1/3} \left( \frac{d}{dt} d(t) \right)^4 f(d(t)) \right. \right. \\ & \quad \left. \left. + 12 h(d(t)) \left( \frac{d}{dt} d(t) \right)^4 + 18 \left( \frac{d^3}{dt^3} d(t) \right) \left( \frac{d}{dt} d(t) \right) - 27 \left( \frac{d^2}{dt^2} d(t) \right)^2 \right) \right. \\ & \quad \left. y^2 \right\} \end{aligned} \quad (8.4.20)$$

The general solution is:

$$\begin{aligned} & \text{eval(sol, pdsolve(eq2))} \\ & \left\{ u(t, x, y) = -\frac{10}{3} \frac{x}{y} + \frac{5}{7} \frac{\_F3(t)}{y} + \frac{5}{2} y^{2/3} \_F1(t) + \_F2(t) - \_F4(t) y, v(t, x, \right. \quad (8.4.21) \\ & \quad y) = -\frac{7}{3} \frac{x^2}{y^2} + \left( \frac{\_F1(t)}{y^{1/3}} + \frac{\_F2(t)}{y} + \frac{\_F3(t)}{y^2} \right) x + y^{7/3} \_F6(t) + \_F5(t) y^2 \\ & \quad + \frac{1}{14} \left( \int \frac{1}{y^{17/3}} \left( 147 \_F1(t)^2 y^{11/3} - 70 \_F1(t) \_F4(t) y^4 \right. \right. \\ & \quad \left. \left. - 42 \_F2(t) \_F4(t) y^{10/3} + 105 y^3 \_F1(t) \_F2(t) + 42 \left( \frac{d}{dt} \_F2(t) \right) y^{10/3} \right) \right. \end{aligned}$$



$$\begin{aligned}
& + 42 \left( \frac{d}{dt} \_F1(t) \right) y^4 - 56 \_F3(t) \_F1(t) y^2 - 90 \_F2(t) \_F3(t) y^{4/3} \\
& + 42 \left( \frac{d}{dt} \_F3(t) \right) y^{7/3} - 78 \_F3(t)^2 y^{1/3} \Big) dy \Big) y^{7/3} - \frac{1}{14} \left( \right. \\
& \int \frac{1}{y^{16/3}} \left( 147 \_F1(t)^2 y^{11/3} - 70 \_F1(t) \_F4(t) y^4 - 42 \_F2(t) \_F4(t) y^{10/3} \right. \\
& + 105 y^3 \_F1(t) \_F2(t) + 42 \left( \frac{d}{dt} \_F2(t) \right) y^{10/3} + 42 \left( \frac{d}{dt} \_F1(t) \right) y^4 \\
& - 56 \_F3(t) \_F1(t) y^2 - 90 \_F2(t) \_F3(t) y^{4/3} + 42 \left( \frac{d}{dt} \_F3(t) \right) y^{7/3} \\
& \left. \left. - 78 \_F3(t)^2 y^{1/3} \right) dy \right) y^2 \Big\}
\end{aligned}$$

>

$$\begin{aligned}
& \text{eval} \left( \text{collect} \left( \text{simplify} \left( \text{eval} \left( \text{solve}(\text{Pullback}(\text{phi}, \text{eval}([u[] - u(t, x, y), v[] - v(t, x, \right. \right. \right. \right. \\
& y)], \text{eval}(\text{sol}, \text{pdsolve}(\text{eq2}))) \right), \{u[], v[]\} \right), \left\{ e(t) = 1, d(t) = t, b(t) = 0, c(t) \right. \\
& \left. = \frac{3}{4} \_F2(t), a(t) = \frac{3}{14} \_F3(t) \right\} \right), \text{symbolic} \Big), [x, y] \Big), \{ \} \Big)
\end{aligned}$$

$$\left\{ u[] = -\frac{10}{3} \frac{x}{y} - \_F4(t) y + \frac{5}{2} y^{2/3} \_F1(t), v[] = -\frac{7}{3} \frac{x^2}{y^2} + \frac{\_F1(t) x}{y^{1/3}} + \left( \frac{1}{14} \right. \right. \quad (8.4.22)$$

$$\begin{aligned}
& \int \frac{1}{y^{17/3}} \left( 147 \_F1(t)^2 y^{11/3} - 70 \_F1(t) \_F4(t) y^4 - 42 \_F2(t) \_F4(t) y^{10/3} \right. \\
& + 105 y^3 \_F1(t) \_F2(t) + 42 \left( \frac{d}{dt} \_F2(t) \right) y^{10/3} + 42 \left( \frac{d}{dt} \_F1(t) \right) y^4 \\
& - 56 \_F3(t) \_F1(t) y^2 - 90 \_F2(t) \_F3(t) y^{4/3} + 42 \left( \frac{d}{dt} \_F3(t) \right) y^{7/3} \\
& \left. - 78 \_F3(t)^2 y^{1/3} \right) dy + \_F5(t) \Big) y^{7/3} + \left( -\frac{1}{14} \int \frac{1}{y^{16/3}} \left( 147 \_F1(t)^2 y^{11/3} \right. \right. \\
& - 70 \_F1(t) \_F4(t) y^4 - 42 \_F2(t) \_F4(t) y^{10/3} + 105 y^3 \_F1(t) \_F2(t) \\
& + 42 \left( \frac{d}{dt} \_F2(t) \right) y^{10/3} + 42 \left( \frac{d}{dt} \_F1(t) \right) y^4 - 56 \_F3(t) \_F1(t) y^2 \\
& - 90 \_F2(t) \_F3(t) y^{4/3} + 42 \left( \frac{d}{dt} \_F3(t) \right) y^{7/3} - 78 \_F3(t)^2 y^{1/3} \Big) dy \\
& \left. + \_F6(t) \right) y^2 + \left( \frac{3}{4} \_F2(t) \_F4(t) - \frac{3}{4} \frac{d}{dt} \_F2(t) \right) y
\end{aligned}$$



$$\begin{aligned}
& + \frac{FI(t) x}{y^{1/3}} + \frac{21}{4} \left[ FI(t)^2 y^{4/3} + F2(t) y^2 + F3(t) y^{5/3} + F4(t) y^{7/3} \right] \Bigg) \Bigg], \\
& \left\{ u \left[ \begin{array}{c} ] \\ ] \end{array} \right], v \left[ \begin{array}{c} ] \\ ] \end{array} \right] \right\}, \left\{ b(t) = 0, c(t) = 0, a(t) = 0 \right\}, symbolic \Bigg), [x, y] \Bigg), \left\{ \begin{array}{c} \\ \end{array} \right\} \Bigg) \\
& \left\{ u \left[ \begin{array}{c} ] \\ ] \end{array} \right] = -\frac{10}{3} \frac{x}{y} + \frac{2}{15} \frac{1}{\left( \frac{d}{dt} d(t) \right)^{7/6} e(t) FI(d(t))} \left( \left( e(t) \left( -F3(d(t)) \right. \right. \right. \right. \quad (8.4.25) \\
& \left. \left. \left. \left. -\frac{9}{2} \frac{d}{dt} FI(t) \right|_{t=d(t)} \right) \left( \frac{d}{dt} d(t) \right)^{13/6} + \frac{75}{4} FI(d(t)) \left( \right. \right. \right. \\
& \left. \left. \left. -\frac{2}{15} \left( \frac{d}{dt} d(t) \right)^{7/6} \left( \frac{d}{dt} e(t) \right) - \frac{1}{5} e(t) \left( \frac{d^2}{dt^2} d(t) \right) \left( \frac{d}{dt} d(t) \right)^{1/6} \right) \right) y \right) \\
& + \frac{5}{2} \frac{\left( \frac{d}{dt} d(t) \right)^{5/6} FI(d(t)) y^{2/3}}{e(t)^{1/3}}, v \left[ \begin{array}{c} ] \\ ] \end{array} \right] = -\frac{7}{3} \frac{x^2}{y^2} \\
& + \frac{\left( \frac{d}{dt} d(t) \right)^{5/6} FI(d(t)) x}{e(t)^{1/3} y^{1/3}} + e(t)^{1/3} F4(d(t)) \left( \frac{d}{dt} d(t) \right)^{13/6} y^{7/3} \\
& + \frac{4}{3} \frac{1}{e(t)^{7/3} \left( \frac{d}{dt} d(t) \right)^{7/6} FI(d(t))} \left( \left( -FI(d(t)) \left( \right. \right. \right. \right. \\
& \left. \left. \left. -\frac{3}{4} \left( \frac{d^2}{dt^2} e(t) \right) e(t)^{4/3} + e(t)^{1/3} \left( \frac{d}{dt} e(t) \right)^2 \right) \left( \frac{d}{dt} d(t) \right)^{7/6} \right. \right. \\
& \left. \left. -\frac{1}{5} \left( \frac{d}{dt} e(t) \right) \left( -F3(d(t)) - \frac{9}{2} \frac{d}{dt} FI(t) \right| \right. \right. \right.
\end{aligned}$$

$$\begin{aligned}
& \left. e(t)^{4/3} \left( \frac{d}{dt} d(t) \right)^{13/6} \right|_{t=d(t)} \\
& + \frac{3}{4} \_F1(d(t)) \left( \left( \frac{d}{dt} d(t) \right)^{19/6} \_F2(d(t)) e(t)^{7/3} \right. \\
& + \left. \left( \frac{d}{dt} d(t) \right)^{1/6} e(t)^{4/3} \left( \frac{d^2}{dt^2} d(t) \right) \left( \frac{d}{dt} e(t) \right) \right) y^2 \\
& + \frac{1}{e(t)^{4/3}} \left( \left( \frac{d}{dt} d(t) \right)^{5/6} \left( \left( \frac{d}{dt} d(t) \right) \_F3(d(t)) e(t) \right. \right. \\
& \left. \left. - 4 \_F1(d(t)) \left( \frac{d}{dt} e(t) \right) \right) y^{5/3} \right) + \frac{21}{4} \frac{\_F1(d(t))^2 \left( \frac{d}{dt} d(t) \right)^{5/3} y^{4/3}}{e(t)^{2/3}} \Bigg\}
\end{aligned}$$

$$\begin{aligned}
& \text{pdsolve} \left( \text{map} \left( \text{coeffs}, \text{numer} \left( \text{pdetest} \left( \left\{ u(t, x, y) = -\frac{10}{3} \frac{x}{y} + \frac{5}{2} y^{2/3} f2(t), v(t, x, y) = \right. \right. \right. \right. \right. \\
& \left. \left. \left. - \frac{7}{3} \frac{x^2}{y^2} + f3(t, y) x + f4(t, y) \right\}, \text{FromJet}(\{E1, E2\}, \{u(t, x, y), v(t, x, y)\}) \right) \right), \\
& \left. x \right) \Bigg) \\
& \left\{ f2(t) = \_F1(t), f3(t, y) = \frac{\_F1(t)}{y^{1/3}}, f4(t, y) = \_F3(t) y^{7/3} + \_F2(t) y^2 \right. \\
& \left. + \frac{3}{4} y^{4/3} \left( 6 \left( \frac{d}{dt} \_F1(t) \right) y^{1/3} + 7 \_F1(t)^2 \right) \right\} \tag{8.4.26}
\end{aligned}$$

$$\begin{aligned}
& \text{collect} \left( \text{simplify} \left( \text{eval} \left( \text{solve} \left( \text{Pullback} \left( \text{phi}, \left[ u[ ] - \left( -\frac{10}{3} \frac{x}{y} + \frac{5}{2} y^{2/3} \_F1(t) \right), \right. \right. \right. \right. \right. \right. \right. \right. \right. \\
& \left. \left. \left. v[ ] - \left( -\frac{7}{3} \frac{x^2}{y^2} + \frac{\_F1(t) x}{y^{1/3}} + \_F3(t) y^{7/3} + \_F2(t) y^2 \right. \right. \right. \right. \right. \\
& \left. \left. \left. + \frac{3}{4} y^{4/3} \left( 6 \left( \frac{d}{dt} \_F1(t) \right) y^{1/3} + 7 \_F1(t)^2 \right) \right) \right) \right), \{u[ ], v[ ]\} \right), \left\{ a(t) = 0, b(t) \right. \\
& \left. = 0, c(t) = 0, e(t) = \left( \frac{5}{2} \right)^3 \left( \frac{d}{dt} d(t) \right)^{5/2} \_F1(d(t))^3 \right\}, \text{symbolic} \Bigg), [x, y] \Bigg) [1] \\
& u[ ] = -\frac{10}{3} \frac{x}{y} + \frac{1}{3} \frac{(-3 D(d)(t)^2 D(\_F1)(d(t)) - 4 \_F1(d(t)) D^{(2)}(d)(t)) y}{D(d)(t) \_F1(d(t))} + y^{2/3} \tag{8.4.27}
\end{aligned}$$
